# Supplementary material for: BindAdapt: Joint Camera-Computation Scheduling for Persistent Target Identity in PTZ Tracking
Source: arXiv:2611.38995 source file (2026-11-28)
Supplement: Supplementary file 1 [file supp_numbers.tex]

\providecommand{\BAval}[1]{\ifcsname BAval@#1\endcsname\csname BAval@#1\endcsname\else\PackageError{BindAdapt}{Unknown numeric ledger key #1}{}\fi}
\expandafter\def\csname BAval@t01.r01.sid\endcsname{44.0}
\expandafter\def\csname BAval@t01.r01.wrong\endcsname{19.8}
\expandafter\def\csname BAval@t01.r01.recovery\endcsname{42.0}
\expandafter\def\csname BAval@t01.r01.t5\endcsname{3.8}
\expandafter\def\csname BAval@t01.r02.sid\endcsname{58.2}
\expandafter\def\csname BAval@t01.r02.wrong\endcsname{15.3}
\expandafter\def\csname BAval@t01.r02.recovery\endcsname{56.0}
\expandafter\def\csname BAval@t01.r02.t5\endcsname{3.2}
\expandafter\def\csname BAval@t01.r03.sid\endcsname{55.6}
\expandafter\def\csname BAval@t01.r03.wrong\endcsname{17.0}
\expandafter\def\csname BAval@t01.r03.recovery\endcsname{54.0}
\expandafter\def\csname BAval@t01.r03.t5\endcsname{3.3}
\expandafter\def\csname BAval@t01.r04.sid\endcsname{64.5}
\expandafter\def\csname BAval@t01.r04.wrong\endcsname{12.2}
\expandafter\def\csname BAval@t01.r04.recovery\endcsname{64.0}
\expandafter\def\csname BAval@t01.r04.t5\endcsname{2.8}
\expandafter\def\csname BAval@t01.r05.sid\endcsname{65.8}
\expandafter\def\csname BAval@t01.r05.wrong\endcsname{11.8}
\expandafter\def\csname BAval@t01.r05.recovery\endcsname{65.0}
\expandafter\def\csname BAval@t01.r05.t5\endcsname{2.7}
\expandafter\def\csname BAval@t01.r06.sid\endcsname{68.7}
\expandafter\def\csname BAval@t01.r06.wrong\endcsname{10.1}
\expandafter\def\csname BAval@t01.r06.recovery\endcsname{70.0}
\expandafter\def\csname BAval@t01.r06.t5\endcsname{2.5}
\expandafter\def\csname BAval@t01.r07.sid\endcsname{70.3}
\expandafter\def\csname BAval@t01.r07.wrong\endcsname{8.8}
\expandafter\def\csname BAval@t01.r07.recovery\endcsname{72.0}
\expandafter\def\csname BAval@t01.r07.t5\endcsname{2.4}
\expandafter\def\csname BAval@t01.r08.sid\endcsname{82.3}
\expandafter\def\csname BAval@t01.r08.wrong\endcsname{4.4}
\expandafter\def\csname BAval@t01.r08.recovery\endcsname{86.2}
\expandafter\def\csname BAval@t01.r08.t5\endcsname{1.4}
\expandafter\def\csname BAval@t01.r09.sid\endcsname{87.9}
\expandafter\def\csname BAval@t01.r09.wrong\endcsname{1.6}
\expandafter\def\csname BAval@t01.r09.recovery\endcsname{92.0}
\expandafter\def\csname BAval@t01.r09.t5\endcsname{1.2}
\expandafter\def\csname BAval@t02.r01.short\endcsname{78.0}
\expandafter\def\csname BAval@t02.r01.similar\endcsname{67.0}
\expandafter\def\csname BAval@t02.r01.long\endcsname{53.0}
\expandafter\def\csname BAval@t02.r02.short\endcsname{79.0}
\expandafter\def\csname BAval@t02.r02.similar\endcsname{68.0}
\expandafter\def\csname BAval@t02.r02.long\endcsname{54.8}
\expandafter\def\csname BAval@t02.r03.short\endcsname{80.0}
\expandafter\def\csname BAval@t02.r03.similar\endcsname{72.0}
\expandafter\def\csname BAval@t02.r03.long\endcsname{57.6}
\expandafter\def\csname BAval@t02.r04.short\endcsname{82.0}
\expandafter\def\csname BAval@t02.r04.similar\endcsname{74.0}
\expandafter\def\csname BAval@t02.r04.long\endcsname{58.3}
\expandafter\def\csname BAval@t02.r05.short\endcsname{90.2}
\expandafter\def\csname BAval@t02.r05.similar\endcsname{85.4}
\expandafter\def\csname BAval@t02.r05.long\endcsname{73.9}
\expandafter\def\csname BAval@t02.r06.short\endcsname{94.0}
\expandafter\def\csname BAval@t02.r06.similar\endcsname{90.0}
\expandafter\def\csname BAval@t02.r06.long\endcsname{82.0}
\expandafter\def\csname BAval@t03.r01.sid\endcsname{65.9}
\expandafter\def\csname BAval@t03.r01.wrong\endcsname{11.9}
\expandafter\def\csname BAval@t03.r02.sid\endcsname{70.3}
\expandafter\def\csname BAval@t03.r02.wrong\endcsname{8.8}
\expandafter\def\csname BAval@t03.r03.sid\endcsname{77.6}
\expandafter\def\csname BAval@t03.r03.wrong\endcsname{6.3}
\expandafter\def\csname BAval@t03.r04.sid\endcsname{82.3}
\expandafter\def\csname BAval@t03.r04.wrong\endcsname{4.4}
\expandafter\def\csname BAval@t04.r01.sid\endcsname{82.3}
\expandafter\def\csname BAval@t04.r01.wrong\endcsname{4.4}
\expandafter\def\csname BAval@t04.r01.t5\endcsname{1.4}
\expandafter\def\csname BAval@t04.r02.sid\endcsname{77.9}
\expandafter\def\csname BAval@t04.r02.wrong\endcsname{7.1}
\expandafter\def\csname BAval@t04.r02.t5\endcsname{1.9}
\expandafter\def\csname BAval@t04.r03.sid\endcsname{76.0}
\expandafter\def\csname BAval@t04.r03.wrong\endcsname{9.0}
\expandafter\def\csname BAval@t04.r03.t5\endcsname{2.0}
\expandafter\def\csname BAval@t04.r04.sid\endcsname{78.0}
\expandafter\def\csname BAval@t04.r04.wrong\endcsname{7.7}
\expandafter\def\csname BAval@t04.r04.t5\endcsname{1.8}
\expandafter\def\csname BAval@t04.r05.sid\endcsname{79.3}
\expandafter\def\csname BAval@t04.r05.wrong\endcsname{6.8}
\expandafter\def\csname BAval@t04.r05.t5\endcsname{1.6}
\expandafter\def\csname BAval@t04.r06.sid\endcsname{73.7}
\expandafter\def\csname BAval@t04.r06.wrong\endcsname{8.8}
\expandafter\def\csname BAval@t04.r06.t5\endcsname{2.2}
\expandafter\def\csname BAval@t04.r07.sid\endcsname{77.6}
\expandafter\def\csname BAval@t04.r07.wrong\endcsname{6.3}
\expandafter\def\csname BAval@t04.r07.t5\endcsname{1.7}
\expandafter\def\csname BAval@t04.r08.sid\endcsname{80.5}
\expandafter\def\csname BAval@t04.r08.wrong\endcsname{5.8}
\expandafter\def\csname BAval@t04.r08.t5\endcsname{1.5}
\expandafter\def\csname BAval@t05.r01.separable\endcsname{78.0}
\expandafter\def\csname BAval@t05.r01.temporal.q\endcsname{80.1}
\expandafter\def\csname BAval@t05.r01.bindadapt\endcsname{86.1}
\expandafter\def\csname BAval@t05.r01.oracle\endcsname{91.7}
\expandafter\def\csname BAval@t05.r02.separable\endcsname{75.6}
\expandafter\def\csname BAval@t05.r02.temporal.q\endcsname{77.2}
\expandafter\def\csname BAval@t05.r02.bindadapt\endcsname{85.3}
\expandafter\def\csname BAval@t05.r02.oracle\endcsname{90.9}
\expandafter\def\csname BAval@t05.r03.separable\endcsname{71.1}
\expandafter\def\csname BAval@t05.r03.temporal.q\endcsname{73.2}
\expandafter\def\csname BAval@t05.r03.bindadapt\endcsname{83.8}
\expandafter\def\csname BAval@t05.r03.oracle\endcsname{90.1}
\expandafter\def\csname BAval@t05.r04.separable\endcsname{65.9}
\expandafter\def\csname BAval@t05.r04.temporal.q\endcsname{68.7}
\expandafter\def\csname BAval@t05.r04.bindadapt\endcsname{82.3}
\expandafter\def\csname BAval@t05.r04.oracle\endcsname{87.9}
\expandafter\def\csname BAval@t05.r05.separable\endcsname{53.9}
\expandafter\def\csname BAval@t05.r05.temporal.q\endcsname{57.7}
\expandafter\def\csname BAval@t05.r05.bindadapt\endcsname{75.6}
\expandafter\def\csname BAval@t05.r05.oracle\endcsname{82.9}
\expandafter\def\csname BAval@t05.r06.separable\endcsname{37.9}
\expandafter\def\csname BAval@t05.r06.temporal.q\endcsname{42.1}
\expandafter\def\csname BAval@t05.r06.bindadapt\endcsname{64.0}
\expandafter\def\csname BAval@t05.r06.oracle\endcsname{72.9}
\expandafter\def\csname BAval@t06.r01.temporal.q\endcsname{54.1}
\expandafter\def\csname BAval@t06.r01.joint.belief\endcsname{56.1}
\expandafter\def\csname BAval@t06.r01.bindadapt\endcsname{70.2}
\expandafter\def\csname BAval@t06.r01.oracle\endcsname{77.0}
\expandafter\def\csname BAval@t06.r02.temporal.q\endcsname{62.0}
\expandafter\def\csname BAval@t06.r02.joint.belief\endcsname{64.0}
\expandafter\def\csname BAval@t06.r02.bindadapt\endcsname{77.1}
\expandafter\def\csname BAval@t06.r02.oracle\endcsname{84.0}
\expandafter\def\csname BAval@t06.r03.temporal.q\endcsname{68.7}
\expandafter\def\csname BAval@t06.r03.joint.belief\endcsname{70.3}
\expandafter\def\csname BAval@t06.r03.bindadapt\endcsname{82.3}
\expandafter\def\csname BAval@t06.r03.oracle\endcsname{87.9}
\expandafter\def\csname BAval@t06.r04.temporal.q\endcsname{72.3}
\expandafter\def\csname BAval@t06.r04.joint.belief\endcsname{74.3}
\expandafter\def\csname BAval@t06.r04.bindadapt\endcsname{84.5}
\expandafter\def\csname BAval@t06.r04.oracle\endcsname{90.2}
\expandafter\def\csname BAval@t06.r05.temporal.q\endcsname{74.7}
\expandafter\def\csname BAval@t06.r05.joint.belief\endcsname{76.1}
\expandafter\def\csname BAval@t06.r05.bindadapt\endcsname{85.6}
\expandafter\def\csname BAval@t06.r05.oracle\endcsname{91.0}
\expandafter\def\csname BAval@t06.r06.temporal.q\endcsname{75.9}
\expandafter\def\csname BAval@t06.r06.joint.belief\endcsname{77.6}
\expandafter\def\csname BAval@t06.r06.bindadapt\endcsname{86.2}
\expandafter\def\csname BAval@t06.r06.oracle\endcsname{91.4}
\expandafter\def\csname BAval@t07.r01.pair.rank.pct\endcsname{67.0}
\expandafter\def\csname BAval@t07.r01.risk.mae\endcsname{0.140}
\expandafter\def\csname BAval@t07.r01.calibration.error\endcsname{0.098}
\expandafter\def\csname BAval@t07.r01.action.regret\endcsname{0.125}
\expandafter\def\csname BAval@t07.r02.pair.rank.pct\endcsname{72.5}
\expandafter\def\csname BAval@t07.r02.risk.mae\endcsname{0.118}
\expandafter\def\csname BAval@t07.r02.calibration.error\endcsname{0.073}
\expandafter\def\csname BAval@t07.r02.action.regret\endcsname{0.091}
\expandafter\def\csname BAval@t07.r03.pair.rank.pct\endcsname{78.0}
\expandafter\def\csname BAval@t07.r03.risk.mae\endcsname{0.096}
\expandafter\def\csname BAval@t07.r03.calibration.error\endcsname{0.056}
\expandafter\def\csname BAval@t07.r03.action.regret\endcsname{0.068}
\expandafter\def\csname BAval@t07.r04.pair.rank.pct\endcsname{88.7}
\expandafter\def\csname BAval@t07.r04.risk.mae\endcsname{0.053}
\expandafter\def\csname BAval@t07.r04.calibration.error\endcsname{0.026}
\expandafter\def\csname BAval@t07.r04.action.regret\endcsname{0.032}
\expandafter\def\csname BAval@t08.r01.sid\endcsname{82.3}
\expandafter\def\csname BAval@t08.r02.sid\endcsname{82.8}
\expandafter\def\csname BAval@t08.r03.sid\endcsname{86.1}
\expandafter\def\csname BAval@t08.r04.sid\endcsname{87.9}
\expandafter\def\csname BAval@t08.r05.sid\endcsname{94.1}
\expandafter\def\csname BAval@t08.r06.sid\endcsname{98.0}
\expandafter\def\csname BAval@t09.r01.groups\endcsname{60}
\expandafter\def\csname BAval@t09.r01.episodes\endcsname{1200}
\expandafter\def\csname BAval@t09.r02.groups\endcsname{20}
\expandafter\def\csname BAval@t09.r02.episodes\endcsname{200}
\expandafter\def\csname BAval@t09.r03.groups\endcsname{40}
\expandafter\def\csname BAval@t09.r03.episodes\endcsname{480}
\expandafter\def\csname BAval@t10.r01.separable\endcsname{68.6}
\expandafter\def\csname BAval@t10.r01.temporal.q\endcsname{70.1}
\expandafter\def\csname BAval@t10.r01.bindadapt\endcsname{82.3}
\expandafter\def\csname BAval@t10.r02.separable\endcsname{65.3}
\expandafter\def\csname BAval@t10.r02.temporal.q\endcsname{67.0}
\expandafter\def\csname BAval@t10.r02.bindadapt\endcsname{80.1}
\expandafter\def\csname BAval@t10.r03.separable\endcsname{61.8}
\expandafter\def\csname BAval@t10.r03.temporal.q\endcsname{65.2}
\expandafter\def\csname BAval@t10.r03.bindadapt\endcsname{78.1}
\expandafter\def\csname BAval@t10.r04.separable\endcsname{58.9}
\expandafter\def\csname BAval@t10.r04.temporal.q\endcsname{62.9}
\expandafter\def\csname BAval@t10.r04.bindadapt\endcsname{76.1}
\expandafter\def\csname BAval@t10.r05.separable\endcsname{62.4}
\expandafter\def\csname BAval@t10.r05.temporal.q\endcsname{64.9}
\expandafter\def\csname BAval@t10.r05.bindadapt\endcsname{77.1}
\expandafter\def\csname BAval@t11.r01.reference\endcsname{91.2}
\expandafter\def\csname BAval@t11.r01.bindadapt\endcsname{92.0}
\expandafter\def\csname BAval@t11.r01.gain.pp\endcsname{0.8}
\expandafter\def\csname BAval@t11.r02.reference\endcsname{93.9}
\expandafter\def\csname BAval@t11.r02.bindadapt\endcsname{94.1}
\expandafter\def\csname BAval@t11.r02.gain.pp\endcsname{0.2}
\expandafter\def\csname BAval@t11.r03.reference\endcsname{65.9}
\expandafter\def\csname BAval@t11.r03.bindadapt\endcsname{82.3}
\expandafter\def\csname BAval@t11.r03.gain.pp\endcsname{16.4}
\expandafter\def\csname BAval@t11.r04.reference\endcsname{40.9}
\expandafter\def\csname BAval@t11.r04.bindadapt\endcsname{41.3}
\expandafter\def\csname BAval@t11.r04.gain.pp\endcsname{0.4}
\expandafter\def\csname BAval@t11.r05.reference\endcsname{20.5}
\expandafter\def\csname BAval@t11.r05.bindadapt\endcsname{20.7}
\expandafter\def\csname BAval@t11.r05.gain.pp\endcsname{0.2}
\expandafter\def\csname BAval@t12.r01.sid\endcsname{60.9}
\expandafter\def\csname BAval@t12.r01.wrong\endcsname{14.6}
\expandafter\def\csname BAval@t12.r01.recovery\endcsname{59.0}
\expandafter\def\csname BAval@t12.r01.t5\endcsname{3.0}
\expandafter\def\csname BAval@t12.r02.sid\endcsname{62.5}
\expandafter\def\csname BAval@t12.r02.wrong\endcsname{13.8}
\expandafter\def\csname BAval@t12.r02.recovery\endcsname{61.1}
\expandafter\def\csname BAval@t12.r02.t5\endcsname{2.9}
\expandafter\def\csname BAval@t12.r03.sid\endcsname{65.3}
\expandafter\def\csname BAval@t12.r03.wrong\endcsname{12.2}
\expandafter\def\csname BAval@t12.r03.recovery\endcsname{64.9}
\expandafter\def\csname BAval@t12.r03.t5\endcsname{2.7}
\expandafter\def\csname BAval@t12.r04.sid\endcsname{66.4}
\expandafter\def\csname BAval@t12.r04.wrong\endcsname{11.8}
\expandafter\def\csname BAval@t12.r04.recovery\endcsname{67.1}
\expandafter\def\csname BAval@t12.r04.t5\endcsname{2.6}
\expandafter\def\csname BAval@t12.r05.sid\endcsname{71.0}
\expandafter\def\csname BAval@t12.r05.wrong\endcsname{8.8}
\expandafter\def\csname BAval@t12.r05.recovery\endcsname{73.0}
\expandafter\def\csname BAval@t12.r05.t5\endcsname{2.3}
\expandafter\def\csname BAval@t12.r06.sid\endcsname{62.0}
\expandafter\def\csname BAval@t12.r06.wrong\endcsname{14.3}
\expandafter\def\csname BAval@t12.r06.recovery\endcsname{64.0}
\expandafter\def\csname BAval@t12.r06.t5\endcsname{2.8}
\expandafter\def\csname BAval@t12.r07.sid\endcsname{65.6}
\expandafter\def\csname BAval@t12.r07.wrong\endcsname{10.4}
\expandafter\def\csname BAval@t12.r07.recovery\endcsname{68.0}
\expandafter\def\csname BAval@t12.r07.t5\endcsname{2.5}
\expandafter\def\csname BAval@t12.r08.sid\endcsname{70.3}
\expandafter\def\csname BAval@t12.r08.wrong\endcsname{8.1}
\expandafter\def\csname BAval@t12.r08.recovery\endcsname{74.0}
\expandafter\def\csname BAval@t12.r08.t5\endcsname{2.2}
\expandafter\def\csname BAval@t12.r09.sid\endcsname{66.5}
\expandafter\def\csname BAval@t12.r09.wrong\endcsname{10.9}
\expandafter\def\csname BAval@t12.r09.recovery\endcsname{68.0}
\expandafter\def\csname BAval@t12.r09.t5\endcsname{2.6}
\expandafter\def\csname BAval@t12.r10.sid\endcsname{72.8}
\expandafter\def\csname BAval@t12.r10.wrong\endcsname{7.8}
\expandafter\def\csname BAval@t12.r10.recovery\endcsname{76.1}
\expandafter\def\csname BAval@t12.r10.t5\endcsname{2.1}
\expandafter\def\csname BAval@t12.r11.sid\endcsname{68.0}
\expandafter\def\csname BAval@t12.r11.wrong\endcsname{10.1}
\expandafter\def\csname BAval@t12.r11.recovery\endcsname{69.0}
\expandafter\def\csname BAval@t12.r11.t5\endcsname{2.5}
\expandafter\def\csname BAval@t12.r12.sid\endcsname{71.6}
\expandafter\def\csname BAval@t12.r12.wrong\endcsname{8.6}
\expandafter\def\csname BAval@t12.r12.recovery\endcsname{73.9}
\expandafter\def\csname BAval@t12.r12.t5\endcsname{2.2}
\expandafter\def\csname BAval@t12.r13.sid\endcsname{74.1}
\expandafter\def\csname BAval@t12.r13.wrong\endcsname{7.4}
\expandafter\def\csname BAval@t12.r13.recovery\endcsname{77.1}
\expandafter\def\csname BAval@t12.r13.t5\endcsname{2.1}
\expandafter\def\csname BAval@t12.r14.sid\endcsname{74.6}
\expandafter\def\csname BAval@t12.r14.wrong\endcsname{6.9}
\expandafter\def\csname BAval@t12.r14.recovery\endcsname{77.9}
\expandafter\def\csname BAval@t12.r14.t5\endcsname{2.0}
\expandafter\def\csname BAval@t12.r15.sid\endcsname{75.2}
\expandafter\def\csname BAval@t12.r15.wrong\endcsname{7.3}
\expandafter\def\csname BAval@t12.r15.recovery\endcsname{79.0}
\expandafter\def\csname BAval@t12.r15.t5\endcsname{2.0}
\expandafter\def\csname BAval@t12.r16.sid\endcsname{82.3}
\expandafter\def\csname BAval@t12.r16.wrong\endcsname{4.4}
\expandafter\def\csname BAval@t12.r16.recovery\endcsname{86.2}
\expandafter\def\csname BAval@t12.r16.t5\endcsname{1.4}
\expandafter\def\csname BAval@t13.r01.ao\endcsname{63.9}
\expandafter\def\csname BAval@t13.r01.p20.pct\endcsname{76.6}
\expandafter\def\csname BAval@t13.r01.pn20\endcsname{78.1}
\expandafter\def\csname BAval@t13.r01.sr50.pct\endcsname{74.2}
\expandafter\def\csname BAval@t13.r01.sr75.pct\endcsname{49.6}
\expandafter\def\csname BAval@t13.r01.sao.pct\endcsname{58.3}
\expandafter\def\csname BAval@t13.r01.ssr50.pct\endcsname{66.7}
\expandafter\def\csname BAval@t13.r01.ssr75.pct\endcsname{41.0}
\expandafter\def\csname BAval@t13.r02.ao\endcsname{65.0}
\expandafter\def\csname BAval@t13.r02.p20.pct\endcsname{77.9}
\expandafter\def\csname BAval@t13.r02.pn20\endcsname{79.2}
\expandafter\def\csname BAval@t13.r02.sr50.pct\endcsname{75.5}
\expandafter\def\csname BAval@t13.r02.sr75.pct\endcsname{51.4}
\expandafter\def\csname BAval@t13.r02.sao.pct\endcsname{59.2}
\expandafter\def\csname BAval@t13.r02.ssr50.pct\endcsname{67.9}
\expandafter\def\csname BAval@t13.r02.ssr75.pct\endcsname{42.4}
\expandafter\def\csname BAval@t13.r03.ao\endcsname{67.7}
\expandafter\def\csname BAval@t13.r03.p20.pct\endcsname{79.7}
\expandafter\def\csname BAval@t13.r03.pn20\endcsname{81.5}
\expandafter\def\csname BAval@t13.r03.sr50.pct\endcsname{78.5}
\expandafter\def\csname BAval@t13.r03.sr75.pct\endcsname{55.8}
\expandafter\def\csname BAval@t13.r03.sao.pct\endcsname{61.9}
\expandafter\def\csname BAval@t13.r03.ssr50.pct\endcsname{70.6}
\expandafter\def\csname BAval@t13.r03.ssr75.pct\endcsname{45.7}
\expandafter\def\csname BAval@t13.r04.ao\endcsname{68.6}
\expandafter\def\csname BAval@t13.r04.p20.pct\endcsname{80.2}
\expandafter\def\csname BAval@t13.r04.pn20\endcsname{82.0}
\expandafter\def\csname BAval@t13.r04.sr50.pct\endcsname{79.5}
\expandafter\def\csname BAval@t13.r04.sr75.pct\endcsname{57.1}
\expandafter\def\csname BAval@t13.r04.sao.pct\endcsname{62.5}
\expandafter\def\csname BAval@t13.r04.ssr50.pct\endcsname{71.4}
\expandafter\def\csname BAval@t13.r04.ssr75.pct\endcsname{47.2}
\expandafter\def\csname BAval@t13.r05.ao\endcsname{72.7}
\expandafter\def\csname BAval@t13.r05.p20.pct\endcsname{84.9}
\expandafter\def\csname BAval@t13.r05.pn20\endcsname{86.0}
\expandafter\def\csname BAval@t13.r05.sr50.pct\endcsname{83.6}
\expandafter\def\csname BAval@t13.r05.sr75.pct\endcsname{63.2}
\expandafter\def\csname BAval@t13.r05.sao.pct\endcsname{67.0}
\expandafter\def\csname BAval@t13.r05.ssr50.pct\endcsname{76.1}
\expandafter\def\csname BAval@t13.r05.ssr75.pct\endcsname{53.6}
\expandafter\def\csname BAval@t13.r06.ao\endcsname{63.7}
\expandafter\def\csname BAval@t13.r06.p20.pct\endcsname{75.3}
\expandafter\def\csname BAval@t13.r06.pn20\endcsname{77.1}
\expandafter\def\csname BAval@t13.r06.sr50.pct\endcsname{74.1}
\expandafter\def\csname BAval@t13.r06.sr75.pct\endcsname{48.3}
\expandafter\def\csname BAval@t13.r06.sao.pct\endcsname{57.8}
\expandafter\def\csname BAval@t13.r06.ssr50.pct\endcsname{66.1}
\expandafter\def\csname BAval@t13.r06.ssr75.pct\endcsname{40.6}
\expandafter\def\csname BAval@t13.r07.ao\endcsname{67.0}
\expandafter\def\csname BAval@t13.r07.p20.pct\endcsname{78.9}
\expandafter\def\csname BAval@t13.r07.pn20\endcsname{80.5}
\expandafter\def\csname BAval@t13.r07.sr50.pct\endcsname{77.9}
\expandafter\def\csname BAval@t13.r07.sr75.pct\endcsname{54.1}
\expandafter\def\csname BAval@t13.r07.sao.pct\endcsname{61.9}
\expandafter\def\csname BAval@t13.r07.ssr50.pct\endcsname{69.9}
\expandafter\def\csname BAval@t13.r07.ssr75.pct\endcsname{46.3}
\expandafter\def\csname BAval@t13.r08.ao\endcsname{73.3}
\expandafter\def\csname BAval@t13.r08.p20.pct\endcsname{84.5}
\expandafter\def\csname BAval@t13.r08.pn20\endcsname{85.9}
\expandafter\def\csname BAval@t13.r08.sr50.pct\endcsname{84.3}
\expandafter\def\csname BAval@t13.r08.sr75.pct\endcsname{63.6}
\expandafter\def\csname BAval@t13.r08.sao.pct\endcsname{66.7}
\expandafter\def\csname BAval@t13.r08.ssr50.pct\endcsname{75.8}
\expandafter\def\csname BAval@t13.r08.ssr75.pct\endcsname{53.0}
\expandafter\def\csname BAval@t13.r09.ao\endcsname{67.3}
\expandafter\def\csname BAval@t13.r09.p20.pct\endcsname{79.2}
\expandafter\def\csname BAval@t13.r09.pn20\endcsname{80.6}
\expandafter\def\csname BAval@t13.r09.sr50.pct\endcsname{78.4}
\expandafter\def\csname BAval@t13.r09.sr75.pct\endcsname{54.7}
\expandafter\def\csname BAval@t13.r09.sao.pct\endcsname{64.6}
\expandafter\def\csname BAval@t13.r09.ssr50.pct\endcsname{73.6}
\expandafter\def\csname BAval@t13.r09.ssr75.pct\endcsname{49.9}
\expandafter\def\csname BAval@t13.r10.ao\endcsname{72.0}
\expandafter\def\csname BAval@t13.r10.p20.pct\endcsname{83.2}
\expandafter\def\csname BAval@t13.r10.pn20\endcsname{84.7}
\expandafter\def\csname BAval@t13.r10.sr50.pct\endcsname{82.7}
\expandafter\def\csname BAval@t13.r10.sr75.pct\endcsname{61.8}
\expandafter\def\csname BAval@t13.r10.sao.pct\endcsname{68.3}
\expandafter\def\csname BAval@t13.r10.ssr50.pct\endcsname{77.0}
\expandafter\def\csname BAval@t13.r10.ssr75.pct\endcsname{55.4}
\expandafter\def\csname BAval@t13.r11.ao\endcsname{79.1}
\expandafter\def\csname BAval@t13.r11.p20.pct\endcsname{88.0}
\expandafter\def\csname BAval@t13.r11.pn20\endcsname{89.3}
\expandafter\def\csname BAval@t13.r11.sr50.pct\endcsname{88.0}
\expandafter\def\csname BAval@t13.r11.sr75.pct\endcsname{71.5}
\expandafter\def\csname BAval@t13.r11.sao.pct\endcsname{76.9}
\expandafter\def\csname BAval@t13.r11.ssr50.pct\endcsname{83.9}
\expandafter\def\csname BAval@t13.r11.ssr75.pct\endcsname{67.2}
\expandafter\def\csname BAval@t14.r01.short\endcsname{84.0}
\expandafter\def\csname BAval@t14.r01.similar\endcsname{75.9}
\expandafter\def\csname BAval@t14.r01.long\endcsname{55.5}
\expandafter\def\csname BAval@t14.r01.weighted\endcsname{70.3}
\expandafter\def\csname BAval@t14.r02.short\endcsname{85.5}
\expandafter\def\csname BAval@t14.r02.similar\endcsname{77.2}
\expandafter\def\csname BAval@t14.r02.long\endcsname{59.9}
\expandafter\def\csname BAval@t14.r02.weighted\endcsname{72.8}
\expandafter\def\csname BAval@t14.r03.short\endcsname{84.8}
\expandafter\def\csname BAval@t14.r03.similar\endcsname{76.5}
\expandafter\def\csname BAval@t14.r03.long\endcsname{58.0}
\expandafter\def\csname BAval@t14.r03.weighted\endcsname{71.6}
\expandafter\def\csname BAval@t14.r04.short\endcsname{85.4}
\expandafter\def\csname BAval@t14.r04.similar\endcsname{78.8}
\expandafter\def\csname BAval@t14.r04.long\endcsname{61.9}
\expandafter\def\csname BAval@t14.r04.weighted\endcsname{74.1}
\expandafter\def\csname BAval@t14.r05.short\endcsname{86.2}
\expandafter\def\csname BAval@t14.r05.similar\endcsname{79.2}
\expandafter\def\csname BAval@t14.r05.long\endcsname{63.9}
\expandafter\def\csname BAval@t14.r05.weighted\endcsname{75.2}
\expandafter\def\csname BAval@t14.r06.short\endcsname{90.2}
\expandafter\def\csname BAval@t14.r06.similar\endcsname{85.4}
\expandafter\def\csname BAval@t14.r06.long\endcsname{73.9}
\expandafter\def\csname BAval@t14.r06.weighted\endcsname{82.3}
\expandafter\def\csname BAval@t14.r07.short\endcsname{74.9}
\expandafter\def\csname BAval@t14.r07.similar\endcsname{65.7}
\expandafter\def\csname BAval@t14.r07.long\endcsname{46.8}
\expandafter\def\csname BAval@t14.r07.weighted\endcsname{60.9}
\expandafter\def\csname BAval@t14.r08.short\endcsname{76.5}
\expandafter\def\csname BAval@t14.r08.similar\endcsname{67.3}
\expandafter\def\csname BAval@t14.r08.long\endcsname{48.3}
\expandafter\def\csname BAval@t14.r08.weighted\endcsname{62.5}
\expandafter\def\csname BAval@t14.r09.short\endcsname{79.1}
\expandafter\def\csname BAval@t14.r09.similar\endcsname{70.2}
\expandafter\def\csname BAval@t14.r09.long\endcsname{51.1}
\expandafter\def\csname BAval@t14.r09.weighted\endcsname{65.3}
\expandafter\def\csname BAval@t14.r10.short\endcsname{80.6}
\expandafter\def\csname BAval@t14.r10.similar\endcsname{71.3}
\expandafter\def\csname BAval@t14.r10.long\endcsname{52.1}
\expandafter\def\csname BAval@t14.r10.weighted\endcsname{66.4}
\expandafter\def\csname BAval@t14.r11.short\endcsname{84.9}
\expandafter\def\csname BAval@t14.r11.similar\endcsname{75.8}
\expandafter\def\csname BAval@t14.r11.long\endcsname{57.1}
\expandafter\def\csname BAval@t14.r11.weighted\endcsname{71.0}
\expandafter\def\csname BAval@t14.r12.short\endcsname{76.1}
\expandafter\def\csname BAval@t14.r12.similar\endcsname{66.9}
\expandafter\def\csname BAval@t14.r12.long\endcsname{47.7}
\expandafter\def\csname BAval@t14.r12.weighted\endcsname{62.0}
\expandafter\def\csname BAval@t14.r13.short\endcsname{79.7}
\expandafter\def\csname BAval@t14.r13.similar\endcsname{70.8}
\expandafter\def\csname BAval@t14.r13.long\endcsname{50.9}
\expandafter\def\csname BAval@t14.r13.weighted\endcsname{65.6}
\expandafter\def\csname BAval@t14.r14.short\endcsname{80.6}
\expandafter\def\csname BAval@t14.r14.similar\endcsname{71.7}
\expandafter\def\csname BAval@t14.r14.long\endcsname{52.0}
\expandafter\def\csname BAval@t14.r14.weighted\endcsname{66.5}
\expandafter\def\csname BAval@t14.r15.short\endcsname{82.0}
\expandafter\def\csname BAval@t14.r15.similar\endcsname{73.1}
\expandafter\def\csname BAval@t14.r15.long\endcsname{53.6}
\expandafter\def\csname BAval@t14.r15.weighted\endcsname{68.0}
\expandafter\def\csname BAval@t14.r16.short\endcsname{88.6}
\expandafter\def\csname BAval@t14.r16.similar\endcsname{79.7}
\expandafter\def\csname BAval@t14.r16.long\endcsname{60.3}
\expandafter\def\csname BAval@t14.r16.weighted\endcsname{74.6}
\expandafter\def\csname BAval@t15.r01.common.controller\endcsname{60.9}
\expandafter\def\csname BAval@t15.r01.oa.vat.ptz\endcsname{66.8}
\expandafter\def\csname BAval@t15.r01.chanakya.j\endcsname{68.9}
\expandafter\def\csname BAval@t15.r01.bindadapt\endcsname{77.1}
\expandafter\def\csname BAval@t15.r02.common.controller\endcsname{71.0}
\expandafter\def\csname BAval@t15.r02.oa.vat.ptz\endcsname{73.2}
\expandafter\def\csname BAval@t15.r02.chanakya.j\endcsname{73.8}
\expandafter\def\csname BAval@t15.r02.bindadapt\endcsname{81.5}
\expandafter\def\csname BAval@t15.r03.common.controller\endcsname{70.3}
\expandafter\def\csname BAval@t15.r03.oa.vat.ptz\endcsname{74.3}
\expandafter\def\csname BAval@t15.r03.chanakya.j\endcsname{75.2}
\expandafter\def\csname BAval@t15.r03.bindadapt\endcsname{82.3}
\expandafter\def\csname BAval@t16.r01.tracking.precision.pct\endcsname{72.9}
\expandafter\def\csname BAval@t16.r01.tracking.recall.pct\endcsname{65.3}
\expandafter\def\csname BAval@t16.r01.fmax.pct\endcsname{68.9}
\expandafter\def\csname BAval@t16.r01.operating.precision.pct\endcsname{72.1}
\expandafter\def\csname BAval@t16.r01.operating.recall.pct\endcsname{63.0}
\expandafter\def\csname BAval@t16.r01.f.operating.pct\endcsname{67.2}
\expandafter\def\csname BAval@t16.r02.tracking.precision.pct\endcsname{75.9}
\expandafter\def\csname BAval@t16.r02.tracking.recall.pct\endcsname{68.2}
\expandafter\def\csname BAval@t16.r02.fmax.pct\endcsname{71.9}
\expandafter\def\csname BAval@t16.r02.operating.precision.pct\endcsname{74.9}
\expandafter\def\csname BAval@t16.r02.operating.recall.pct\endcsname{66.2}
\expandafter\def\csname BAval@t16.r02.f.operating.pct\endcsname{70.2}
\expandafter\def\csname BAval@t16.r03.tracking.precision.pct\endcsname{79.0}
\expandafter\def\csname BAval@t16.r03.tracking.recall.pct\endcsname{73.5}
\expandafter\def\csname BAval@t16.r03.fmax.pct\endcsname{76.1}
\expandafter\def\csname BAval@t16.r03.operating.precision.pct\endcsname{77.9}
\expandafter\def\csname BAval@t16.r03.operating.recall.pct\endcsname{71.4}
\expandafter\def\csname BAval@t16.r03.f.operating.pct\endcsname{74.5}
\expandafter\def\csname BAval@t16.r04.tracking.precision.pct\endcsname{80.0}
\expandafter\def\csname BAval@t16.r04.tracking.recall.pct\endcsname{74.3}
\expandafter\def\csname BAval@t16.r04.fmax.pct\endcsname{77.0}
\expandafter\def\csname BAval@t16.r04.operating.precision.pct\endcsname{79.1}
\expandafter\def\csname BAval@t16.r04.operating.recall.pct\endcsname{72.5}
\expandafter\def\csname BAval@t16.r04.f.operating.pct\endcsname{75.6}
\expandafter\def\csname BAval@t16.r05.tracking.precision.pct\endcsname{80.9}
\expandafter\def\csname BAval@t16.r05.tracking.recall.pct\endcsname{75.0}
\expandafter\def\csname BAval@t16.r05.fmax.pct\endcsname{77.9}
\expandafter\def\csname BAval@t16.r05.operating.precision.pct\endcsname{80.1}
\expandafter\def\csname BAval@t16.r05.operating.recall.pct\endcsname{72.8}
\expandafter\def\csname BAval@t16.r05.f.operating.pct\endcsname{76.3}
\expandafter\def\csname BAval@t16.r06.tracking.precision.pct\endcsname{82.0}
\expandafter\def\csname BAval@t16.r06.tracking.recall.pct\endcsname{76.1}
\expandafter\def\csname BAval@t16.r06.fmax.pct\endcsname{78.9}
\expandafter\def\csname BAval@t16.r06.operating.precision.pct\endcsname{81.1}
\expandafter\def\csname BAval@t16.r06.operating.recall.pct\endcsname{74.1}
\expandafter\def\csname BAval@t16.r06.f.operating.pct\endcsname{77.4}
\expandafter\def\csname BAval@t16.r07.tracking.precision.pct\endcsname{87.4}
\expandafter\def\csname BAval@t16.r07.tracking.recall.pct\endcsname{82.8}
\expandafter\def\csname BAval@t16.r07.fmax.pct\endcsname{85.0}
\expandafter\def\csname BAval@t16.r07.operating.precision.pct\endcsname{86.5}
\expandafter\def\csname BAval@t16.r07.operating.recall.pct\endcsname{81.2}
\expandafter\def\csname BAval@t16.r07.f.operating.pct\endcsname{83.8}
\expandafter\def\csname BAval@t17.r01.dam4sam\endcsname{79.4}
\expandafter\def\csname BAval@t17.r01.oa.vat.ptz\endcsname{81.2}
\expandafter\def\csname BAval@t17.r01.artrack.ac\endcsname{80.1}
\expandafter\def\csname BAval@t17.r01.chanakya.j\endcsname{81.3}
\expandafter\def\csname BAval@t17.r01.dam4sam.chanakya.j\endcsname{82.0}
\expandafter\def\csname BAval@t17.r01.bindadapt\endcsname{86.1}
\expandafter\def\csname BAval@t17.r02.dam4sam\endcsname{78.0}
\expandafter\def\csname BAval@t17.r02.oa.vat.ptz\endcsname{79.8}
\expandafter\def\csname BAval@t17.r02.artrack.ac\endcsname{78.9}
\expandafter\def\csname BAval@t17.r02.chanakya.j\endcsname{80.1}
\expandafter\def\csname BAval@t17.r02.dam4sam.chanakya.j\endcsname{81.1}
\expandafter\def\csname BAval@t17.r02.bindadapt\endcsname{85.3}
\expandafter\def\csname BAval@t17.r03.dam4sam\endcsname{74.5}
\expandafter\def\csname BAval@t17.r03.oa.vat.ptz\endcsname{76.8}
\expandafter\def\csname BAval@t17.r03.artrack.ac\endcsname{75.9}
\expandafter\def\csname BAval@t17.r03.chanakya.j\endcsname{77.8}
\expandafter\def\csname BAval@t17.r03.dam4sam.chanakya.j\endcsname{78.7}
\expandafter\def\csname BAval@t17.r03.bindadapt\endcsname{83.8}
\expandafter\def\csname BAval@t17.r04.dam4sam\endcsname{70.3}
\expandafter\def\csname BAval@t17.r04.oa.vat.ptz\endcsname{72.8}
\expandafter\def\csname BAval@t17.r04.artrack.ac\endcsname{71.6}
\expandafter\def\csname BAval@t17.r04.chanakya.j\endcsname{74.1}
\expandafter\def\csname BAval@t17.r04.dam4sam.chanakya.j\endcsname{75.2}
\expandafter\def\csname BAval@t17.r04.bindadapt\endcsname{82.3}
\expandafter\def\csname BAval@t17.r05.dam4sam\endcsname{58.6}
\expandafter\def\csname BAval@t17.r05.oa.vat.ptz\endcsname{62.0}
\expandafter\def\csname BAval@t17.r05.artrack.ac\endcsname{61.8}
\expandafter\def\csname BAval@t17.r05.chanakya.j\endcsname{65.7}
\expandafter\def\csname BAval@t17.r05.dam4sam.chanakya.j\endcsname{66.9}
\expandafter\def\csname BAval@t17.r05.bindadapt\endcsname{75.6}
\expandafter\def\csname BAval@t17.r06.dam4sam\endcsname{40.1}
\expandafter\def\csname BAval@t17.r06.oa.vat.ptz\endcsname{45.4}
\expandafter\def\csname BAval@t17.r06.artrack.ac\endcsname{44.9}
\expandafter\def\csname BAval@t17.r06.chanakya.j\endcsname{50.0}
\expandafter\def\csname BAval@t17.r06.dam4sam.chanakya.j\endcsname{51.9}
\expandafter\def\csname BAval@t17.r06.bindadapt\endcsname{64.0}
\expandafter\def\csname BAval@t17.r07.dam4sam\endcsname{52.8}
\expandafter\def\csname BAval@t17.r07.oa.vat.ptz\endcsname{56.9}
\expandafter\def\csname BAval@t17.r07.artrack.ac\endcsname{59.1}
\expandafter\def\csname BAval@t17.r07.chanakya.j\endcsname{60.5}
\expandafter\def\csname BAval@t17.r07.dam4sam.chanakya.j\endcsname{61.5}
\expandafter\def\csname BAval@t17.r07.bindadapt\endcsname{70.2}
\expandafter\def\csname BAval@t17.r08.dam4sam\endcsname{62.8}
\expandafter\def\csname BAval@t17.r08.oa.vat.ptz\endcsname{65.7}
\expandafter\def\csname BAval@t17.r08.artrack.ac\endcsname{66.5}
\expandafter\def\csname BAval@t17.r08.chanakya.j\endcsname{68.2}
\expandafter\def\csname BAval@t17.r08.dam4sam.chanakya.j\endcsname{69.5}
\expandafter\def\csname BAval@t17.r08.bindadapt\endcsname{77.1}
\expandafter\def\csname BAval@t17.r09.dam4sam\endcsname{70.3}
\expandafter\def\csname BAval@t17.r09.oa.vat.ptz\endcsname{72.8}
\expandafter\def\csname BAval@t17.r09.artrack.ac\endcsname{71.6}
\expandafter\def\csname BAval@t17.r09.chanakya.j\endcsname{74.1}
\expandafter\def\csname BAval@t17.r09.dam4sam.chanakya.j\endcsname{75.2}
\expandafter\def\csname BAval@t17.r09.bindadapt\endcsname{82.3}
\expandafter\def\csname BAval@t17.r10.dam4sam\endcsname{73.4}
\expandafter\def\csname BAval@t17.r10.oa.vat.ptz\endcsname{76.0}
\expandafter\def\csname BAval@t17.r10.artrack.ac\endcsname{75.2}
\expandafter\def\csname BAval@t17.r10.chanakya.j\endcsname{77.3}
\expandafter\def\csname BAval@t17.r10.dam4sam.chanakya.j\endcsname{78.7}
\expandafter\def\csname BAval@t17.r10.bindadapt\endcsname{84.5}
\expandafter\def\csname BAval@t17.r11.dam4sam\endcsname{75.5}
\expandafter\def\csname BAval@t17.r11.oa.vat.ptz\endcsname{77.3}
\expandafter\def\csname BAval@t17.r11.artrack.ac\endcsname{76.7}
\expandafter\def\csname BAval@t17.r11.chanakya.j\endcsname{78.6}
\expandafter\def\csname BAval@t17.r11.dam4sam.chanakya.j\endcsname{79.5}
\expandafter\def\csname BAval@t17.r11.bindadapt\endcsname{85.6}
\expandafter\def\csname BAval@t17.r12.dam4sam\endcsname{76.8}
\expandafter\def\csname BAval@t17.r12.oa.vat.ptz\endcsname{78.5}
\expandafter\def\csname BAval@t17.r12.artrack.ac\endcsname{78.0}
\expandafter\def\csname BAval@t17.r12.chanakya.j\endcsname{79.7}
\expandafter\def\csname BAval@t17.r12.dam4sam.chanakya.j\endcsname{80.8}
\expandafter\def\csname BAval@t17.r12.bindadapt\endcsname{86.2}
\expandafter\def\csname BAval@t18.r01.mean.inference.ms\endcsname{16.0}
\expandafter\def\csname BAval@t18.r01.p95.inference.ms\endcsname{21.9}
\expandafter\def\csname BAval@t18.r01.fps\endcsname{62.5}
\expandafter\def\csname BAval@t18.r01.decision.overhead.ms\endcsname{0.5}
\expandafter\def\csname BAval@t18.r02.mean.inference.ms\endcsname{23.1}
\expandafter\def\csname BAval@t18.r02.p95.inference.ms\endcsname{31.2}
\expandafter\def\csname BAval@t18.r02.fps\endcsname{43.4}
\expandafter\def\csname BAval@t18.r02.decision.overhead.ms\endcsname{0.5}
\expandafter\def\csname BAval@t18.r03.mean.inference.ms\endcsname{36.2}
\expandafter\def\csname BAval@t18.r03.p95.inference.ms\endcsname{48.8}
\expandafter\def\csname BAval@t18.r03.fps\endcsname{27.6}
\expandafter\def\csname BAval@t18.r03.decision.overhead.ms\endcsname{0.5}
\expandafter\def\csname BAval@t18.r04.mean.inference.ms\endcsname{19.5}
\expandafter\def\csname BAval@t18.r04.p95.inference.ms\endcsname{28.1}
\expandafter\def\csname BAval@t18.r04.fps\endcsname{51.4}
\expandafter\def\csname BAval@t18.r04.decision.overhead.ms\endcsname{1.5}
\expandafter\def\csname BAval@t18.r05.mean.inference.ms\endcsname{17.1}
\expandafter\def\csname BAval@t18.r05.p95.inference.ms\endcsname{24.8}
\expandafter\def\csname BAval@t18.r05.fps\endcsname{58.6}
\expandafter\def\csname BAval@t18.r05.decision.overhead.ms\endcsname{1.2}
\expandafter\def\csname BAval@t18.r06.mean.inference.ms\endcsname{26.1}
\expandafter\def\csname BAval@t18.r06.p95.inference.ms\endcsname{39.3}
\expandafter\def\csname BAval@t18.r06.fps\endcsname{38.3}
\expandafter\def\csname BAval@t18.r06.decision.overhead.ms\endcsname{5.6}
\expandafter\def\csname BAval@t18.r07.mean.inference.ms\endcsname{23.9}
\expandafter\def\csname BAval@t18.r07.p95.inference.ms\endcsname{34.3}
\expandafter\def\csname BAval@t18.r07.fps\endcsname{41.8}
\expandafter\def\csname BAval@t18.r07.decision.overhead.ms\endcsname{1.8}
\expandafter\def\csname BAval@t18.r08.mean.inference.ms\endcsname{37.8}
\expandafter\def\csname BAval@t18.r08.p95.inference.ms\endcsname{52.2}
\expandafter\def\csname BAval@t18.r08.fps\endcsname{26.4}
\expandafter\def\csname BAval@t18.r08.decision.overhead.ms\endcsname{1.8}
\expandafter\def\csname BAval@t18.r09.mean.inference.ms\endcsname{37.4}
\expandafter\def\csname BAval@t18.r09.p95.inference.ms\endcsname{51.7}
\expandafter\def\csname BAval@t18.r09.fps\endcsname{26.8}
\expandafter\def\csname BAval@t18.r09.decision.overhead.ms\endcsname{2.1}
\expandafter\def\csname BAval@t19.r01.auc.la0.pct\endcsname{67.0}
\expandafter\def\csname BAval@t19.r01.dp.la0.pct\endcsname{73.5}
\expandafter\def\csname BAval@t19.r01.mauc.pct\endcsname{69.8}
\expandafter\def\csname BAval@t19.r01.mdp.pct\endcsname{76.6}
\expandafter\def\csname BAval@t19.r02.auc.la0.pct\endcsname{66.7}
\expandafter\def\csname BAval@t19.r02.dp.la0.pct\endcsname{73.8}
\expandafter\def\csname BAval@t19.r02.mauc.pct\endcsname{69.5}
\expandafter\def\csname BAval@t19.r02.mdp.pct\endcsname{76.7}
\expandafter\def\csname BAval@t19.r03.auc.la0.pct\endcsname{64.6}
\expandafter\def\csname BAval@t19.r03.dp.la0.pct\endcsname{76.0}
\expandafter\def\csname BAval@t19.r03.mauc.pct\endcsname{66.4}
\expandafter\def\csname BAval@t19.r03.mdp.pct\endcsname{78.0}
\expandafter\def\csname BAval@t19.r04.auc.la0.pct\endcsname{68.3}
\expandafter\def\csname BAval@t19.r04.dp.la0.pct\endcsname{78.2}
\expandafter\def\csname BAval@t19.r04.mauc.pct\endcsname{70.2}
\expandafter\def\csname BAval@t19.r04.mdp.pct\endcsname{80.4}
\expandafter\def\csname BAval@t19.r05.auc.la0.pct\endcsname{67.7}
\expandafter\def\csname BAval@t19.r05.dp.la0.pct\endcsname{79.1}
\expandafter\def\csname BAval@t19.r05.mauc.pct\endcsname{69.8}
\expandafter\def\csname BAval@t19.r05.mdp.pct\endcsname{81.2}
\expandafter\def\csname BAval@t19.r06.auc.la0.pct\endcsname{76.9}
\expandafter\def\csname BAval@t19.r06.dp.la0.pct\endcsname{85.1}
\expandafter\def\csname BAval@t19.r06.mauc.pct\endcsname{78.1}
\expandafter\def\csname BAval@t19.r06.mdp.pct\endcsname{86.7}
\expandafter\def\csname BAval@t20.r01.auc.pct\endcsname{67.0}
\expandafter\def\csname BAval@t20.r01.dp.pct\endcsname{73.5}
\expandafter\def\csname BAval@t20.r02.auc.pct\endcsname{67.2}
\expandafter\def\csname BAval@t20.r02.dp.pct\endcsname{73.7}
\expandafter\def\csname BAval@t20.r03.auc.pct\endcsname{67.3}
\expandafter\def\csname BAval@t20.r03.dp.pct\endcsname{73.9}
\expandafter\def\csname BAval@t20.r04.auc.pct\endcsname{67.5}
\expandafter\def\csname BAval@t20.r04.dp.pct\endcsname{74.0}
\expandafter\def\csname BAval@t20.r05.auc.pct\endcsname{67.6}
\expandafter\def\csname BAval@t20.r05.dp.pct\endcsname{74.2}
\expandafter\def\csname BAval@t20.r06.auc.pct\endcsname{67.8}
\expandafter\def\csname BAval@t20.r06.dp.pct\endcsname{74.4}
\expandafter\def\csname BAval@t20.r07.auc.pct\endcsname{67.9}
\expandafter\def\csname BAval@t20.r07.dp.pct\endcsname{74.5}
\expandafter\def\csname BAval@t20.r08.auc.pct\endcsname{68.1}
\expandafter\def\csname BAval@t20.r08.dp.pct\endcsname{74.7}
\expandafter\def\csname BAval@t20.r09.auc.pct\endcsname{68.2}
\expandafter\def\csname BAval@t20.r09.dp.pct\endcsname{74.9}
\expandafter\def\csname BAval@t20.r10.auc.pct\endcsname{68.4}
\expandafter\def\csname BAval@t20.r10.dp.pct\endcsname{75.0}
\expandafter\def\csname BAval@t20.r11.auc.pct\endcsname{68.5}
\expandafter\def\csname BAval@t20.r11.dp.pct\endcsname{75.2}
\expandafter\def\csname BAval@t20.r12.auc.pct\endcsname{68.6}
\expandafter\def\csname BAval@t20.r12.dp.pct\endcsname{75.3}
\expandafter\def\csname BAval@t20.r13.auc.pct\endcsname{68.8}
\expandafter\def\csname BAval@t20.r13.dp.pct\endcsname{75.4}
\expandafter\def\csname BAval@t20.r14.auc.pct\endcsname{68.9}
\expandafter\def\csname BAval@t20.r14.dp.pct\endcsname{75.6}
\expandafter\def\csname BAval@t20.r15.auc.pct\endcsname{69.0}
\expandafter\def\csname BAval@t20.r15.dp.pct\endcsname{75.7}
\expandafter\def\csname BAval@t20.r16.auc.pct\endcsname{69.1}
\expandafter\def\csname BAval@t20.r16.dp.pct\endcsname{75.8}
\expandafter\def\csname BAval@t20.r17.auc.pct\endcsname{69.3}
\expandafter\def\csname BAval@t20.r17.dp.pct\endcsname{76.0}
\expandafter\def\csname BAval@t20.r18.auc.pct\endcsname{69.4}
\expandafter\def\csname BAval@t20.r18.dp.pct\endcsname{76.1}
\expandafter\def\csname BAval@t20.r19.auc.pct\endcsname{69.5}
\expandafter\def\csname BAval@t20.r19.dp.pct\endcsname{76.2}
\expandafter\def\csname BAval@t20.r20.auc.pct\endcsname{69.6}
\expandafter\def\csname BAval@t20.r20.dp.pct\endcsname{76.3}
\expandafter\def\csname BAval@t20.r21.auc.pct\endcsname{69.7}
\expandafter\def\csname BAval@t20.r21.dp.pct\endcsname{76.4}
\expandafter\def\csname BAval@t20.r22.auc.pct\endcsname{69.8}
\expandafter\def\csname BAval@t20.r22.dp.pct\endcsname{76.6}
\expandafter\def\csname BAval@t20.r23.auc.pct\endcsname{69.9}
\expandafter\def\csname BAval@t20.r23.dp.pct\endcsname{76.7}
\expandafter\def\csname BAval@t20.r24.auc.pct\endcsname{70.0}
\expandafter\def\csname BAval@t20.r24.dp.pct\endcsname{76.8}
\expandafter\def\csname BAval@t20.r25.auc.pct\endcsname{70.1}
\expandafter\def\csname BAval@t20.r25.dp.pct\endcsname{76.9}
\expandafter\def\csname BAval@t20.r26.auc.pct\endcsname{70.2}
\expandafter\def\csname BAval@t20.r26.dp.pct\endcsname{77.0}
\expandafter\def\csname BAval@t20.r27.auc.pct\endcsname{70.2}
\expandafter\def\csname BAval@t20.r27.dp.pct\endcsname{77.0}
\expandafter\def\csname BAval@t20.r28.auc.pct\endcsname{70.3}
\expandafter\def\csname BAval@t20.r28.dp.pct\endcsname{77.1}
\expandafter\def\csname BAval@t20.r29.auc.pct\endcsname{70.4}
\expandafter\def\csname BAval@t20.r29.dp.pct\endcsname{77.2}
\expandafter\def\csname BAval@t20.r30.auc.pct\endcsname{70.5}
\expandafter\def\csname BAval@t20.r30.dp.pct\endcsname{77.3}
\expandafter\def\csname BAval@t20.r31.auc.pct\endcsname{70.5}
\expandafter\def\csname BAval@t20.r31.dp.pct\endcsname{77.4}
\expandafter\def\csname BAval@t20.r32.auc.pct\endcsname{70.6}
\expandafter\def\csname BAval@t20.r32.dp.pct\endcsname{77.4}
\expandafter\def\csname BAval@t20.r33.auc.pct\endcsname{70.7}
\expandafter\def\csname BAval@t20.r33.dp.pct\endcsname{77.5}
\expandafter\def\csname BAval@t20.r34.auc.pct\endcsname{70.7}
\expandafter\def\csname BAval@t20.r34.dp.pct\endcsname{77.6}
\expandafter\def\csname BAval@t20.r35.auc.pct\endcsname{70.8}
\expandafter\def\csname BAval@t20.r35.dp.pct\endcsname{77.6}
\expandafter\def\csname BAval@t20.r36.auc.pct\endcsname{70.8}
\expandafter\def\csname BAval@t20.r36.dp.pct\endcsname{77.7}
\expandafter\def\csname BAval@t20.r37.auc.pct\endcsname{70.9}
\expandafter\def\csname BAval@t20.r37.dp.pct\endcsname{77.7}
\expandafter\def\csname BAval@t20.r38.auc.pct\endcsname{70.9}
\expandafter\def\csname BAval@t20.r38.dp.pct\endcsname{77.8}
\expandafter\def\csname BAval@t20.r39.auc.pct\endcsname{71.0}
\expandafter\def\csname BAval@t20.r39.dp.pct\endcsname{77.8}
\expandafter\def\csname BAval@t20.r40.auc.pct\endcsname{71.0}
\expandafter\def\csname BAval@t20.r40.dp.pct\endcsname{77.9}
\expandafter\def\csname BAval@t20.r41.auc.pct\endcsname{71.0}
\expandafter\def\csname BAval@t20.r41.dp.pct\endcsname{77.9}
\expandafter\def\csname BAval@t20.r42.auc.pct\endcsname{71.1}
\expandafter\def\csname BAval@t20.r42.dp.pct\endcsname{78.0}
\expandafter\def\csname BAval@t20.r43.auc.pct\endcsname{71.1}
\expandafter\def\csname BAval@t20.r43.dp.pct\endcsname{78.0}
\expandafter\def\csname BAval@t20.r44.auc.pct\endcsname{71.1}
\expandafter\def\csname BAval@t20.r44.dp.pct\endcsname{78.0}
\expandafter\def\csname BAval@t20.r45.auc.pct\endcsname{71.1}
\expandafter\def\csname BAval@t20.r45.dp.pct\endcsname{78.0}
\expandafter\def\csname BAval@t20.r46.auc.pct\endcsname{71.2}
\expandafter\def\csname BAval@t20.r46.dp.pct\endcsname{78.1}
\expandafter\def\csname BAval@t20.r47.auc.pct\endcsname{71.2}
\expandafter\def\csname BAval@t20.r47.dp.pct\endcsname{78.1}
\expandafter\def\csname BAval@t20.r48.auc.pct\endcsname{71.2}
\expandafter\def\csname BAval@t20.r48.dp.pct\endcsname{78.1}
\expandafter\def\csname BAval@t20.r49.auc.pct\endcsname{71.2}
\expandafter\def\csname BAval@t20.r49.dp.pct\endcsname{78.1}
\expandafter\def\csname BAval@t20.r50.auc.pct\endcsname{71.2}
\expandafter\def\csname BAval@t20.r50.dp.pct\endcsname{78.1}
\expandafter\def\csname BAval@t20.r51.auc.pct\endcsname{71.2}
\expandafter\def\csname BAval@t20.r51.dp.pct\endcsname{78.1}
\expandafter\def\csname BAval@t20.r52.auc.pct\endcsname{66.7}
\expandafter\def\csname BAval@t20.r52.dp.pct\endcsname{73.8}
\expandafter\def\csname BAval@t20.r53.auc.pct\endcsname{66.9}
\expandafter\def\csname BAval@t20.r53.dp.pct\endcsname{74.0}
\expandafter\def\csname BAval@t20.r54.auc.pct\endcsname{67.0}
\expandafter\def\csname BAval@t20.r54.dp.pct\endcsname{74.1}
\expandafter\def\csname BAval@t20.r55.auc.pct\endcsname{67.2}
\expandafter\def\csname BAval@t20.r55.dp.pct\endcsname{74.3}
\expandafter\def\csname BAval@t20.r56.auc.pct\endcsname{67.3}
\expandafter\def\csname BAval@t20.r56.dp.pct\endcsname{74.5}
\expandafter\def\csname BAval@t20.r57.auc.pct\endcsname{67.5}
\expandafter\def\csname BAval@t20.r57.dp.pct\endcsname{74.6}
\expandafter\def\csname BAval@t20.r58.auc.pct\endcsname{67.6}
\expandafter\def\csname BAval@t20.r58.dp.pct\endcsname{74.8}
\expandafter\def\csname BAval@t20.r59.auc.pct\endcsname{67.8}
\expandafter\def\csname BAval@t20.r59.dp.pct\endcsname{74.9}
\expandafter\def\csname BAval@t20.r60.auc.pct\endcsname{67.9}
\expandafter\def\csname BAval@t20.r60.dp.pct\endcsname{75.1}
\expandafter\def\csname BAval@t20.r61.auc.pct\endcsname{68.0}
\expandafter\def\csname BAval@t20.r61.dp.pct\endcsname{75.2}
\expandafter\def\csname BAval@t20.r62.auc.pct\endcsname{68.2}
\expandafter\def\csname BAval@t20.r62.dp.pct\endcsname{75.4}
\expandafter\def\csname BAval@t20.r63.auc.pct\endcsname{68.3}
\expandafter\def\csname BAval@t20.r63.dp.pct\endcsname{75.5}
\expandafter\def\csname BAval@t20.r64.auc.pct\endcsname{68.4}
\expandafter\def\csname BAval@t20.r64.dp.pct\endcsname{75.7}
\expandafter\def\csname BAval@t20.r65.auc.pct\endcsname{68.6}
\expandafter\def\csname BAval@t20.r65.dp.pct\endcsname{75.8}
\expandafter\def\csname BAval@t20.r66.auc.pct\endcsname{68.7}
\expandafter\def\csname BAval@t20.r66.dp.pct\endcsname{75.9}
\expandafter\def\csname BAval@t20.r67.auc.pct\endcsname{68.8}
\expandafter\def\csname BAval@t20.r67.dp.pct\endcsname{76.0}
\expandafter\def\csname BAval@t20.r68.auc.pct\endcsname{68.9}
\expandafter\def\csname BAval@t20.r68.dp.pct\endcsname{76.2}
\expandafter\def\csname BAval@t20.r69.auc.pct\endcsname{69.0}
\expandafter\def\csname BAval@t20.r69.dp.pct\endcsname{76.3}
\expandafter\def\csname BAval@t20.r70.auc.pct\endcsname{69.1}
\expandafter\def\csname BAval@t20.r70.dp.pct\endcsname{76.4}
\expandafter\def\csname BAval@t20.r71.auc.pct\endcsname{69.2}
\expandafter\def\csname BAval@t20.r71.dp.pct\endcsname{76.5}
\expandafter\def\csname BAval@t20.r72.auc.pct\endcsname{69.3}
\expandafter\def\csname BAval@t20.r72.dp.pct\endcsname{76.6}
\expandafter\def\csname BAval@t20.r73.auc.pct\endcsname{69.5}
\expandafter\def\csname BAval@t20.r73.dp.pct\endcsname{76.7}
\expandafter\def\csname BAval@t20.r74.auc.pct\endcsname{69.6}
\expandafter\def\csname BAval@t20.r74.dp.pct\endcsname{76.8}
\expandafter\def\csname BAval@t20.r75.auc.pct\endcsname{69.7}
\expandafter\def\csname BAval@t20.r75.dp.pct\endcsname{76.9}
\expandafter\def\csname BAval@t20.r76.auc.pct\endcsname{69.8}
\expandafter\def\csname BAval@t20.r76.dp.pct\endcsname{77.0}
\expandafter\def\csname BAval@t20.r77.auc.pct\endcsname{69.9}
\expandafter\def\csname BAval@t20.r77.dp.pct\endcsname{77.1}
\expandafter\def\csname BAval@t20.r78.auc.pct\endcsname{70.0}
\expandafter\def\csname BAval@t20.r78.dp.pct\endcsname{77.2}
\expandafter\def\csname BAval@t20.r79.auc.pct\endcsname{70.0}
\expandafter\def\csname BAval@t20.r79.dp.pct\endcsname{77.3}
\expandafter\def\csname BAval@t20.r80.auc.pct\endcsname{70.1}
\expandafter\def\csname BAval@t20.r80.dp.pct\endcsname{77.3}
\expandafter\def\csname BAval@t20.r81.auc.pct\endcsname{70.2}
\expandafter\def\csname BAval@t20.r81.dp.pct\endcsname{77.4}
\expandafter\def\csname BAval@t20.r82.auc.pct\endcsname{70.2}
\expandafter\def\csname BAval@t20.r82.dp.pct\endcsname{77.5}
\expandafter\def\csname BAval@t20.r83.auc.pct\endcsname{70.3}
\expandafter\def\csname BAval@t20.r83.dp.pct\endcsname{77.6}
\expandafter\def\csname BAval@t20.r84.auc.pct\endcsname{70.4}
\expandafter\def\csname BAval@t20.r84.dp.pct\endcsname{77.6}
\expandafter\def\csname BAval@t20.r85.auc.pct\endcsname{70.4}
\expandafter\def\csname BAval@t20.r85.dp.pct\endcsname{77.7}
\expandafter\def\csname BAval@t20.r86.auc.pct\endcsname{70.5}
\expandafter\def\csname BAval@t20.r86.dp.pct\endcsname{77.7}
\expandafter\def\csname BAval@t20.r87.auc.pct\endcsname{70.5}
\expandafter\def\csname BAval@t20.r87.dp.pct\endcsname{77.8}
\expandafter\def\csname BAval@t20.r88.auc.pct\endcsname{70.6}
\expandafter\def\csname BAval@t20.r88.dp.pct\endcsname{77.9}
\expandafter\def\csname BAval@t20.r89.auc.pct\endcsname{70.6}
\expandafter\def\csname BAval@t20.r89.dp.pct\endcsname{77.9}
\expandafter\def\csname BAval@t20.r90.auc.pct\endcsname{70.7}
\expandafter\def\csname BAval@t20.r90.dp.pct\endcsname{77.9}
\expandafter\def\csname BAval@t20.r91.auc.pct\endcsname{70.7}
\expandafter\def\csname BAval@t20.r91.dp.pct\endcsname{78.0}
\expandafter\def\csname BAval@t20.r92.auc.pct\endcsname{70.7}
\expandafter\def\csname BAval@t20.r92.dp.pct\endcsname{78.0}
\expandafter\def\csname BAval@t20.r93.auc.pct\endcsname{70.8}
\expandafter\def\csname BAval@t20.r93.dp.pct\endcsname{78.1}
\expandafter\def\csname BAval@t20.r94.auc.pct\endcsname{70.8}
\expandafter\def\csname BAval@t20.r94.dp.pct\endcsname{78.1}
\expandafter\def\csname BAval@t20.r95.auc.pct\endcsname{70.8}
\expandafter\def\csname BAval@t20.r95.dp.pct\endcsname{78.1}
\expandafter\def\csname BAval@t20.r96.auc.pct\endcsname{70.8}
\expandafter\def\csname BAval@t20.r96.dp.pct\endcsname{78.1}
\expandafter\def\csname BAval@t20.r97.auc.pct\endcsname{70.9}
\expandafter\def\csname BAval@t20.r97.dp.pct\endcsname{78.2}
\expandafter\def\csname BAval@t20.r98.auc.pct\endcsname{70.9}
\expandafter\def\csname BAval@t20.r98.dp.pct\endcsname{78.2}
\expandafter\def\csname BAval@t20.r99.auc.pct\endcsname{70.9}
\expandafter\def\csname BAval@t20.r99.dp.pct\endcsname{78.2}
\expandafter\def\csname BAval@t20.r100.auc.pct\endcsname{70.9}
\expandafter\def\csname BAval@t20.r100.dp.pct\endcsname{78.2}
\expandafter\def\csname BAval@t20.r101.auc.pct\endcsname{70.9}
\expandafter\def\csname BAval@t20.r101.dp.pct\endcsname{78.2}
\expandafter\def\csname BAval@t20.r102.auc.pct\endcsname{70.9}
\expandafter\def\csname BAval@t20.r102.dp.pct\endcsname{78.2}
\expandafter\def\csname BAval@t20.r103.auc.pct\endcsname{64.6}
\expandafter\def\csname BAval@t20.r103.dp.pct\endcsname{76.0}
\expandafter\def\csname BAval@t20.r104.auc.pct\endcsname{64.7}
\expandafter\def\csname BAval@t20.r104.dp.pct\endcsname{76.1}
\expandafter\def\csname BAval@t20.r105.auc.pct\endcsname{64.8}
\expandafter\def\csname BAval@t20.r105.dp.pct\endcsname{76.2}
\expandafter\def\csname BAval@t20.r106.auc.pct\endcsname{64.9}
\expandafter\def\csname BAval@t20.r106.dp.pct\endcsname{76.4}
\expandafter\def\csname BAval@t20.r107.auc.pct\endcsname{65.0}
\expandafter\def\csname BAval@t20.r107.dp.pct\endcsname{76.5}
\expandafter\def\csname BAval@t20.r108.auc.pct\endcsname{65.1}
\expandafter\def\csname BAval@t20.r108.dp.pct\endcsname{76.6}
\expandafter\def\csname BAval@t20.r109.auc.pct\endcsname{65.2}
\expandafter\def\csname BAval@t20.r109.dp.pct\endcsname{76.7}
\expandafter\def\csname BAval@t20.r110.auc.pct\endcsname{65.3}
\expandafter\def\csname BAval@t20.r110.dp.pct\endcsname{76.8}
\expandafter\def\csname BAval@t20.r111.auc.pct\endcsname{65.4}
\expandafter\def\csname BAval@t20.r111.dp.pct\endcsname{76.9}
\expandafter\def\csname BAval@t20.r112.auc.pct\endcsname{65.5}
\expandafter\def\csname BAval@t20.r112.dp.pct\endcsname{77.0}
\expandafter\def\csname BAval@t20.r113.auc.pct\endcsname{65.5}
\expandafter\def\csname BAval@t20.r113.dp.pct\endcsname{77.1}
\expandafter\def\csname BAval@t20.r114.auc.pct\endcsname{65.7}
\expandafter\def\csname BAval@t20.r114.dp.pct\endcsname{77.2}
\expandafter\def\csname BAval@t20.r115.auc.pct\endcsname{65.8}
\expandafter\def\csname BAval@t20.r115.dp.pct\endcsname{77.3}
\expandafter\def\csname BAval@t20.r116.auc.pct\endcsname{65.9}
\expandafter\def\csname BAval@t20.r116.dp.pct\endcsname{77.4}
\expandafter\def\csname BAval@t20.r117.auc.pct\endcsname{66.0}
\expandafter\def\csname BAval@t20.r117.dp.pct\endcsname{77.5}
\expandafter\def\csname BAval@t20.r118.auc.pct\endcsname{66.0}
\expandafter\def\csname BAval@t20.r118.dp.pct\endcsname{77.6}
\expandafter\def\csname BAval@t20.r119.auc.pct\endcsname{66.1}
\expandafter\def\csname BAval@t20.r119.dp.pct\endcsname{77.7}
\expandafter\def\csname BAval@t20.r120.auc.pct\endcsname{66.2}
\expandafter\def\csname BAval@t20.r120.dp.pct\endcsname{77.7}
\expandafter\def\csname BAval@t20.r121.auc.pct\endcsname{66.2}
\expandafter\def\csname BAval@t20.r121.dp.pct\endcsname{77.8}
\expandafter\def\csname BAval@t20.r122.auc.pct\endcsname{66.3}
\expandafter\def\csname BAval@t20.r122.dp.pct\endcsname{77.9}
\expandafter\def\csname BAval@t20.r123.auc.pct\endcsname{66.4}
\expandafter\def\csname BAval@t20.r123.dp.pct\endcsname{78.0}
\expandafter\def\csname BAval@t20.r124.auc.pct\endcsname{66.4}
\expandafter\def\csname BAval@t20.r124.dp.pct\endcsname{78.1}
\expandafter\def\csname BAval@t20.r125.auc.pct\endcsname{66.5}
\expandafter\def\csname BAval@t20.r125.dp.pct\endcsname{78.1}
\expandafter\def\csname BAval@t20.r126.auc.pct\endcsname{66.5}
\expandafter\def\csname BAval@t20.r126.dp.pct\endcsname{78.2}
\expandafter\def\csname BAval@t20.r127.auc.pct\endcsname{66.6}
\expandafter\def\csname BAval@t20.r127.dp.pct\endcsname{78.3}
\expandafter\def\csname BAval@t20.r128.auc.pct\endcsname{66.7}
\expandafter\def\csname BAval@t20.r128.dp.pct\endcsname{78.3}
\expandafter\def\csname BAval@t20.r129.auc.pct\endcsname{66.7}
\expandafter\def\csname BAval@t20.r129.dp.pct\endcsname{78.4}
\expandafter\def\csname BAval@t20.r130.auc.pct\endcsname{66.7}
\expandafter\def\csname BAval@t20.r130.dp.pct\endcsname{78.4}
\expandafter\def\csname BAval@t20.r131.auc.pct\endcsname{66.8}
\expandafter\def\csname BAval@t20.r131.dp.pct\endcsname{78.5}
\expandafter\def\csname BAval@t20.r132.auc.pct\endcsname{66.8}
\expandafter\def\csname BAval@t20.r132.dp.pct\endcsname{78.6}
\expandafter\def\csname BAval@t20.r133.auc.pct\endcsname{66.9}
\expandafter\def\csname BAval@t20.r133.dp.pct\endcsname{78.6}
\expandafter\def\csname BAval@t20.r134.auc.pct\endcsname{66.9}
\expandafter\def\csname BAval@t20.r134.dp.pct\endcsname{78.7}
\expandafter\def\csname BAval@t20.r135.auc.pct\endcsname{67.0}
\expandafter\def\csname BAval@t20.r135.dp.pct\endcsname{78.7}
\expandafter\def\csname BAval@t20.r136.auc.pct\endcsname{67.0}
\expandafter\def\csname BAval@t20.r136.dp.pct\endcsname{78.7}
\expandafter\def\csname BAval@t20.r137.auc.pct\endcsname{67.0}
\expandafter\def\csname BAval@t20.r137.dp.pct\endcsname{78.8}
\expandafter\def\csname BAval@t20.r138.auc.pct\endcsname{67.1}
\expandafter\def\csname BAval@t20.r138.dp.pct\endcsname{78.8}
\expandafter\def\csname BAval@t20.r139.auc.pct\endcsname{67.1}
\expandafter\def\csname BAval@t20.r139.dp.pct\endcsname{78.9}
\expandafter\def\csname BAval@t20.r140.auc.pct\endcsname{67.1}
\expandafter\def\csname BAval@t20.r140.dp.pct\endcsname{78.9}
\expandafter\def\csname BAval@t20.r141.auc.pct\endcsname{67.2}
\expandafter\def\csname BAval@t20.r141.dp.pct\endcsname{78.9}
\expandafter\def\csname BAval@t20.r142.auc.pct\endcsname{67.2}
\expandafter\def\csname BAval@t20.r142.dp.pct\endcsname{78.9}
\expandafter\def\csname BAval@t20.r143.auc.pct\endcsname{67.2}
\expandafter\def\csname BAval@t20.r143.dp.pct\endcsname{79.0}
\expandafter\def\csname BAval@t20.r144.auc.pct\endcsname{67.2}
\expandafter\def\csname BAval@t20.r144.dp.pct\endcsname{79.0}
\expandafter\def\csname BAval@t20.r145.auc.pct\endcsname{67.2}
\expandafter\def\csname BAval@t20.r145.dp.pct\endcsname{79.0}
\expandafter\def\csname BAval@t20.r146.auc.pct\endcsname{67.2}
\expandafter\def\csname BAval@t20.r146.dp.pct\endcsname{79.0}
\expandafter\def\csname BAval@t20.r147.auc.pct\endcsname{67.3}
\expandafter\def\csname BAval@t20.r147.dp.pct\endcsname{79.1}
\expandafter\def\csname BAval@t20.r148.auc.pct\endcsname{67.3}
\expandafter\def\csname BAval@t20.r148.dp.pct\endcsname{79.1}
\expandafter\def\csname BAval@t20.r149.auc.pct\endcsname{67.3}
\expandafter\def\csname BAval@t20.r149.dp.pct\endcsname{79.1}
\expandafter\def\csname BAval@t20.r150.auc.pct\endcsname{67.3}
\expandafter\def\csname BAval@t20.r150.dp.pct\endcsname{79.1}
\expandafter\def\csname BAval@t20.r151.auc.pct\endcsname{67.3}
\expandafter\def\csname BAval@t20.r151.dp.pct\endcsname{79.1}
\expandafter\def\csname BAval@t20.r152.auc.pct\endcsname{67.3}
\expandafter\def\csname BAval@t20.r152.dp.pct\endcsname{79.1}
\expandafter\def\csname BAval@t20.r153.auc.pct\endcsname{67.3}
\expandafter\def\csname BAval@t20.r153.dp.pct\endcsname{79.1}
\expandafter\def\csname BAval@t20.r154.auc.pct\endcsname{68.3}
\expandafter\def\csname BAval@t20.r154.dp.pct\endcsname{78.2}
\expandafter\def\csname BAval@t20.r155.auc.pct\endcsname{68.4}
\expandafter\def\csname BAval@t20.r155.dp.pct\endcsname{78.3}
\expandafter\def\csname BAval@t20.r156.auc.pct\endcsname{68.5}
\expandafter\def\csname BAval@t20.r156.dp.pct\endcsname{78.5}
\expandafter\def\csname BAval@t20.r157.auc.pct\endcsname{68.5}
\expandafter\def\csname BAval@t20.r157.dp.pct\endcsname{78.6}
\expandafter\def\csname BAval@t20.r158.auc.pct\endcsname{68.7}
\expandafter\def\csname BAval@t20.r158.dp.pct\endcsname{78.7}
\expandafter\def\csname BAval@t20.r159.auc.pct\endcsname{68.8}
\expandafter\def\csname BAval@t20.r159.dp.pct\endcsname{78.8}
\expandafter\def\csname BAval@t20.r160.auc.pct\endcsname{68.9}
\expandafter\def\csname BAval@t20.r160.dp.pct\endcsname{78.9}
\expandafter\def\csname BAval@t20.r161.auc.pct\endcsname{69.0}
\expandafter\def\csname BAval@t20.r161.dp.pct\endcsname{79.1}
\expandafter\def\csname BAval@t20.r162.auc.pct\endcsname{69.1}
\expandafter\def\csname BAval@t20.r162.dp.pct\endcsname{79.2}
\expandafter\def\csname BAval@t20.r163.auc.pct\endcsname{69.2}
\expandafter\def\csname BAval@t20.r163.dp.pct\endcsname{79.3}
\expandafter\def\csname BAval@t20.r164.auc.pct\endcsname{69.3}
\expandafter\def\csname BAval@t20.r164.dp.pct\endcsname{79.4}
\expandafter\def\csname BAval@t20.r165.auc.pct\endcsname{69.4}
\expandafter\def\csname BAval@t20.r165.dp.pct\endcsname{79.5}
\expandafter\def\csname BAval@t20.r166.auc.pct\endcsname{69.5}
\expandafter\def\csname BAval@t20.r166.dp.pct\endcsname{79.6}
\expandafter\def\csname BAval@t20.r167.auc.pct\endcsname{69.6}
\expandafter\def\csname BAval@t20.r167.dp.pct\endcsname{79.7}
\expandafter\def\csname BAval@t20.r168.auc.pct\endcsname{69.6}
\expandafter\def\csname BAval@t20.r168.dp.pct\endcsname{79.8}
\expandafter\def\csname BAval@t20.r169.auc.pct\endcsname{69.7}
\expandafter\def\csname BAval@t20.r169.dp.pct\endcsname{79.9}
\expandafter\def\csname BAval@t20.r170.auc.pct\endcsname{69.8}
\expandafter\def\csname BAval@t20.r170.dp.pct\endcsname{80.0}
\expandafter\def\csname BAval@t20.r171.auc.pct\endcsname{69.9}
\expandafter\def\csname BAval@t20.r171.dp.pct\endcsname{80.1}
\expandafter\def\csname BAval@t20.r172.auc.pct\endcsname{70.0}
\expandafter\def\csname BAval@t20.r172.dp.pct\endcsname{80.1}
\expandafter\def\csname BAval@t20.r173.auc.pct\endcsname{70.0}
\expandafter\def\csname BAval@t20.r173.dp.pct\endcsname{80.2}
\expandafter\def\csname BAval@t20.r174.auc.pct\endcsname{70.1}
\expandafter\def\csname BAval@t20.r174.dp.pct\endcsname{80.3}
\expandafter\def\csname BAval@t20.r175.auc.pct\endcsname{70.2}
\expandafter\def\csname BAval@t20.r175.dp.pct\endcsname{80.4}
\expandafter\def\csname BAval@t20.r176.auc.pct\endcsname{70.3}
\expandafter\def\csname BAval@t20.r176.dp.pct\endcsname{80.5}
\expandafter\def\csname BAval@t20.r177.auc.pct\endcsname{70.3}
\expandafter\def\csname BAval@t20.r177.dp.pct\endcsname{80.5}
\expandafter\def\csname BAval@t20.r178.auc.pct\endcsname{70.4}
\expandafter\def\csname BAval@t20.r178.dp.pct\endcsname{80.6}
\expandafter\def\csname BAval@t20.r179.auc.pct\endcsname{70.5}
\expandafter\def\csname BAval@t20.r179.dp.pct\endcsname{80.7}
\expandafter\def\csname BAval@t20.r180.auc.pct\endcsname{70.5}
\expandafter\def\csname BAval@t20.r180.dp.pct\endcsname{80.7}
\expandafter\def\csname BAval@t20.r181.auc.pct\endcsname{70.5}
\expandafter\def\csname BAval@t20.r181.dp.pct\endcsname{80.8}
\expandafter\def\csname BAval@t20.r182.auc.pct\endcsname{70.5}
\expandafter\def\csname BAval@t20.r182.dp.pct\endcsname{80.9}
\expandafter\def\csname BAval@t20.r183.auc.pct\endcsname{70.6}
\expandafter\def\csname BAval@t20.r183.dp.pct\endcsname{80.9}
\expandafter\def\csname BAval@t20.r184.auc.pct\endcsname{70.6}
\expandafter\def\csname BAval@t20.r184.dp.pct\endcsname{81.0}
\expandafter\def\csname BAval@t20.r185.auc.pct\endcsname{70.7}
\expandafter\def\csname BAval@t20.r185.dp.pct\endcsname{81.0}
\expandafter\def\csname BAval@t20.r186.auc.pct\endcsname{70.7}
\expandafter\def\csname BAval@t20.r186.dp.pct\endcsname{81.1}
\expandafter\def\csname BAval@t20.r187.auc.pct\endcsname{70.8}
\expandafter\def\csname BAval@t20.r187.dp.pct\endcsname{81.1}
\expandafter\def\csname BAval@t20.r188.auc.pct\endcsname{70.8}
\expandafter\def\csname BAval@t20.r188.dp.pct\endcsname{81.2}
\expandafter\def\csname BAval@t20.r189.auc.pct\endcsname{70.8}
\expandafter\def\csname BAval@t20.r189.dp.pct\endcsname{81.2}
\expandafter\def\csname BAval@t20.r190.auc.pct\endcsname{70.9}
\expandafter\def\csname BAval@t20.r190.dp.pct\endcsname{81.2}
\expandafter\def\csname BAval@t20.r191.auc.pct\endcsname{70.9}
\expandafter\def\csname BAval@t20.r191.dp.pct\endcsname{81.3}
\expandafter\def\csname BAval@t20.r192.auc.pct\endcsname{70.9}
\expandafter\def\csname BAval@t20.r192.dp.pct\endcsname{81.3}
\expandafter\def\csname BAval@t20.r193.auc.pct\endcsname{71.0}
\expandafter\def\csname BAval@t20.r193.dp.pct\endcsname{81.3}
\expandafter\def\csname BAval@t20.r194.auc.pct\endcsname{71.0}
\expandafter\def\csname BAval@t20.r194.dp.pct\endcsname{81.4}
\expandafter\def\csname BAval@t20.r195.auc.pct\endcsname{71.0}
\expandafter\def\csname BAval@t20.r195.dp.pct\endcsname{81.4}
\expandafter\def\csname BAval@t20.r196.auc.pct\endcsname{71.0}
\expandafter\def\csname BAval@t20.r196.dp.pct\endcsname{81.4}
\expandafter\def\csname BAval@t20.r197.auc.pct\endcsname{71.0}
\expandafter\def\csname BAval@t20.r197.dp.pct\endcsname{81.4}
\expandafter\def\csname BAval@t20.r198.auc.pct\endcsname{71.1}
\expandafter\def\csname BAval@t20.r198.dp.pct\endcsname{81.5}
\expandafter\def\csname BAval@t20.r199.auc.pct\endcsname{71.1}
\expandafter\def\csname BAval@t20.r199.dp.pct\endcsname{81.5}
\expandafter\def\csname BAval@t20.r200.auc.pct\endcsname{71.1}
\expandafter\def\csname BAval@t20.r200.dp.pct\endcsname{81.5}
\expandafter\def\csname BAval@t20.r201.auc.pct\endcsname{71.1}
\expandafter\def\csname BAval@t20.r201.dp.pct\endcsname{81.5}
\expandafter\def\csname BAval@t20.r202.auc.pct\endcsname{71.1}
\expandafter\def\csname BAval@t20.r202.dp.pct\endcsname{81.5}
\expandafter\def\csname BAval@t20.r203.auc.pct\endcsname{71.1}
\expandafter\def\csname BAval@t20.r203.dp.pct\endcsname{81.5}
\expandafter\def\csname BAval@t20.r204.auc.pct\endcsname{71.1}
\expandafter\def\csname BAval@t20.r204.dp.pct\endcsname{81.5}
\expandafter\def\csname BAval@t20.r205.auc.pct\endcsname{67.7}
\expandafter\def\csname BAval@t20.r205.dp.pct\endcsname{79.1}
\expandafter\def\csname BAval@t20.r206.auc.pct\endcsname{67.8}
\expandafter\def\csname BAval@t20.r206.dp.pct\endcsname{79.2}
\expandafter\def\csname BAval@t20.r207.auc.pct\endcsname{67.9}
\expandafter\def\csname BAval@t20.r207.dp.pct\endcsname{79.3}
\expandafter\def\csname BAval@t20.r208.auc.pct\endcsname{68.0}
\expandafter\def\csname BAval@t20.r208.dp.pct\endcsname{79.4}
\expandafter\def\csname BAval@t20.r209.auc.pct\endcsname{68.1}
\expandafter\def\csname BAval@t20.r209.dp.pct\endcsname{79.6}
\expandafter\def\csname BAval@t20.r210.auc.pct\endcsname{68.3}
\expandafter\def\csname BAval@t20.r210.dp.pct\endcsname{79.7}
\expandafter\def\csname BAval@t20.r211.auc.pct\endcsname{68.4}
\expandafter\def\csname BAval@t20.r211.dp.pct\endcsname{79.8}
\expandafter\def\csname BAval@t20.r212.auc.pct\endcsname{68.5}
\expandafter\def\csname BAval@t20.r212.dp.pct\endcsname{79.9}
\expandafter\def\csname BAval@t20.r213.auc.pct\endcsname{68.7}
\expandafter\def\csname BAval@t20.r213.dp.pct\endcsname{80.1}
\expandafter\def\csname BAval@t20.r214.auc.pct\endcsname{68.8}
\expandafter\def\csname BAval@t20.r214.dp.pct\endcsname{80.2}
\expandafter\def\csname BAval@t20.r215.auc.pct\endcsname{68.8}
\expandafter\def\csname BAval@t20.r215.dp.pct\endcsname{80.3}
\expandafter\def\csname BAval@t20.r216.auc.pct\endcsname{68.9}
\expandafter\def\csname BAval@t20.r216.dp.pct\endcsname{80.4}
\expandafter\def\csname BAval@t20.r217.auc.pct\endcsname{69.0}
\expandafter\def\csname BAval@t20.r217.dp.pct\endcsname{80.5}
\expandafter\def\csname BAval@t20.r218.auc.pct\endcsname{69.1}
\expandafter\def\csname BAval@t20.r218.dp.pct\endcsname{80.6}
\expandafter\def\csname BAval@t20.r219.auc.pct\endcsname{69.2}
\expandafter\def\csname BAval@t20.r219.dp.pct\endcsname{80.6}
\expandafter\def\csname BAval@t20.r220.auc.pct\endcsname{69.3}
\expandafter\def\csname BAval@t20.r220.dp.pct\endcsname{80.7}
\expandafter\def\csname BAval@t20.r221.auc.pct\endcsname{69.4}
\expandafter\def\csname BAval@t20.r221.dp.pct\endcsname{80.8}
\expandafter\def\csname BAval@t20.r222.auc.pct\endcsname{69.4}
\expandafter\def\csname BAval@t20.r222.dp.pct\endcsname{80.9}
\expandafter\def\csname BAval@t20.r223.auc.pct\endcsname{69.5}
\expandafter\def\csname BAval@t20.r223.dp.pct\endcsname{81.0}
\expandafter\def\csname BAval@t20.r224.auc.pct\endcsname{69.6}
\expandafter\def\csname BAval@t20.r224.dp.pct\endcsname{81.0}
\expandafter\def\csname BAval@t20.r225.auc.pct\endcsname{69.7}
\expandafter\def\csname BAval@t20.r225.dp.pct\endcsname{81.1}
\expandafter\def\csname BAval@t20.r226.auc.pct\endcsname{69.7}
\expandafter\def\csname BAval@t20.r226.dp.pct\endcsname{81.2}
\expandafter\def\csname BAval@t20.r227.auc.pct\endcsname{69.8}
\expandafter\def\csname BAval@t20.r227.dp.pct\endcsname{81.3}
\expandafter\def\csname BAval@t20.r228.auc.pct\endcsname{69.9}
\expandafter\def\csname BAval@t20.r228.dp.pct\endcsname{81.3}
\expandafter\def\csname BAval@t20.r229.auc.pct\endcsname{69.9}
\expandafter\def\csname BAval@t20.r229.dp.pct\endcsname{81.4}
\expandafter\def\csname BAval@t20.r230.auc.pct\endcsname{70.1}
\expandafter\def\csname BAval@t20.r230.dp.pct\endcsname{81.5}
\expandafter\def\csname BAval@t20.r231.auc.pct\endcsname{70.1}
\expandafter\def\csname BAval@t20.r231.dp.pct\endcsname{81.5}
\expandafter\def\csname BAval@t20.r232.auc.pct\endcsname{70.2}
\expandafter\def\csname BAval@t20.r232.dp.pct\endcsname{81.6}
\expandafter\def\csname BAval@t20.r233.auc.pct\endcsname{70.2}
\expandafter\def\csname BAval@t20.r233.dp.pct\endcsname{81.6}
\expandafter\def\csname BAval@t20.r234.auc.pct\endcsname{70.3}
\expandafter\def\csname BAval@t20.r234.dp.pct\endcsname{81.7}
\expandafter\def\csname BAval@t20.r235.auc.pct\endcsname{70.3}
\expandafter\def\csname BAval@t20.r235.dp.pct\endcsname{81.7}
\expandafter\def\csname BAval@t20.r236.auc.pct\endcsname{70.4}
\expandafter\def\csname BAval@t20.r236.dp.pct\endcsname{81.8}
\expandafter\def\csname BAval@t20.r237.auc.pct\endcsname{70.4}
\expandafter\def\csname BAval@t20.r237.dp.pct\endcsname{81.8}
\expandafter\def\csname BAval@t20.r238.auc.pct\endcsname{70.5}
\expandafter\def\csname BAval@t20.r238.dp.pct\endcsname{81.9}
\expandafter\def\csname BAval@t20.r239.auc.pct\endcsname{70.5}
\expandafter\def\csname BAval@t20.r239.dp.pct\endcsname{81.9}
\expandafter\def\csname BAval@t20.r240.auc.pct\endcsname{70.5}
\expandafter\def\csname BAval@t20.r240.dp.pct\endcsname{81.9}
\expandafter\def\csname BAval@t20.r241.auc.pct\endcsname{70.6}
\expandafter\def\csname BAval@t20.r241.dp.pct\endcsname{82.0}
\expandafter\def\csname BAval@t20.r242.auc.pct\endcsname{70.6}
\expandafter\def\csname BAval@t20.r242.dp.pct\endcsname{82.0}
\expandafter\def\csname BAval@t20.r243.auc.pct\endcsname{70.6}
\expandafter\def\csname BAval@t20.r243.dp.pct\endcsname{82.0}
\expandafter\def\csname BAval@t20.r244.auc.pct\endcsname{70.7}
\expandafter\def\csname BAval@t20.r244.dp.pct\endcsname{82.2}
\expandafter\def\csname BAval@t20.r245.auc.pct\endcsname{70.7}
\expandafter\def\csname BAval@t20.r245.dp.pct\endcsname{82.2}
\expandafter\def\csname BAval@t20.r246.auc.pct\endcsname{70.7}
\expandafter\def\csname BAval@t20.r246.dp.pct\endcsname{82.2}
\expandafter\def\csname BAval@t20.r247.auc.pct\endcsname{70.7}
\expandafter\def\csname BAval@t20.r247.dp.pct\endcsname{82.2}
\expandafter\def\csname BAval@t20.r248.auc.pct\endcsname{70.7}
\expandafter\def\csname BAval@t20.r248.dp.pct\endcsname{82.2}
\expandafter\def\csname BAval@t20.r249.auc.pct\endcsname{70.8}
\expandafter\def\csname BAval@t20.r249.dp.pct\endcsname{82.3}
\expandafter\def\csname BAval@t20.r250.auc.pct\endcsname{70.8}
\expandafter\def\csname BAval@t20.r250.dp.pct\endcsname{82.3}
\expandafter\def\csname BAval@t20.r251.auc.pct\endcsname{70.8}
\expandafter\def\csname BAval@t20.r251.dp.pct\endcsname{82.3}
\expandafter\def\csname BAval@t20.r252.auc.pct\endcsname{70.8}
\expandafter\def\csname BAval@t20.r252.dp.pct\endcsname{82.3}
\expandafter\def\csname BAval@t20.r253.auc.pct\endcsname{70.8}
\expandafter\def\csname BAval@t20.r253.dp.pct\endcsname{82.3}
\expandafter\def\csname BAval@t20.r254.auc.pct\endcsname{70.8}
\expandafter\def\csname BAval@t20.r254.dp.pct\endcsname{82.3}
\expandafter\def\csname BAval@t20.r255.auc.pct\endcsname{70.8}
\expandafter\def\csname BAval@t20.r255.dp.pct\endcsname{82.3}
\expandafter\def\csname BAval@t20.r256.auc.pct\endcsname{76.9}
\expandafter\def\csname BAval@t20.r256.dp.pct\endcsname{85.1}
\expandafter\def\csname BAval@t20.r257.auc.pct\endcsname{77.0}
\expandafter\def\csname BAval@t20.r257.dp.pct\endcsname{85.2}
\expandafter\def\csname BAval@t20.r258.auc.pct\endcsname{77.1}
\expandafter\def\csname BAval@t20.r258.dp.pct\endcsname{85.2}
\expandafter\def\csname BAval@t20.r259.auc.pct\endcsname{77.2}
\expandafter\def\csname BAval@t20.r259.dp.pct\endcsname{85.3}
\expandafter\def\csname BAval@t20.r260.auc.pct\endcsname{77.2}
\expandafter\def\csname BAval@t20.r260.dp.pct\endcsname{85.4}
\expandafter\def\csname BAval@t20.r261.auc.pct\endcsname{77.2}
\expandafter\def\csname BAval@t20.r261.dp.pct\endcsname{85.5}
\expandafter\def\csname BAval@t20.r262.auc.pct\endcsname{77.3}
\expandafter\def\csname BAval@t20.r262.dp.pct\endcsname{85.6}
\expandafter\def\csname BAval@t20.r263.auc.pct\endcsname{77.4}
\expandafter\def\csname BAval@t20.r263.dp.pct\endcsname{85.7}
\expandafter\def\csname BAval@t20.r264.auc.pct\endcsname{77.4}
\expandafter\def\csname BAval@t20.r264.dp.pct\endcsname{85.7}
\expandafter\def\csname BAval@t20.r265.auc.pct\endcsname{77.5}
\expandafter\def\csname BAval@t20.r265.dp.pct\endcsname{85.8}
\expandafter\def\csname BAval@t20.r266.auc.pct\endcsname{77.5}
\expandafter\def\csname BAval@t20.r266.dp.pct\endcsname{85.9}
\expandafter\def\csname BAval@t20.r267.auc.pct\endcsname{77.6}
\expandafter\def\csname BAval@t20.r267.dp.pct\endcsname{86.0}
\expandafter\def\csname BAval@t20.r268.auc.pct\endcsname{77.6}
\expandafter\def\csname BAval@t20.r268.dp.pct\endcsname{86.1}
\expandafter\def\csname BAval@t20.r269.auc.pct\endcsname{77.7}
\expandafter\def\csname BAval@t20.r269.dp.pct\endcsname{86.1}
\expandafter\def\csname BAval@t20.r270.auc.pct\endcsname{77.8}
\expandafter\def\csname BAval@t20.r270.dp.pct\endcsname{86.2}
\expandafter\def\csname BAval@t20.r271.auc.pct\endcsname{77.8}
\expandafter\def\csname BAval@t20.r271.dp.pct\endcsname{86.3}
\expandafter\def\csname BAval@t20.r272.auc.pct\endcsname{77.9}
\expandafter\def\csname BAval@t20.r272.dp.pct\endcsname{86.3}
\expandafter\def\csname BAval@t20.r273.auc.pct\endcsname{77.9}
\expandafter\def\csname BAval@t20.r273.dp.pct\endcsname{86.4}
\expandafter\def\csname BAval@t20.r274.auc.pct\endcsname{77.9}
\expandafter\def\csname BAval@t20.r274.dp.pct\endcsname{86.5}
\expandafter\def\csname BAval@t20.r275.auc.pct\endcsname{78.0}
\expandafter\def\csname BAval@t20.r275.dp.pct\endcsname{86.5}
\expandafter\def\csname BAval@t20.r276.auc.pct\endcsname{78.0}
\expandafter\def\csname BAval@t20.r276.dp.pct\endcsname{86.6}
\expandafter\def\csname BAval@t20.r277.auc.pct\endcsname{78.1}
\expandafter\def\csname BAval@t20.r277.dp.pct\endcsname{86.7}
\expandafter\def\csname BAval@t20.r278.auc.pct\endcsname{78.1}
\expandafter\def\csname BAval@t20.r278.dp.pct\endcsname{86.7}
\expandafter\def\csname BAval@t20.r279.auc.pct\endcsname{78.2}
\expandafter\def\csname BAval@t20.r279.dp.pct\endcsname{86.8}
\expandafter\def\csname BAval@t20.r280.auc.pct\endcsname{78.2}
\expandafter\def\csname BAval@t20.r280.dp.pct\endcsname{86.8}
\expandafter\def\csname BAval@t20.r281.auc.pct\endcsname{78.2}
\expandafter\def\csname BAval@t20.r281.dp.pct\endcsname{86.9}
\expandafter\def\csname BAval@t20.r282.auc.pct\endcsname{78.2}
\expandafter\def\csname BAval@t20.r282.dp.pct\endcsname{86.9}
\expandafter\def\csname BAval@t20.r283.auc.pct\endcsname{78.2}
\expandafter\def\csname BAval@t20.r283.dp.pct\endcsname{87.0}
\expandafter\def\csname BAval@t20.r284.auc.pct\endcsname{78.3}
\expandafter\def\csname BAval@t20.r284.dp.pct\endcsname{87.0}
\expandafter\def\csname BAval@t20.r285.auc.pct\endcsname{78.3}
\expandafter\def\csname BAval@t20.r285.dp.pct\endcsname{87.1}
\expandafter\def\csname BAval@t20.r286.auc.pct\endcsname{78.3}
\expandafter\def\csname BAval@t20.r286.dp.pct\endcsname{87.1}
\expandafter\def\csname BAval@t20.r287.auc.pct\endcsname{78.4}
\expandafter\def\csname BAval@t20.r287.dp.pct\endcsname{87.1}
\expandafter\def\csname BAval@t20.r288.auc.pct\endcsname{78.4}
\expandafter\def\csname BAval@t20.r288.dp.pct\endcsname{87.2}
\expandafter\def\csname BAval@t20.r289.auc.pct\endcsname{78.4}
\expandafter\def\csname BAval@t20.r289.dp.pct\endcsname{87.2}
\expandafter\def\csname BAval@t20.r290.auc.pct\endcsname{78.5}
\expandafter\def\csname BAval@t20.r290.dp.pct\endcsname{87.2}
\expandafter\def\csname BAval@t20.r291.auc.pct\endcsname{78.5}
\expandafter\def\csname BAval@t20.r291.dp.pct\endcsname{87.3}
\expandafter\def\csname BAval@t20.r292.auc.pct\endcsname{78.5}
\expandafter\def\csname BAval@t20.r292.dp.pct\endcsname{87.3}
\expandafter\def\csname BAval@t20.r293.auc.pct\endcsname{78.5}
\expandafter\def\csname BAval@t20.r293.dp.pct\endcsname{87.3}
\expandafter\def\csname BAval@t20.r294.auc.pct\endcsname{78.5}
\expandafter\def\csname BAval@t20.r294.dp.pct\endcsname{87.4}
\expandafter\def\csname BAval@t20.r295.auc.pct\endcsname{78.5}
\expandafter\def\csname BAval@t20.r295.dp.pct\endcsname{87.4}
\expandafter\def\csname BAval@t20.r296.auc.pct\endcsname{78.5}
\expandafter\def\csname BAval@t20.r296.dp.pct\endcsname{87.4}
\expandafter\def\csname BAval@t20.r297.auc.pct\endcsname{78.5}
\expandafter\def\csname BAval@t20.r297.dp.pct\endcsname{87.4}
\expandafter\def\csname BAval@t20.r298.auc.pct\endcsname{78.5}
\expandafter\def\csname BAval@t20.r298.dp.pct\endcsname{87.4}
\expandafter\def\csname BAval@t20.r299.auc.pct\endcsname{78.6}
\expandafter\def\csname BAval@t20.r299.dp.pct\endcsname{87.5}
\expandafter\def\csname BAval@t20.r300.auc.pct\endcsname{78.6}
\expandafter\def\csname BAval@t20.r300.dp.pct\endcsname{87.5}
\expandafter\def\csname BAval@t20.r301.auc.pct\endcsname{78.6}
\expandafter\def\csname BAval@t20.r301.dp.pct\endcsname{87.5}
\expandafter\def\csname BAval@t20.r302.auc.pct\endcsname{78.6}
\expandafter\def\csname BAval@t20.r302.dp.pct\endcsname{87.5}
\expandafter\def\csname BAval@t20.r303.auc.pct\endcsname{78.6}
\expandafter\def\csname BAval@t20.r303.dp.pct\endcsname{87.5}
\expandafter\def\csname BAval@t20.r304.auc.pct\endcsname{78.6}
\expandafter\def\csname BAval@t20.r304.dp.pct\endcsname{87.5}
\expandafter\def\csname BAval@t20.r305.auc.pct\endcsname{78.6}
\expandafter\def\csname BAval@t20.r305.dp.pct\endcsname{87.5}
\expandafter\def\csname BAval@t20.r306.auc.pct\endcsname{78.6}
\expandafter\def\csname BAval@t20.r306.dp.pct\endcsname{87.5}
\expandafter\def\csname BAval@t21.r01.car.pct\endcsname{89.3}
\expandafter\def\csname BAval@t21.r02.car.pct\endcsname{91.5}
\expandafter\def\csname BAval@t21.r03.car.pct\endcsname{95.0}
\expandafter\def\csname BAval@t21.r04.car.pct\endcsname{93.2}
\expandafter\def\csname BAval@t21.r05.car.pct\endcsname{94.0}
\expandafter\def\csname BAval@t22.r01.full.s.id.pct\endcsname{75.8}
\expandafter\def\csname BAval@t22.r01.ablated.s.id.pct\endcsname{67.7}
\expandafter\def\csname BAval@t22.r01.drop.pp\endcsname{8.2}
\expandafter\def\csname BAval@t22.r02.full.s.id.pct\endcsname{87.0}
\expandafter\def\csname BAval@t22.r02.ablated.s.id.pct\endcsname{85.8}
\expandafter\def\csname BAval@t22.r02.drop.pp\endcsname{1.1}
\expandafter\def\csname BAval@t22.r03.full.s.id.pct\endcsname{80.1}
\expandafter\def\csname BAval@t22.r03.ablated.s.id.pct\endcsname{73.8}
\expandafter\def\csname BAval@t22.r03.drop.pp\endcsname{6.3}
\expandafter\def\csname BAval@t22.r04.full.s.id.pct\endcsname{84.6}
\expandafter\def\csname BAval@t22.r04.ablated.s.id.pct\endcsname{84.2}
\expandafter\def\csname BAval@t22.r04.drop.pp\endcsname{0.4}
\expandafter\def\csname BAval@t23.r01.sid\endcsname{78.1}
\expandafter\def\csname BAval@t23.r02.sid\endcsname{81.0}
\expandafter\def\csname BAval@t23.r03.sid\endcsname{81.7}
\expandafter\def\csname BAval@t24.r01.sid\endcsname{81.6}
\expandafter\def\csname BAval@t24.r01.wrong\endcsname{4.9}
\expandafter\def\csname BAval@t24.r01.recovery\endcsname{84.6}
\expandafter\def\csname BAval@t24.r01.t5\endcsname{1.5}
\expandafter\def\csname BAval@t24.r02.sid\endcsname{82.1}
\expandafter\def\csname BAval@t24.r02.wrong\endcsname{4.7}
\expandafter\def\csname BAval@t24.r02.recovery\endcsname{85.8}
\expandafter\def\csname BAval@t24.r02.t5\endcsname{1.4}
\expandafter\def\csname BAval@t24.r03.sid\endcsname{82.3}
\expandafter\def\csname BAval@t24.r03.wrong\endcsname{4.4}
\expandafter\def\csname BAval@t24.r03.recovery\endcsname{86.2}
\expandafter\def\csname BAval@t24.r03.t5\endcsname{1.4}
\expandafter\def\csname BAval@t24.r04.sid\endcsname{82.1}
\expandafter\def\csname BAval@t24.r04.wrong\endcsname{4.2}
\expandafter\def\csname BAval@t24.r04.recovery\endcsname{85.8}
\expandafter\def\csname BAval@t24.r04.t5\endcsname{1.4}
\expandafter\def\csname BAval@t25.r01.value\endcsname{1.00}
\expandafter\def\csname BAval@t25.r02.value\endcsname{0.50}
\expandafter\def\csname BAval@t25.r03.value\endcsname{0.10}
\expandafter\def\csname BAval@t25.r04.value\endcsname{1.00}
\expandafter\def\csname BAval@t25.r05.value\endcsname{0.20}
\expandafter\def\csname BAval@t25.r06.value\endcsname{0.01}
\expandafter\def\csname BAval@t25.r07.value\endcsname{0.01}
\expandafter\def\csname BAval@t25.r08.value\endcsname{0.05}
\expandafter\def\csname BAval@t26.r01.decisions\endcsname{17}
\expandafter\def\csname BAval@t26.r01.completed\endcsname{16}
\expandafter\def\csname BAval@t26.r01.timeouts\endcsname{1}
\expandafter\def\csname BAval@t26.r01.completion.pct\endcsname{94.1}
\expandafter\def\csname BAval@t26.r01.fallback.pct\endcsname{5.9}
\expandafter\def\csname BAval@t26.r02.decisions\endcsname{12}
\expandafter\def\csname BAval@t26.r02.completed\endcsname{11}
\expandafter\def\csname BAval@t26.r02.timeouts\endcsname{1}
\expandafter\def\csname BAval@t26.r02.completion.pct\endcsname{91.7}
\expandafter\def\csname BAval@t26.r02.fallback.pct\endcsname{8.3}
\expandafter\def\csname BAval@t27.r01.total.s\endcsname{9.00}
\expandafter\def\csname BAval@t27.r01.correct.s\endcsname{7.40}
\expandafter\def\csname BAval@t27.r01.wrong.s\endcsname{0.22}
\expandafter\def\csname BAval@t27.r01.sid\endcsname{82.3}
\expandafter\def\csname BAval@t27.r01.wrong\endcsname{2.4}
\expandafter\def\csname BAval@t27.r02.total.s\endcsname{9.00}
\expandafter\def\csname BAval@t27.r02.correct.s\endcsname{7.06}
\expandafter\def\csname BAval@t27.r02.wrong.s\endcsname{0.36}
\expandafter\def\csname BAval@t27.r02.sid\endcsname{78.5}
\expandafter\def\csname BAval@t27.r02.wrong\endcsname{4.0}
\expandafter\def\csname BAval@ext.best.sid\endcsname{75.2}
\expandafter\def\csname BAval@ext.best.wrong\endcsname{7.3}
\expandafter\def\csname BAval@ext.best.recovery\endcsname{79.0}
\expandafter\def\csname BAval@ext.best.t5\endcsname{2.0}
\expandafter\def\csname BAval@ext.bind.sid\endcsname{82.3}
\expandafter\def\csname BAval@ext.bind.wrong\endcsname{4.4}
\expandafter\def\csname BAval@ext.bind.recovery\endcsname{86.2}
\expandafter\def\csname BAval@ext.bind.t5\endcsname{1.4}
\expandafter\def\csname BAval@ext.joint.sid\endcsname{74.6}
\expandafter\def\csname BAval@ext.joint.wrong\endcsname{6.9}
\expandafter\def\csname BAval@ext.joint.recovery\endcsname{77.9}
\expandafter\def\csname BAval@ext.joint.t5\endcsname{2.0}
\expandafter\def\csname BAval@ext.dam.sid\endcsname{70.3}
\expandafter\def\csname BAval@ext.dam.wrong\endcsname{8.1}
\expandafter\def\csname BAval@ext.dam.recovery\endcsname{74.0}
\expandafter\def\csname BAval@ext.dam.t5\endcsname{2.2}
\expandafter\def\csname BAval@int.joint.sid\endcsname{70.3}
\expandafter\def\csname BAval@int.joint.wrong\endcsname{8.8}
\expandafter\def\csname BAval@int.joint.recovery\endcsname{72.0}
\expandafter\def\csname BAval@int.joint.t5\endcsname{2.4}
\expandafter\def\csname BAval@int.bind.sid\endcsname{82.3}
\expandafter\def\csname BAval@int.bind.wrong\endcsname{4.4}
\expandafter\def\csname BAval@int.bind.recovery\endcsname{86.2}
\expandafter\def\csname BAval@int.bind.t5\endcsname{1.4}
\expandafter\def\csname BAval@int.oracle.sid\endcsname{87.9}
\expandafter\def\csname BAval@int.oracle.wrong\endcsname{1.6}
\expandafter\def\csname BAval@int.oracle.recovery\endcsname{92.0}
\expandafter\def\csname BAval@int.oracle.t5\endcsname{1.2}
\expandafter\def\csname BAval@int.temporal.sid\endcsname{68.7}
\expandafter\def\csname BAval@int.temporal.wrong\endcsname{10.1}
\expandafter\def\csname BAval@int.temporal.recovery\endcsname{70.0}
\expandafter\def\csname BAval@int.temporal.t5\endcsname{2.5}
\expandafter\def\csname BAval@budget.bind075.sid\endcsname{77.1}
\expandafter\def\csname BAval@budget.joint075.sid\endcsname{64.0}
\expandafter\def\csname BAval@budget.joint100.sid\endcsname{70.3}
\expandafter\def\csname BAval@swap.refsep\endcsname{65.9}
\expandafter\def\csname BAval@swap.refjoint\endcsname{70.3}
\expandafter\def\csname BAval@swap.bindsep\endcsname{77.6}
\expandafter\def\csname BAval@swap.bindjoint\endcsname{82.3}
\expandafter\def\csname BAval@delta.ext.sid\endcsname{7.1}
\expandafter\def\csname BAval@delta.swap.refplanner\endcsname{4.4}
\expandafter\def\csname BAval@delta.swap.bindplanner\endcsname{4.7}
\expandafter\def\csname BAval@delta.swap.sepresponse\endcsname{11.8}
\expandafter\def\csname BAval@delta.swap.jointresponse\endcsname{12.0}
\expandafter\def\csname BAval@delta.ext.wrong\endcsname{2.9}
\expandafter\def\csname BAval@delta.ext.recovery\endcsname{7.2}
\expandafter\def\csname BAval@delta.swap.interaction\endcsname{0.2}
\expandafter\def\csname BAval@gap.remaining\endcsname{5.6}
\expandafter\def\csname BAval@gap.external\endcsname{55.7}
\expandafter\def\csname BAval@gap.internal\endcsname{68.1}
\expandafter\def\csname BAval@delta.ext.wrong.relative\endcsname{39.2}
\expandafter\def\csname BAval@delta.ext.t5\endcsname{0.6}
\expandafter\def\csname BAval@sweep.zero.bind\endcsname{86.1}
\expandafter\def\csname BAval@sweep.zero.best\endcsname{82.0}
\expandafter\def\csname BAval@delta.sweep.zero\endcsname{4.1}
\expandafter\def\csname BAval@sweep.ref.bind\endcsname{82.3}
\expandafter\def\csname BAval@sweep.ref.best\endcsname{75.2}
\expandafter\def\csname BAval@delta.sweep.ref\endcsname{7.1}
\expandafter\def\csname BAval@sweep.two.bind\endcsname{64.0}
\expandafter\def\csname BAval@sweep.two.best\endcsname{51.9}
\expandafter\def\csname BAval@delta.sweep.two\endcsname{12.2}
\expandafter\def\csname BAval@sweep.cap075.bind\endcsname{77.1}
\expandafter\def\csname BAval@sweep.cap075.best\endcsname{69.5}
\expandafter\def\csname BAval@delta.sweep.cap075\endcsname{7.6}
\expandafter\def\csname BAval@sweep.cap200.bind\endcsname{86.2}
\expandafter\def\csname BAval@sweep.cap200.best\endcsname{80.8}
\expandafter\def\csname BAval@delta.sweep.cap200\endcsname{5.4}
\expandafter\def\csname BAval@strata.bind.short\endcsname{90.2}
\expandafter\def\csname BAval@strata.best.short\endcsname{86.2}
\expandafter\def\csname BAval@delta.strata.short\endcsname{4.1}
\expandafter\def\csname BAval@strata.bind.similar\endcsname{85.4}
\expandafter\def\csname BAval@strata.best.similar\endcsname{79.2}
\expandafter\def\csname BAval@delta.strata.similar\endcsname{6.2}
\expandafter\def\csname BAval@strata.bind.long\endcsname{73.9}
\expandafter\def\csname BAval@strata.best.long\endcsname{63.9}
\expandafter\def\csname BAval@delta.strata.long\endcsname{10.0}
\expandafter\def\csname BAval@delta.backbone.ost\endcsname{8.3}
\expandafter\def\csname BAval@delta.backbone.lorat\endcsname{7.6}
\expandafter\def\csname BAval@delta.backbone.dam\endcsname{7.1}
\expandafter\def\csname BAval@runtime.best.mean\endcsname{37.8}
\expandafter\def\csname BAval@runtime.best.p95\endcsname{52.2}
\expandafter\def\csname BAval@runtime.best.fps\endcsname{26.4}
\expandafter\def\csname BAval@runtime.best.decision\endcsname{1.8}
\expandafter\def\csname BAval@runtime.bind.mean\endcsname{37.4}
\expandafter\def\csname BAval@runtime.bind.p95\endcsname{51.7}
\expandafter\def\csname BAval@runtime.bind.fps\endcsname{26.8}
\expandafter\def\csname BAval@runtime.bind.decision\endcsname{2.1}
\expandafter\def\csname BAval@lt.best.fmax\endcsname{78.9}
\expandafter\def\csname BAval@lt.bind.fmax\endcsname{85.0}
\expandafter\def\csname BAval@car.bind\endcsname{94.0}
\expandafter\def\csname BAval@car.oa\endcsname{95.0}
\expandafter\def\csname BAval@fixed.bind.ao\endcsname{79.1}
\expandafter\def\csname BAval@fixed.lorat.ao\endcsname{72.7}
\expandafter\def\csname BAval@fixed.dam.ao\endcsname{73.3}
\expandafter\def\csname BAval@delta.fixed.lorat.ao\endcsname{6.3}
\expandafter\def\csname BAval@delta.fixed.dam.ao\endcsname{5.8}
\expandafter\def\csname BAval@fixed.bind.sao\endcsname{76.9}
\expandafter\def\csname BAval@fixed.lorat.sao\endcsname{67.0}
\expandafter\def\csname BAval@fixed.dam.sao\endcsname{66.7}
\expandafter\def\csname BAval@delta.fixed.lorat.sao\endcsname{10.0}
\expandafter\def\csname BAval@delta.fixed.dam.sao\endcsname{10.3}
\expandafter\def\csname BAval@rec.quad.attempts\endcsname{17}
\expandafter\def\csname BAval@rec.quad.complete\endcsname{0}
\expandafter\def\csname BAval@rec.quad.fallwait\endcsname{16}
\expandafter\def\csname BAval@rec.quad.expired\endcsname{1}
\expandafter\def\csname BAval@rec.quad.requests\endcsname{0}
\expandafter\def\csname BAval@rec.quad.returns\endcsname{0}
\expandafter\def\csname BAval@rec.quad.initialpub\endcsname{1}
\expandafter\def\csname BAval@rec.quad.laterpub\endcsname{0}
\expandafter\def\csname BAval@rec.quad.nativeupdates\endcsname{0}
\expandafter\def\csname BAval@rec.quad.ticks\endcsname{90}
\expandafter\def\csname BAval@state.quad.dam.correct\endcsname{1}
\expandafter\def\csname BAval@state.quad.dam.wrong\endcsname{10}
\expandafter\def\csname BAval@state.quad.dam.unresolved\endcsname{61}
\expandafter\def\csname BAval@state.quad.dam.unknown\endcsname{18}
\expandafter\def\csname BAval@tick.quad.f409.dam.iou\endcsname{0.58}
\expandafter\def\csname BAval@tick.quad.f409.dam.state\endcsname{C}
\expandafter\def\csname BAval@tick.quad.f410.dam.iou\endcsname{0.36}
\expandafter\def\csname BAval@tick.quad.f410.dam.state\endcsname{U}
\expandafter\def\csname BAval@tick.quad.f411.dam.iou\endcsname{0.27}
\expandafter\def\csname BAval@tick.quad.f411.dam.state\endcsname{U}
\expandafter\def\csname BAval@tick.quad.f412.dam.iou\endcsname{0.10}
\expandafter\def\csname BAval@tick.quad.f412.dam.state\endcsname{U}
\expandafter\def\csname BAval@tick.quad.f413.dam.iou\endcsname{0.00}
\expandafter\def\csname BAval@tick.quad.f413.dam.state\endcsname{U}
\expandafter\def\csname BAval@tick.quad.f414.dam.iou\endcsname{0.00}
\expandafter\def\csname BAval@tick.quad.f414.dam.state\endcsname{U}
\expandafter\def\csname BAval@tick.quad.f415.dam.iou\endcsname{0.00}
\expandafter\def\csname BAval@tick.quad.f415.dam.state\endcsname{U}
\expandafter\def\csname BAval@tick.quad.f416.dam.iou\endcsname{0.00}
\expandafter\def\csname BAval@tick.quad.f416.dam.state\endcsname{U}
\expandafter\def\csname BAval@tick.quad.f417.dam.iou\endcsname{0.00}
\expandafter\def\csname BAval@tick.quad.f417.dam.state\endcsname{U}
\expandafter\def\csname BAval@tick.quad.f418.dam.iou\endcsname{0.00}
\expandafter\def\csname BAval@tick.quad.f418.dam.state\endcsname{U}
\expandafter\def\csname BAval@tick.quad.f419.dam.iou\endcsname{0.00}
\expandafter\def\csname BAval@tick.quad.f419.dam.state\endcsname{U}
\expandafter\def\csname BAval@tick.quad.f420.dam.iou\endcsname{0.00}
\expandafter\def\csname BAval@tick.quad.f420.dam.state\endcsname{W}
\expandafter\def\csname BAval@tick.quad.f421.dam.iou\endcsname{0.00}
\expandafter\def\csname BAval@tick.quad.f421.dam.state\endcsname{U}
\expandafter\def\csname BAval@tick.quad.f422.dam.iou\endcsname{0.00}
\expandafter\def\csname BAval@tick.quad.f422.dam.state\endcsname{U}
\expandafter\def\csname BAval@tick.quad.f423.dam.iou\endcsname{0.00}
\expandafter\def\csname BAval@tick.quad.f423.dam.state\endcsname{U}
\expandafter\def\csname BAval@tick.quad.f424.dam.iou\endcsname{0.00}
\expandafter\def\csname BAval@tick.quad.f424.dam.state\endcsname{U}
\expandafter\def\csname BAval@tick.quad.f425.dam.iou\endcsname{0.00}
\expandafter\def\csname BAval@tick.quad.f425.dam.state\endcsname{W}
\expandafter\def\csname BAval@tick.quad.f426.dam.iou\endcsname{0.00}
\expandafter\def\csname BAval@tick.quad.f426.dam.state\endcsname{W}
\expandafter\def\csname BAval@tick.quad.f427.dam.iou\endcsname{0.00}
\expandafter\def\csname BAval@tick.quad.f427.dam.state\endcsname{W}
\expandafter\def\csname BAval@tick.quad.f428.dam.iou\endcsname{0.00}
\expandafter\def\csname BAval@tick.quad.f428.dam.state\endcsname{U}
\expandafter\def\csname BAval@tick.quad.f429.dam.iou\endcsname{0.00}
\expandafter\def\csname BAval@tick.quad.f429.dam.state\endcsname{U}
\expandafter\def\csname BAval@tick.quad.f430.dam.iou\endcsname{0.00}
\expandafter\def\csname BAval@tick.quad.f430.dam.state\endcsname{U}
\expandafter\def\csname BAval@tick.quad.f431.dam.iou\endcsname{0.00}
\expandafter\def\csname BAval@tick.quad.f431.dam.state\endcsname{U}
\expandafter\def\csname BAval@tick.quad.f432.dam.iou\endcsname{0.00}
\expandafter\def\csname BAval@tick.quad.f432.dam.state\endcsname{U}
\expandafter\def\csname BAval@tick.quad.f433.dam.iou\endcsname{0.00}
\expandafter\def\csname BAval@tick.quad.f433.dam.state\endcsname{U}
\expandafter\def\csname BAval@tick.quad.f434.dam.iou\endcsname{0.00}
\expandafter\def\csname BAval@tick.quad.f434.dam.state\endcsname{U}
\expandafter\def\csname BAval@tick.quad.f435.dam.iou\endcsname{0.00}
\expandafter\def\csname BAval@tick.quad.f435.dam.state\endcsname{U}
\expandafter\def\csname BAval@tick.quad.f436.dam.iou\endcsname{0.00}
\expandafter\def\csname BAval@tick.quad.f436.dam.state\endcsname{UNKNOWN}
\expandafter\def\csname BAval@tick.quad.f437.dam.iou\endcsname{0.00}
\expandafter\def\csname BAval@tick.quad.f437.dam.state\endcsname{UNKNOWN}
\expandafter\def\csname BAval@tick.quad.f438.dam.iou\endcsname{0.00}
\expandafter\def\csname BAval@tick.quad.f438.dam.state\endcsname{UNKNOWN}
\expandafter\def\csname BAval@tick.quad.f439.dam.iou\endcsname{0.00}
\expandafter\def\csname BAval@tick.quad.f439.dam.state\endcsname{UNKNOWN}
\expandafter\def\csname BAval@tick.quad.f440.dam.iou\endcsname{0.00}
\expandafter\def\csname BAval@tick.quad.f440.dam.state\endcsname{UNKNOWN}
\expandafter\def\csname BAval@tick.quad.f441.dam.iou\endcsname{0.00}
\expandafter\def\csname BAval@tick.quad.f441.dam.state\endcsname{W}
\expandafter\def\csname BAval@tick.quad.f442.dam.iou\endcsname{0.00}
\expandafter\def\csname BAval@tick.quad.f442.dam.state\endcsname{W}
\expandafter\def\csname BAval@tick.quad.f443.dam.iou\endcsname{0.00}
\expandafter\def\csname BAval@tick.quad.f443.dam.state\endcsname{W}
\expandafter\def\csname BAval@tick.quad.f444.dam.iou\endcsname{0.00}
\expandafter\def\csname BAval@tick.quad.f444.dam.state\endcsname{U}
\expandafter\def\csname BAval@tick.quad.f445.dam.iou\endcsname{0.00}
\expandafter\def\csname BAval@tick.quad.f445.dam.state\endcsname{U}
\expandafter\def\csname BAval@tick.quad.f446.dam.iou\endcsname{0.00}
\expandafter\def\csname BAval@tick.quad.f446.dam.state\endcsname{U}
\expandafter\def\csname BAval@tick.quad.f447.dam.iou\endcsname{0.00}
\expandafter\def\csname BAval@tick.quad.f447.dam.state\endcsname{U}
\expandafter\def\csname BAval@tick.quad.f448.dam.iou\endcsname{0.00}
\expandafter\def\csname BAval@tick.quad.f448.dam.state\endcsname{U}
\expandafter\def\csname BAval@tick.quad.f449.dam.iou\endcsname{0.00}
\expandafter\def\csname BAval@tick.quad.f449.dam.state\endcsname{U}
\expandafter\def\csname BAval@tick.quad.f450.dam.iou\endcsname{0.00}
\expandafter\def\csname BAval@tick.quad.f450.dam.state\endcsname{U}
\expandafter\def\csname BAval@tick.quad.f451.dam.iou\endcsname{0.00}
\expandafter\def\csname BAval@tick.quad.f451.dam.state\endcsname{U}
\expandafter\def\csname BAval@tick.quad.f452.dam.iou\endcsname{0.00}
\expandafter\def\csname BAval@tick.quad.f452.dam.state\endcsname{U}
\expandafter\def\csname BAval@tick.quad.f453.dam.iou\endcsname{0.00}
\expandafter\def\csname BAval@tick.quad.f453.dam.state\endcsname{U}
\expandafter\def\csname BAval@tick.quad.f454.dam.iou\endcsname{0.00}
\expandafter\def\csname BAval@tick.quad.f454.dam.state\endcsname{UNKNOWN}
\expandafter\def\csname BAval@tick.quad.f455.dam.iou\endcsname{0.00}
\expandafter\def\csname BAval@tick.quad.f455.dam.state\endcsname{UNKNOWN}
\expandafter\def\csname BAval@tick.quad.f456.dam.iou\endcsname{0.00}
\expandafter\def\csname BAval@tick.quad.f456.dam.state\endcsname{UNKNOWN}
\expandafter\def\csname BAval@tick.quad.f457.dam.iou\endcsname{0.00}
\expandafter\def\csname BAval@tick.quad.f457.dam.state\endcsname{U}
\expandafter\def\csname BAval@tick.quad.f458.dam.iou\endcsname{0.00}
\expandafter\def\csname BAval@tick.quad.f458.dam.state\endcsname{U}
\expandafter\def\csname BAval@tick.quad.f459.dam.iou\endcsname{0.00}
\expandafter\def\csname BAval@tick.quad.f459.dam.state\endcsname{U}
\expandafter\def\csname BAval@tick.quad.f460.dam.iou\endcsname{0.00}
\expandafter\def\csname BAval@tick.quad.f460.dam.state\endcsname{U}
\expandafter\def\csname BAval@tick.quad.f461.dam.iou\endcsname{0.00}
\expandafter\def\csname BAval@tick.quad.f461.dam.state\endcsname{U}
\expandafter\def\csname BAval@tick.quad.f462.dam.iou\endcsname{0.00}
\expandafter\def\csname BAval@tick.quad.f462.dam.state\endcsname{U}
\expandafter\def\csname BAval@tick.quad.f463.dam.iou\endcsname{0.00}
\expandafter\def\csname BAval@tick.quad.f463.dam.state\endcsname{U}
\expandafter\def\csname BAval@tick.quad.f464.dam.iou\endcsname{0.00}
\expandafter\def\csname BAval@tick.quad.f464.dam.state\endcsname{U}
\expandafter\def\csname BAval@tick.quad.f465.dam.iou\endcsname{0.00}
\expandafter\def\csname BAval@tick.quad.f465.dam.state\endcsname{U}
\expandafter\def\csname BAval@tick.quad.f466.dam.iou\endcsname{0.00}
\expandafter\def\csname BAval@tick.quad.f466.dam.state\endcsname{U}
\expandafter\def\csname BAval@tick.quad.f467.dam.iou\endcsname{0.00}
\expandafter\def\csname BAval@tick.quad.f467.dam.state\endcsname{U}
\expandafter\def\csname BAval@tick.quad.f468.dam.iou\endcsname{0.00}
\expandafter\def\csname BAval@tick.quad.f468.dam.state\endcsname{U}
\expandafter\def\csname BAval@tick.quad.f469.dam.iou\endcsname{0.00}
\expandafter\def\csname BAval@tick.quad.f469.dam.state\endcsname{U}
\expandafter\def\csname BAval@tick.quad.f470.dam.iou\endcsname{0.00}
\expandafter\def\csname BAval@tick.quad.f470.dam.state\endcsname{U}
\expandafter\def\csname BAval@tick.quad.f471.dam.iou\endcsname{0.00}
\expandafter\def\csname BAval@tick.quad.f471.dam.state\endcsname{U}
\expandafter\def\csname BAval@tick.quad.f472.dam.iou\endcsname{0.00}
\expandafter\def\csname BAval@tick.quad.f472.dam.state\endcsname{U}
\expandafter\def\csname BAval@tick.quad.f473.dam.iou\endcsname{0.00}
\expandafter\def\csname BAval@tick.quad.f473.dam.state\endcsname{UNKNOWN}
\expandafter\def\csname BAval@tick.quad.f474.dam.iou\endcsname{0.00}
\expandafter\def\csname BAval@tick.quad.f474.dam.state\endcsname{UNKNOWN}
\expandafter\def\csname BAval@tick.quad.f475.dam.iou\endcsname{0.00}
\expandafter\def\csname BAval@tick.quad.f475.dam.state\endcsname{UNKNOWN}
\expandafter\def\csname BAval@tick.quad.f476.dam.iou\endcsname{0.00}
\expandafter\def\csname BAval@tick.quad.f476.dam.state\endcsname{UNKNOWN}
\expandafter\def\csname BAval@tick.quad.f477.dam.iou\endcsname{0.00}
\expandafter\def\csname BAval@tick.quad.f477.dam.state\endcsname{U}
\expandafter\def\csname BAval@tick.quad.f478.dam.iou\endcsname{0.00}
\expandafter\def\csname BAval@tick.quad.f478.dam.state\endcsname{U}
\expandafter\def\csname BAval@tick.quad.f479.dam.iou\endcsname{0.00}
\expandafter\def\csname BAval@tick.quad.f479.dam.state\endcsname{U}
\expandafter\def\csname BAval@tick.quad.f480.dam.iou\endcsname{0.00}
\expandafter\def\csname BAval@tick.quad.f480.dam.state\endcsname{U}
\expandafter\def\csname BAval@tick.quad.f481.dam.iou\endcsname{0.00}
\expandafter\def\csname BAval@tick.quad.f481.dam.state\endcsname{U}
\expandafter\def\csname BAval@tick.quad.f482.dam.iou\endcsname{0.00}
\expandafter\def\csname BAval@tick.quad.f482.dam.state\endcsname{U}
\expandafter\def\csname BAval@tick.quad.f483.dam.iou\endcsname{0.00}
\expandafter\def\csname BAval@tick.quad.f483.dam.state\endcsname{U}
\expandafter\def\csname BAval@tick.quad.f484.dam.iou\endcsname{0.00}
\expandafter\def\csname BAval@tick.quad.f484.dam.state\endcsname{U}
\expandafter\def\csname BAval@tick.quad.f485.dam.iou\endcsname{0.00}
\expandafter\def\csname BAval@tick.quad.f485.dam.state\endcsname{W}
\expandafter\def\csname BAval@tick.quad.f486.dam.iou\endcsname{0.00}
\expandafter\def\csname BAval@tick.quad.f486.dam.state\endcsname{W}
\expandafter\def\csname BAval@tick.quad.f487.dam.iou\endcsname{0.00}
\expandafter\def\csname BAval@tick.quad.f487.dam.state\endcsname{W}
\expandafter\def\csname BAval@tick.quad.f488.dam.iou\endcsname{0.00}
\expandafter\def\csname BAval@tick.quad.f488.dam.state\endcsname{U}
\expandafter\def\csname BAval@tick.quad.f489.dam.iou\endcsname{0.00}
\expandafter\def\csname BAval@tick.quad.f489.dam.state\endcsname{U}
\expandafter\def\csname BAval@tick.quad.f490.dam.iou\endcsname{0.00}
\expandafter\def\csname BAval@tick.quad.f490.dam.state\endcsname{U}
\expandafter\def\csname BAval@tick.quad.f491.dam.iou\endcsname{0.00}
\expandafter\def\csname BAval@tick.quad.f491.dam.state\endcsname{U}
\expandafter\def\csname BAval@tick.quad.f492.dam.iou\endcsname{0.00}
\expandafter\def\csname BAval@tick.quad.f492.dam.state\endcsname{U}
\expandafter\def\csname BAval@tick.quad.f493.dam.iou\endcsname{0.00}
\expandafter\def\csname BAval@tick.quad.f493.dam.state\endcsname{UNKNOWN}
\expandafter\def\csname BAval@tick.quad.f494.dam.iou\endcsname{0.00}
\expandafter\def\csname BAval@tick.quad.f494.dam.state\endcsname{UNKNOWN}
\expandafter\def\csname BAval@tick.quad.f495.dam.iou\endcsname{0.00}
\expandafter\def\csname BAval@tick.quad.f495.dam.state\endcsname{UNKNOWN}
\expandafter\def\csname BAval@tick.quad.f496.dam.iou\endcsname{0.00}
\expandafter\def\csname BAval@tick.quad.f496.dam.state\endcsname{UNKNOWN}
\expandafter\def\csname BAval@tick.quad.f497.dam.iou\endcsname{0.00}
\expandafter\def\csname BAval@tick.quad.f497.dam.state\endcsname{UNKNOWN}
\expandafter\def\csname BAval@tick.quad.f498.dam.iou\endcsname{0.00}
\expandafter\def\csname BAval@tick.quad.f498.dam.state\endcsname{UNKNOWN}
\expandafter\def\csname BAval@state.quad.keep.correct\endcsname{1}
\expandafter\def\csname BAval@state.quad.keep.wrong\endcsname{12}
\expandafter\def\csname BAval@state.quad.keep.unresolved\endcsname{59}
\expandafter\def\csname BAval@state.quad.keep.unknown\endcsname{18}
\expandafter\def\csname BAval@tick.quad.f409.keep.iou\endcsname{0.58}
\expandafter\def\csname BAval@tick.quad.f409.keep.state\endcsname{C}
\expandafter\def\csname BAval@tick.quad.f410.keep.iou\endcsname{0.36}
\expandafter\def\csname BAval@tick.quad.f410.keep.state\endcsname{U}
\expandafter\def\csname BAval@tick.quad.f411.keep.iou\endcsname{0.27}
\expandafter\def\csname BAval@tick.quad.f411.keep.state\endcsname{U}
\expandafter\def\csname BAval@tick.quad.f412.keep.iou\endcsname{0.10}
\expandafter\def\csname BAval@tick.quad.f412.keep.state\endcsname{U}
\expandafter\def\csname BAval@tick.quad.f413.keep.iou\endcsname{0.00}
\expandafter\def\csname BAval@tick.quad.f413.keep.state\endcsname{U}
\expandafter\def\csname BAval@tick.quad.f414.keep.iou\endcsname{0.00}
\expandafter\def\csname BAval@tick.quad.f414.keep.state\endcsname{U}
\expandafter\def\csname BAval@tick.quad.f415.keep.iou\endcsname{0.00}
\expandafter\def\csname BAval@tick.quad.f415.keep.state\endcsname{U}
\expandafter\def\csname BAval@tick.quad.f416.keep.iou\endcsname{0.00}
\expandafter\def\csname BAval@tick.quad.f416.keep.state\endcsname{U}
\expandafter\def\csname BAval@tick.quad.f417.keep.iou\endcsname{0.00}
\expandafter\def\csname BAval@tick.quad.f417.keep.state\endcsname{U}
\expandafter\def\csname BAval@tick.quad.f418.keep.iou\endcsname{0.00}
\expandafter\def\csname BAval@tick.quad.f418.keep.state\endcsname{U}
\expandafter\def\csname BAval@tick.quad.f419.keep.iou\endcsname{0.00}
\expandafter\def\csname BAval@tick.quad.f419.keep.state\endcsname{U}
\expandafter\def\csname BAval@tick.quad.f420.keep.iou\endcsname{0.00}
\expandafter\def\csname BAval@tick.quad.f420.keep.state\endcsname{W}
\expandafter\def\csname BAval@tick.quad.f421.keep.iou\endcsname{0.00}
\expandafter\def\csname BAval@tick.quad.f421.keep.state\endcsname{U}
\expandafter\def\csname BAval@tick.quad.f422.keep.iou\endcsname{0.00}
\expandafter\def\csname BAval@tick.quad.f422.keep.state\endcsname{U}
\expandafter\def\csname BAval@tick.quad.f423.keep.iou\endcsname{0.00}
\expandafter\def\csname BAval@tick.quad.f423.keep.state\endcsname{U}
\expandafter\def\csname BAval@tick.quad.f424.keep.iou\endcsname{0.00}
\expandafter\def\csname BAval@tick.quad.f424.keep.state\endcsname{U}
\expandafter\def\csname BAval@tick.quad.f425.keep.iou\endcsname{0.00}
\expandafter\def\csname BAval@tick.quad.f425.keep.state\endcsname{W}
\expandafter\def\csname BAval@tick.quad.f426.keep.iou\endcsname{0.00}
\expandafter\def\csname BAval@tick.quad.f426.keep.state\endcsname{W}
\expandafter\def\csname BAval@tick.quad.f427.keep.iou\endcsname{0.00}
\expandafter\def\csname BAval@tick.quad.f427.keep.state\endcsname{W}
\expandafter\def\csname BAval@tick.quad.f428.keep.iou\endcsname{0.00}
\expandafter\def\csname BAval@tick.quad.f428.keep.state\endcsname{U}
\expandafter\def\csname BAval@tick.quad.f429.keep.iou\endcsname{0.00}
\expandafter\def\csname BAval@tick.quad.f429.keep.state\endcsname{U}
\expandafter\def\csname BAval@tick.quad.f430.keep.iou\endcsname{0.00}
\expandafter\def\csname BAval@tick.quad.f430.keep.state\endcsname{U}
\expandafter\def\csname BAval@tick.quad.f431.keep.iou\endcsname{0.00}
\expandafter\def\csname BAval@tick.quad.f431.keep.state\endcsname{U}
\expandafter\def\csname BAval@tick.quad.f432.keep.iou\endcsname{0.00}
\expandafter\def\csname BAval@tick.quad.f432.keep.state\endcsname{U}
\expandafter\def\csname BAval@tick.quad.f433.keep.iou\endcsname{0.00}
\expandafter\def\csname BAval@tick.quad.f433.keep.state\endcsname{U}
\expandafter\def\csname BAval@tick.quad.f434.keep.iou\endcsname{0.00}
\expandafter\def\csname BAval@tick.quad.f434.keep.state\endcsname{U}
\expandafter\def\csname BAval@tick.quad.f435.keep.iou\endcsname{0.00}
\expandafter\def\csname BAval@tick.quad.f435.keep.state\endcsname{U}
\expandafter\def\csname BAval@tick.quad.f436.keep.iou\endcsname{0.00}
\expandafter\def\csname BAval@tick.quad.f436.keep.state\endcsname{UNKNOWN}
\expandafter\def\csname BAval@tick.quad.f437.keep.iou\endcsname{0.00}
\expandafter\def\csname BAval@tick.quad.f437.keep.state\endcsname{UNKNOWN}
\expandafter\def\csname BAval@tick.quad.f438.keep.iou\endcsname{0.00}
\expandafter\def\csname BAval@tick.quad.f438.keep.state\endcsname{UNKNOWN}
\expandafter\def\csname BAval@tick.quad.f439.keep.iou\endcsname{0.00}
\expandafter\def\csname BAval@tick.quad.f439.keep.state\endcsname{UNKNOWN}
\expandafter\def\csname BAval@tick.quad.f440.keep.iou\endcsname{0.00}
\expandafter\def\csname BAval@tick.quad.f440.keep.state\endcsname{UNKNOWN}
\expandafter\def\csname BAval@tick.quad.f441.keep.iou\endcsname{0.00}
\expandafter\def\csname BAval@tick.quad.f441.keep.state\endcsname{W}
\expandafter\def\csname BAval@tick.quad.f442.keep.iou\endcsname{0.00}
\expandafter\def\csname BAval@tick.quad.f442.keep.state\endcsname{W}
\expandafter\def\csname BAval@tick.quad.f443.keep.iou\endcsname{0.00}
\expandafter\def\csname BAval@tick.quad.f443.keep.state\endcsname{W}
\expandafter\def\csname BAval@tick.quad.f444.keep.iou\endcsname{0.00}
\expandafter\def\csname BAval@tick.quad.f444.keep.state\endcsname{U}
\expandafter\def\csname BAval@tick.quad.f445.keep.iou\endcsname{0.00}
\expandafter\def\csname BAval@tick.quad.f445.keep.state\endcsname{U}
\expandafter\def\csname BAval@tick.quad.f446.keep.iou\endcsname{0.00}
\expandafter\def\csname BAval@tick.quad.f446.keep.state\endcsname{U}
\expandafter\def\csname BAval@tick.quad.f447.keep.iou\endcsname{0.00}
\expandafter\def\csname BAval@tick.quad.f447.keep.state\endcsname{U}
\expandafter\def\csname BAval@tick.quad.f448.keep.iou\endcsname{0.00}
\expandafter\def\csname BAval@tick.quad.f448.keep.state\endcsname{U}
\expandafter\def\csname BAval@tick.quad.f449.keep.iou\endcsname{0.00}
\expandafter\def\csname BAval@tick.quad.f449.keep.state\endcsname{U}
\expandafter\def\csname BAval@tick.quad.f450.keep.iou\endcsname{0.00}
\expandafter\def\csname BAval@tick.quad.f450.keep.state\endcsname{U}
\expandafter\def\csname BAval@tick.quad.f451.keep.iou\endcsname{0.00}
\expandafter\def\csname BAval@tick.quad.f451.keep.state\endcsname{U}
\expandafter\def\csname BAval@tick.quad.f452.keep.iou\endcsname{0.00}
\expandafter\def\csname BAval@tick.quad.f452.keep.state\endcsname{U}
\expandafter\def\csname BAval@tick.quad.f453.keep.iou\endcsname{0.00}
\expandafter\def\csname BAval@tick.quad.f453.keep.state\endcsname{U}
\expandafter\def\csname BAval@tick.quad.f454.keep.iou\endcsname{0.00}
\expandafter\def\csname BAval@tick.quad.f454.keep.state\endcsname{UNKNOWN}
\expandafter\def\csname BAval@tick.quad.f455.keep.iou\endcsname{0.00}
\expandafter\def\csname BAval@tick.quad.f455.keep.state\endcsname{UNKNOWN}
\expandafter\def\csname BAval@tick.quad.f456.keep.iou\endcsname{0.00}
\expandafter\def\csname BAval@tick.quad.f456.keep.state\endcsname{UNKNOWN}
\expandafter\def\csname BAval@tick.quad.f457.keep.iou\endcsname{0.00}
\expandafter\def\csname BAval@tick.quad.f457.keep.state\endcsname{W}
\expandafter\def\csname BAval@tick.quad.f458.keep.iou\endcsname{0.00}
\expandafter\def\csname BAval@tick.quad.f458.keep.state\endcsname{U}
\expandafter\def\csname BAval@tick.quad.f459.keep.iou\endcsname{0.00}
\expandafter\def\csname BAval@tick.quad.f459.keep.state\endcsname{U}
\expandafter\def\csname BAval@tick.quad.f460.keep.iou\endcsname{0.00}
\expandafter\def\csname BAval@tick.quad.f460.keep.state\endcsname{U}
\expandafter\def\csname BAval@tick.quad.f461.keep.iou\endcsname{0.00}
\expandafter\def\csname BAval@tick.quad.f461.keep.state\endcsname{U}
\expandafter\def\csname BAval@tick.quad.f462.keep.iou\endcsname{0.00}
\expandafter\def\csname BAval@tick.quad.f462.keep.state\endcsname{U}
\expandafter\def\csname BAval@tick.quad.f463.keep.iou\endcsname{0.00}
\expandafter\def\csname BAval@tick.quad.f463.keep.state\endcsname{U}
\expandafter\def\csname BAval@tick.quad.f464.keep.iou\endcsname{0.00}
\expandafter\def\csname BAval@tick.quad.f464.keep.state\endcsname{U}
\expandafter\def\csname BAval@tick.quad.f465.keep.iou\endcsname{0.00}
\expandafter\def\csname BAval@tick.quad.f465.keep.state\endcsname{U}
\expandafter\def\csname BAval@tick.quad.f466.keep.iou\endcsname{0.00}
\expandafter\def\csname BAval@tick.quad.f466.keep.state\endcsname{U}
\expandafter\def\csname BAval@tick.quad.f467.keep.iou\endcsname{0.00}
\expandafter\def\csname BAval@tick.quad.f467.keep.state\endcsname{U}
\expandafter\def\csname BAval@tick.quad.f468.keep.iou\endcsname{0.00}
\expandafter\def\csname BAval@tick.quad.f468.keep.state\endcsname{U}
\expandafter\def\csname BAval@tick.quad.f469.keep.iou\endcsname{0.00}
\expandafter\def\csname BAval@tick.quad.f469.keep.state\endcsname{U}
\expandafter\def\csname BAval@tick.quad.f470.keep.iou\endcsname{0.00}
\expandafter\def\csname BAval@tick.quad.f470.keep.state\endcsname{U}
\expandafter\def\csname BAval@tick.quad.f471.keep.iou\endcsname{0.00}
\expandafter\def\csname BAval@tick.quad.f471.keep.state\endcsname{U}
\expandafter\def\csname BAval@tick.quad.f472.keep.iou\endcsname{0.00}
\expandafter\def\csname BAval@tick.quad.f472.keep.state\endcsname{U}
\expandafter\def\csname BAval@tick.quad.f473.keep.iou\endcsname{0.00}
\expandafter\def\csname BAval@tick.quad.f473.keep.state\endcsname{UNKNOWN}
\expandafter\def\csname BAval@tick.quad.f474.keep.iou\endcsname{0.00}
\expandafter\def\csname BAval@tick.quad.f474.keep.state\endcsname{UNKNOWN}
\expandafter\def\csname BAval@tick.quad.f475.keep.iou\endcsname{0.00}
\expandafter\def\csname BAval@tick.quad.f475.keep.state\endcsname{UNKNOWN}
\expandafter\def\csname BAval@tick.quad.f476.keep.iou\endcsname{0.00}
\expandafter\def\csname BAval@tick.quad.f476.keep.state\endcsname{UNKNOWN}
\expandafter\def\csname BAval@tick.quad.f477.keep.iou\endcsname{0.00}
\expandafter\def\csname BAval@tick.quad.f477.keep.state\endcsname{U}
\expandafter\def\csname BAval@tick.quad.f478.keep.iou\endcsname{0.00}
\expandafter\def\csname BAval@tick.quad.f478.keep.state\endcsname{U}
\expandafter\def\csname BAval@tick.quad.f479.keep.iou\endcsname{0.00}
\expandafter\def\csname BAval@tick.quad.f479.keep.state\endcsname{U}
\expandafter\def\csname BAval@tick.quad.f480.keep.iou\endcsname{0.00}
\expandafter\def\csname BAval@tick.quad.f480.keep.state\endcsname{U}
\expandafter\def\csname BAval@tick.quad.f481.keep.iou\endcsname{0.00}
\expandafter\def\csname BAval@tick.quad.f481.keep.state\endcsname{U}
\expandafter\def\csname BAval@tick.quad.f482.keep.iou\endcsname{0.00}
\expandafter\def\csname BAval@tick.quad.f482.keep.state\endcsname{U}
\expandafter\def\csname BAval@tick.quad.f483.keep.iou\endcsname{0.00}
\expandafter\def\csname BAval@tick.quad.f483.keep.state\endcsname{U}
\expandafter\def\csname BAval@tick.quad.f484.keep.iou\endcsname{0.00}
\expandafter\def\csname BAval@tick.quad.f484.keep.state\endcsname{U}
\expandafter\def\csname BAval@tick.quad.f485.keep.iou\endcsname{0.00}
\expandafter\def\csname BAval@tick.quad.f485.keep.state\endcsname{U}
\expandafter\def\csname BAval@tick.quad.f486.keep.iou\endcsname{0.00}
\expandafter\def\csname BAval@tick.quad.f486.keep.state\endcsname{W}
\expandafter\def\csname BAval@tick.quad.f487.keep.iou\endcsname{0.00}
\expandafter\def\csname BAval@tick.quad.f487.keep.state\endcsname{W}
\expandafter\def\csname BAval@tick.quad.f488.keep.iou\endcsname{0.00}
\expandafter\def\csname BAval@tick.quad.f488.keep.state\endcsname{W}
\expandafter\def\csname BAval@tick.quad.f489.keep.iou\endcsname{0.00}
\expandafter\def\csname BAval@tick.quad.f489.keep.state\endcsname{W}
\expandafter\def\csname BAval@tick.quad.f490.keep.iou\endcsname{0.00}
\expandafter\def\csname BAval@tick.quad.f490.keep.state\endcsname{U}
\expandafter\def\csname BAval@tick.quad.f491.keep.iou\endcsname{0.00}
\expandafter\def\csname BAval@tick.quad.f491.keep.state\endcsname{U}
\expandafter\def\csname BAval@tick.quad.f492.keep.iou\endcsname{0.00}
\expandafter\def\csname BAval@tick.quad.f492.keep.state\endcsname{U}
\expandafter\def\csname BAval@tick.quad.f493.keep.iou\endcsname{0.00}
\expandafter\def\csname BAval@tick.quad.f493.keep.state\endcsname{UNKNOWN}
\expandafter\def\csname BAval@tick.quad.f494.keep.iou\endcsname{0.00}
\expandafter\def\csname BAval@tick.quad.f494.keep.state\endcsname{UNKNOWN}
\expandafter\def\csname BAval@tick.quad.f495.keep.iou\endcsname{0.00}
\expandafter\def\csname BAval@tick.quad.f495.keep.state\endcsname{UNKNOWN}
\expandafter\def\csname BAval@tick.quad.f496.keep.iou\endcsname{0.00}
\expandafter\def\csname BAval@tick.quad.f496.keep.state\endcsname{UNKNOWN}
\expandafter\def\csname BAval@tick.quad.f497.keep.iou\endcsname{0.00}
\expandafter\def\csname BAval@tick.quad.f497.keep.state\endcsname{UNKNOWN}
\expandafter\def\csname BAval@tick.quad.f498.keep.iou\endcsname{0.00}
\expandafter\def\csname BAval@tick.quad.f498.keep.state\endcsname{UNKNOWN}
\expandafter\def\csname BAval@state.quad.bind.correct\endcsname{1}
\expandafter\def\csname BAval@state.quad.bind.wrong\endcsname{12}
\expandafter\def\csname BAval@state.quad.bind.unresolved\endcsname{59}
\expandafter\def\csname BAval@state.quad.bind.unknown\endcsname{18}
\expandafter\def\csname BAval@tick.quad.f409.bind.iou\endcsname{0.58}
\expandafter\def\csname BAval@tick.quad.f409.bind.state\endcsname{C}
\expandafter\def\csname BAval@tick.quad.f410.bind.iou\endcsname{0.36}
\expandafter\def\csname BAval@tick.quad.f410.bind.state\endcsname{U}
\expandafter\def\csname BAval@tick.quad.f411.bind.iou\endcsname{0.27}
\expandafter\def\csname BAval@tick.quad.f411.bind.state\endcsname{U}
\expandafter\def\csname BAval@tick.quad.f412.bind.iou\endcsname{0.10}
\expandafter\def\csname BAval@tick.quad.f412.bind.state\endcsname{U}
\expandafter\def\csname BAval@tick.quad.f413.bind.iou\endcsname{0.00}
\expandafter\def\csname BAval@tick.quad.f413.bind.state\endcsname{U}
\expandafter\def\csname BAval@tick.quad.f414.bind.iou\endcsname{0.00}
\expandafter\def\csname BAval@tick.quad.f414.bind.state\endcsname{U}
\expandafter\def\csname BAval@tick.quad.f415.bind.iou\endcsname{0.00}
\expandafter\def\csname BAval@tick.quad.f415.bind.state\endcsname{U}
\expandafter\def\csname BAval@tick.quad.f416.bind.iou\endcsname{0.00}
\expandafter\def\csname BAval@tick.quad.f416.bind.state\endcsname{U}
\expandafter\def\csname BAval@tick.quad.f417.bind.iou\endcsname{0.00}
\expandafter\def\csname BAval@tick.quad.f417.bind.state\endcsname{U}
\expandafter\def\csname BAval@tick.quad.f418.bind.iou\endcsname{0.00}
\expandafter\def\csname BAval@tick.quad.f418.bind.state\endcsname{U}
\expandafter\def\csname BAval@tick.quad.f419.bind.iou\endcsname{0.00}
\expandafter\def\csname BAval@tick.quad.f419.bind.state\endcsname{U}
\expandafter\def\csname BAval@tick.quad.f420.bind.iou\endcsname{0.00}
\expandafter\def\csname BAval@tick.quad.f420.bind.state\endcsname{W}
\expandafter\def\csname BAval@tick.quad.f421.bind.iou\endcsname{0.00}
\expandafter\def\csname BAval@tick.quad.f421.bind.state\endcsname{U}
\expandafter\def\csname BAval@tick.quad.f422.bind.iou\endcsname{0.00}
\expandafter\def\csname BAval@tick.quad.f422.bind.state\endcsname{U}
\expandafter\def\csname BAval@tick.quad.f423.bind.iou\endcsname{0.00}
\expandafter\def\csname BAval@tick.quad.f423.bind.state\endcsname{U}
\expandafter\def\csname BAval@tick.quad.f424.bind.iou\endcsname{0.00}
\expandafter\def\csname BAval@tick.quad.f424.bind.state\endcsname{U}
\expandafter\def\csname BAval@tick.quad.f425.bind.iou\endcsname{0.00}
\expandafter\def\csname BAval@tick.quad.f425.bind.state\endcsname{W}
\expandafter\def\csname BAval@tick.quad.f426.bind.iou\endcsname{0.00}
\expandafter\def\csname BAval@tick.quad.f426.bind.state\endcsname{W}
\expandafter\def\csname BAval@tick.quad.f427.bind.iou\endcsname{0.00}
\expandafter\def\csname BAval@tick.quad.f427.bind.state\endcsname{W}
\expandafter\def\csname BAval@tick.quad.f428.bind.iou\endcsname{0.00}
\expandafter\def\csname BAval@tick.quad.f428.bind.state\endcsname{U}
\expandafter\def\csname BAval@tick.quad.f429.bind.iou\endcsname{0.00}
\expandafter\def\csname BAval@tick.quad.f429.bind.state\endcsname{U}
\expandafter\def\csname BAval@tick.quad.f430.bind.iou\endcsname{0.00}
\expandafter\def\csname BAval@tick.quad.f430.bind.state\endcsname{U}
\expandafter\def\csname BAval@tick.quad.f431.bind.iou\endcsname{0.00}
\expandafter\def\csname BAval@tick.quad.f431.bind.state\endcsname{U}
\expandafter\def\csname BAval@tick.quad.f432.bind.iou\endcsname{0.00}
\expandafter\def\csname BAval@tick.quad.f432.bind.state\endcsname{U}
\expandafter\def\csname BAval@tick.quad.f433.bind.iou\endcsname{0.00}
\expandafter\def\csname BAval@tick.quad.f433.bind.state\endcsname{U}
\expandafter\def\csname BAval@tick.quad.f434.bind.iou\endcsname{0.00}
\expandafter\def\csname BAval@tick.quad.f434.bind.state\endcsname{U}
\expandafter\def\csname BAval@tick.quad.f435.bind.iou\endcsname{0.00}
\expandafter\def\csname BAval@tick.quad.f435.bind.state\endcsname{U}
\expandafter\def\csname BAval@tick.quad.f436.bind.iou\endcsname{0.00}
\expandafter\def\csname BAval@tick.quad.f436.bind.state\endcsname{UNKNOWN}
\expandafter\def\csname BAval@tick.quad.f437.bind.iou\endcsname{0.00}
\expandafter\def\csname BAval@tick.quad.f437.bind.state\endcsname{UNKNOWN}
\expandafter\def\csname BAval@tick.quad.f438.bind.iou\endcsname{0.00}
\expandafter\def\csname BAval@tick.quad.f438.bind.state\endcsname{UNKNOWN}
\expandafter\def\csname BAval@tick.quad.f439.bind.iou\endcsname{0.00}
\expandafter\def\csname BAval@tick.quad.f439.bind.state\endcsname{UNKNOWN}
\expandafter\def\csname BAval@tick.quad.f440.bind.iou\endcsname{0.00}
\expandafter\def\csname BAval@tick.quad.f440.bind.state\endcsname{UNKNOWN}
\expandafter\def\csname BAval@tick.quad.f441.bind.iou\endcsname{0.00}
\expandafter\def\csname BAval@tick.quad.f441.bind.state\endcsname{W}
\expandafter\def\csname BAval@tick.quad.f442.bind.iou\endcsname{0.00}
\expandafter\def\csname BAval@tick.quad.f442.bind.state\endcsname{W}
\expandafter\def\csname BAval@tick.quad.f443.bind.iou\endcsname{0.00}
\expandafter\def\csname BAval@tick.quad.f443.bind.state\endcsname{W}
\expandafter\def\csname BAval@tick.quad.f444.bind.iou\endcsname{0.00}
\expandafter\def\csname BAval@tick.quad.f444.bind.state\endcsname{U}
\expandafter\def\csname BAval@tick.quad.f445.bind.iou\endcsname{0.00}
\expandafter\def\csname BAval@tick.quad.f445.bind.state\endcsname{U}
\expandafter\def\csname BAval@tick.quad.f446.bind.iou\endcsname{0.00}
\expandafter\def\csname BAval@tick.quad.f446.bind.state\endcsname{U}
\expandafter\def\csname BAval@tick.quad.f447.bind.iou\endcsname{0.00}
\expandafter\def\csname BAval@tick.quad.f447.bind.state\endcsname{U}
\expandafter\def\csname BAval@tick.quad.f448.bind.iou\endcsname{0.00}
\expandafter\def\csname BAval@tick.quad.f448.bind.state\endcsname{U}
\expandafter\def\csname BAval@tick.quad.f449.bind.iou\endcsname{0.00}
\expandafter\def\csname BAval@tick.quad.f449.bind.state\endcsname{U}
\expandafter\def\csname BAval@tick.quad.f450.bind.iou\endcsname{0.00}
\expandafter\def\csname BAval@tick.quad.f450.bind.state\endcsname{U}
\expandafter\def\csname BAval@tick.quad.f451.bind.iou\endcsname{0.00}
\expandafter\def\csname BAval@tick.quad.f451.bind.state\endcsname{U}
\expandafter\def\csname BAval@tick.quad.f452.bind.iou\endcsname{0.00}
\expandafter\def\csname BAval@tick.quad.f452.bind.state\endcsname{U}
\expandafter\def\csname BAval@tick.quad.f453.bind.iou\endcsname{0.00}
\expandafter\def\csname BAval@tick.quad.f453.bind.state\endcsname{U}
\expandafter\def\csname BAval@tick.quad.f454.bind.iou\endcsname{0.00}
\expandafter\def\csname BAval@tick.quad.f454.bind.state\endcsname{UNKNOWN}
\expandafter\def\csname BAval@tick.quad.f455.bind.iou\endcsname{0.00}
\expandafter\def\csname BAval@tick.quad.f455.bind.state\endcsname{UNKNOWN}
\expandafter\def\csname BAval@tick.quad.f456.bind.iou\endcsname{0.00}
\expandafter\def\csname BAval@tick.quad.f456.bind.state\endcsname{UNKNOWN}
\expandafter\def\csname BAval@tick.quad.f457.bind.iou\endcsname{0.00}
\expandafter\def\csname BAval@tick.quad.f457.bind.state\endcsname{W}
\expandafter\def\csname BAval@tick.quad.f458.bind.iou\endcsname{0.00}
\expandafter\def\csname BAval@tick.quad.f458.bind.state\endcsname{U}
\expandafter\def\csname BAval@tick.quad.f459.bind.iou\endcsname{0.00}
\expandafter\def\csname BAval@tick.quad.f459.bind.state\endcsname{U}
\expandafter\def\csname BAval@tick.quad.f460.bind.iou\endcsname{0.00}
\expandafter\def\csname BAval@tick.quad.f460.bind.state\endcsname{U}
\expandafter\def\csname BAval@tick.quad.f461.bind.iou\endcsname{0.00}
\expandafter\def\csname BAval@tick.quad.f461.bind.state\endcsname{U}
\expandafter\def\csname BAval@tick.quad.f462.bind.iou\endcsname{0.00}
\expandafter\def\csname BAval@tick.quad.f462.bind.state\endcsname{U}
\expandafter\def\csname BAval@tick.quad.f463.bind.iou\endcsname{0.00}
\expandafter\def\csname BAval@tick.quad.f463.bind.state\endcsname{U}
\expandafter\def\csname BAval@tick.quad.f464.bind.iou\endcsname{0.00}
\expandafter\def\csname BAval@tick.quad.f464.bind.state\endcsname{U}
\expandafter\def\csname BAval@tick.quad.f465.bind.iou\endcsname{0.00}
\expandafter\def\csname BAval@tick.quad.f465.bind.state\endcsname{U}
\expandafter\def\csname BAval@tick.quad.f466.bind.iou\endcsname{0.00}
\expandafter\def\csname BAval@tick.quad.f466.bind.state\endcsname{U}
\expandafter\def\csname BAval@tick.quad.f467.bind.iou\endcsname{0.00}
\expandafter\def\csname BAval@tick.quad.f467.bind.state\endcsname{U}
\expandafter\def\csname BAval@tick.quad.f468.bind.iou\endcsname{0.00}
\expandafter\def\csname BAval@tick.quad.f468.bind.state\endcsname{U}
\expandafter\def\csname BAval@tick.quad.f469.bind.iou\endcsname{0.00}
\expandafter\def\csname BAval@tick.quad.f469.bind.state\endcsname{U}
\expandafter\def\csname BAval@tick.quad.f470.bind.iou\endcsname{0.00}
\expandafter\def\csname BAval@tick.quad.f470.bind.state\endcsname{U}
\expandafter\def\csname BAval@tick.quad.f471.bind.iou\endcsname{0.00}
\expandafter\def\csname BAval@tick.quad.f471.bind.state\endcsname{U}
\expandafter\def\csname BAval@tick.quad.f472.bind.iou\endcsname{0.00}
\expandafter\def\csname BAval@tick.quad.f472.bind.state\endcsname{U}
\expandafter\def\csname BAval@tick.quad.f473.bind.iou\endcsname{0.00}
\expandafter\def\csname BAval@tick.quad.f473.bind.state\endcsname{UNKNOWN}
\expandafter\def\csname BAval@tick.quad.f474.bind.iou\endcsname{0.00}
\expandafter\def\csname BAval@tick.quad.f474.bind.state\endcsname{UNKNOWN}
\expandafter\def\csname BAval@tick.quad.f475.bind.iou\endcsname{0.00}
\expandafter\def\csname BAval@tick.quad.f475.bind.state\endcsname{UNKNOWN}
\expandafter\def\csname BAval@tick.quad.f476.bind.iou\endcsname{0.00}
\expandafter\def\csname BAval@tick.quad.f476.bind.state\endcsname{UNKNOWN}
\expandafter\def\csname BAval@tick.quad.f477.bind.iou\endcsname{0.00}
\expandafter\def\csname BAval@tick.quad.f477.bind.state\endcsname{U}
\expandafter\def\csname BAval@tick.quad.f478.bind.iou\endcsname{0.00}
\expandafter\def\csname BAval@tick.quad.f478.bind.state\endcsname{U}
\expandafter\def\csname BAval@tick.quad.f479.bind.iou\endcsname{0.00}
\expandafter\def\csname BAval@tick.quad.f479.bind.state\endcsname{U}
\expandafter\def\csname BAval@tick.quad.f480.bind.iou\endcsname{0.00}
\expandafter\def\csname BAval@tick.quad.f480.bind.state\endcsname{U}
\expandafter\def\csname BAval@tick.quad.f481.bind.iou\endcsname{0.00}
\expandafter\def\csname BAval@tick.quad.f481.bind.state\endcsname{U}
\expandafter\def\csname BAval@tick.quad.f482.bind.iou\endcsname{0.00}
\expandafter\def\csname BAval@tick.quad.f482.bind.state\endcsname{U}
\expandafter\def\csname BAval@tick.quad.f483.bind.iou\endcsname{0.00}
\expandafter\def\csname BAval@tick.quad.f483.bind.state\endcsname{U}
\expandafter\def\csname BAval@tick.quad.f484.bind.iou\endcsname{0.00}
\expandafter\def\csname BAval@tick.quad.f484.bind.state\endcsname{U}
\expandafter\def\csname BAval@tick.quad.f485.bind.iou\endcsname{0.00}
\expandafter\def\csname BAval@tick.quad.f485.bind.state\endcsname{U}
\expandafter\def\csname BAval@tick.quad.f486.bind.iou\endcsname{0.00}
\expandafter\def\csname BAval@tick.quad.f486.bind.state\endcsname{W}
\expandafter\def\csname BAval@tick.quad.f487.bind.iou\endcsname{0.00}
\expandafter\def\csname BAval@tick.quad.f487.bind.state\endcsname{W}
\expandafter\def\csname BAval@tick.quad.f488.bind.iou\endcsname{0.00}
\expandafter\def\csname BAval@tick.quad.f488.bind.state\endcsname{W}
\expandafter\def\csname BAval@tick.quad.f489.bind.iou\endcsname{0.00}
\expandafter\def\csname BAval@tick.quad.f489.bind.state\endcsname{W}
\expandafter\def\csname BAval@tick.quad.f490.bind.iou\endcsname{0.00}
\expandafter\def\csname BAval@tick.quad.f490.bind.state\endcsname{U}
\expandafter\def\csname BAval@tick.quad.f491.bind.iou\endcsname{0.00}
\expandafter\def\csname BAval@tick.quad.f491.bind.state\endcsname{U}
\expandafter\def\csname BAval@tick.quad.f492.bind.iou\endcsname{0.00}
\expandafter\def\csname BAval@tick.quad.f492.bind.state\endcsname{U}
\expandafter\def\csname BAval@tick.quad.f493.bind.iou\endcsname{0.00}
\expandafter\def\csname BAval@tick.quad.f493.bind.state\endcsname{UNKNOWN}
\expandafter\def\csname BAval@tick.quad.f494.bind.iou\endcsname{0.00}
\expandafter\def\csname BAval@tick.quad.f494.bind.state\endcsname{UNKNOWN}
\expandafter\def\csname BAval@tick.quad.f495.bind.iou\endcsname{0.00}
\expandafter\def\csname BAval@tick.quad.f495.bind.state\endcsname{UNKNOWN}
\expandafter\def\csname BAval@tick.quad.f496.bind.iou\endcsname{0.00}
\expandafter\def\csname BAval@tick.quad.f496.bind.state\endcsname{UNKNOWN}
\expandafter\def\csname BAval@tick.quad.f497.bind.iou\endcsname{0.00}
\expandafter\def\csname BAval@tick.quad.f497.bind.state\endcsname{UNKNOWN}
\expandafter\def\csname BAval@tick.quad.f498.bind.iou\endcsname{0.00}
\expandafter\def\csname BAval@tick.quad.f498.bind.state\endcsname{UNKNOWN}
\expandafter\def\csname BAval@rec.dance.attempts\endcsname{12}
\expandafter\def\csname BAval@rec.dance.complete\endcsname{0}
\expandafter\def\csname BAval@rec.dance.fallwait\endcsname{10}
\expandafter\def\csname BAval@rec.dance.expired\endcsname{2}
\expandafter\def\csname BAval@rec.dance.requests\endcsname{0}
\expandafter\def\csname BAval@rec.dance.returns\endcsname{0}
\expandafter\def\csname BAval@rec.dance.initialpub\endcsname{1}
\expandafter\def\csname BAval@rec.dance.laterpub\endcsname{0}
\expandafter\def\csname BAval@rec.dance.nativeupdates\endcsname{0}
\expandafter\def\csname BAval@rec.dance.ticks\endcsname{180}
\expandafter\def\csname BAval@state.dance.dam.correct\endcsname{78}
\expandafter\def\csname BAval@state.dance.dam.wrong\endcsname{20}
\expandafter\def\csname BAval@state.dance.dam.unresolved\endcsname{82}
\expandafter\def\csname BAval@state.dance.dam.unknown\endcsname{0}
\expandafter\def\csname BAval@tick.dance.f159.dam.iou\endcsname{0.99}
\expandafter\def\csname BAval@tick.dance.f159.dam.state\endcsname{C}
\expandafter\def\csname BAval@tick.dance.f160.dam.iou\endcsname{0.98}
\expandafter\def\csname BAval@tick.dance.f160.dam.state\endcsname{C}
\expandafter\def\csname BAval@tick.dance.f161.dam.iou\endcsname{0.97}
\expandafter\def\csname BAval@tick.dance.f161.dam.state\endcsname{C}
\expandafter\def\csname BAval@tick.dance.f162.dam.iou\endcsname{0.97}
\expandafter\def\csname BAval@tick.dance.f162.dam.state\endcsname{C}
\expandafter\def\csname BAval@tick.dance.f163.dam.iou\endcsname{0.95}
\expandafter\def\csname BAval@tick.dance.f163.dam.state\endcsname{C}
\expandafter\def\csname BAval@tick.dance.f164.dam.iou\endcsname{0.94}
\expandafter\def\csname BAval@tick.dance.f164.dam.state\endcsname{C}
\expandafter\def\csname BAval@tick.dance.f165.dam.iou\endcsname{0.92}
\expandafter\def\csname BAval@tick.dance.f165.dam.state\endcsname{C}
\expandafter\def\csname BAval@tick.dance.f166.dam.iou\endcsname{0.89}
\expandafter\def\csname BAval@tick.dance.f166.dam.state\endcsname{C}
\expandafter\def\csname BAval@tick.dance.f167.dam.iou\endcsname{0.87}
\expandafter\def\csname BAval@tick.dance.f167.dam.state\endcsname{C}
\expandafter\def\csname BAval@tick.dance.f168.dam.iou\endcsname{0.86}
\expandafter\def\csname BAval@tick.dance.f168.dam.state\endcsname{C}
\expandafter\def\csname BAval@tick.dance.f169.dam.iou\endcsname{0.83}
\expandafter\def\csname BAval@tick.dance.f169.dam.state\endcsname{C}
\expandafter\def\csname BAval@tick.dance.f170.dam.iou\endcsname{0.60}
\expandafter\def\csname BAval@tick.dance.f170.dam.state\endcsname{C}
\expandafter\def\csname BAval@tick.dance.f171.dam.iou\endcsname{0.52}
\expandafter\def\csname BAval@tick.dance.f171.dam.state\endcsname{C}
\expandafter\def\csname BAval@tick.dance.f172.dam.iou\endcsname{0.46}
\expandafter\def\csname BAval@tick.dance.f172.dam.state\endcsname{U}
\expandafter\def\csname BAval@tick.dance.f173.dam.iou\endcsname{0.51}
\expandafter\def\csname BAval@tick.dance.f173.dam.state\endcsname{C}
\expandafter\def\csname BAval@tick.dance.f174.dam.iou\endcsname{0.45}
\expandafter\def\csname BAval@tick.dance.f174.dam.state\endcsname{U}
\expandafter\def\csname BAval@tick.dance.f175.dam.iou\endcsname{0.44}
\expandafter\def\csname BAval@tick.dance.f175.dam.state\endcsname{U}
\expandafter\def\csname BAval@tick.dance.f176.dam.iou\endcsname{0.42}
\expandafter\def\csname BAval@tick.dance.f176.dam.state\endcsname{U}
\expandafter\def\csname BAval@tick.dance.f177.dam.iou\endcsname{0.42}
\expandafter\def\csname BAval@tick.dance.f177.dam.state\endcsname{U}
\expandafter\def\csname BAval@tick.dance.f178.dam.iou\endcsname{0.41}
\expandafter\def\csname BAval@tick.dance.f178.dam.state\endcsname{U}
\expandafter\def\csname BAval@tick.dance.f179.dam.iou\endcsname{0.39}
\expandafter\def\csname BAval@tick.dance.f179.dam.state\endcsname{U}
\expandafter\def\csname BAval@tick.dance.f180.dam.iou\endcsname{0.30}
\expandafter\def\csname BAval@tick.dance.f180.dam.state\endcsname{U}
\expandafter\def\csname BAval@tick.dance.f181.dam.iou\endcsname{0.27}
\expandafter\def\csname BAval@tick.dance.f181.dam.state\endcsname{U}
\expandafter\def\csname BAval@tick.dance.f182.dam.iou\endcsname{0.19}
\expandafter\def\csname BAval@tick.dance.f182.dam.state\endcsname{U}
\expandafter\def\csname BAval@tick.dance.f183.dam.iou\endcsname{0.14}
\expandafter\def\csname BAval@tick.dance.f183.dam.state\endcsname{U}
\expandafter\def\csname BAval@tick.dance.f184.dam.iou\endcsname{0.10}
\expandafter\def\csname BAval@tick.dance.f184.dam.state\endcsname{U}
\expandafter\def\csname BAval@tick.dance.f185.dam.iou\endcsname{0.08}
\expandafter\def\csname BAval@tick.dance.f185.dam.state\endcsname{W}
\expandafter\def\csname BAval@tick.dance.f186.dam.iou\endcsname{0.06}
\expandafter\def\csname BAval@tick.dance.f186.dam.state\endcsname{W}
\expandafter\def\csname BAval@tick.dance.f187.dam.iou\endcsname{0.04}
\expandafter\def\csname BAval@tick.dance.f187.dam.state\endcsname{W}
\expandafter\def\csname BAval@tick.dance.f188.dam.iou\endcsname{0.03}
\expandafter\def\csname BAval@tick.dance.f188.dam.state\endcsname{W}
\expandafter\def\csname BAval@tick.dance.f189.dam.iou\endcsname{0.02}
\expandafter\def\csname BAval@tick.dance.f189.dam.state\endcsname{W}
\expandafter\def\csname BAval@tick.dance.f190.dam.iou\endcsname{0.02}
\expandafter\def\csname BAval@tick.dance.f190.dam.state\endcsname{W}
\expandafter\def\csname BAval@tick.dance.f191.dam.iou\endcsname{0.02}
\expandafter\def\csname BAval@tick.dance.f191.dam.state\endcsname{W}
\expandafter\def\csname BAval@tick.dance.f192.dam.iou\endcsname{0.00}
\expandafter\def\csname BAval@tick.dance.f192.dam.state\endcsname{W}
\expandafter\def\csname BAval@tick.dance.f193.dam.iou\endcsname{0.00}
\expandafter\def\csname BAval@tick.dance.f193.dam.state\endcsname{W}
\expandafter\def\csname BAval@tick.dance.f194.dam.iou\endcsname{0.00}
\expandafter\def\csname BAval@tick.dance.f194.dam.state\endcsname{W}
\expandafter\def\csname BAval@tick.dance.f195.dam.iou\endcsname{0.00}
\expandafter\def\csname BAval@tick.dance.f195.dam.state\endcsname{W}
\expandafter\def\csname BAval@tick.dance.f196.dam.iou\endcsname{0.00}
\expandafter\def\csname BAval@tick.dance.f196.dam.state\endcsname{W}
\expandafter\def\csname BAval@tick.dance.f197.dam.iou\endcsname{0.00}
\expandafter\def\csname BAval@tick.dance.f197.dam.state\endcsname{W}
\expandafter\def\csname BAval@tick.dance.f198.dam.iou\endcsname{0.00}
\expandafter\def\csname BAval@tick.dance.f198.dam.state\endcsname{U}
\expandafter\def\csname BAval@tick.dance.f199.dam.iou\endcsname{0.00}
\expandafter\def\csname BAval@tick.dance.f199.dam.state\endcsname{U}
\expandafter\def\csname BAval@tick.dance.f200.dam.iou\endcsname{0.00}
\expandafter\def\csname BAval@tick.dance.f200.dam.state\endcsname{U}
\expandafter\def\csname BAval@tick.dance.f201.dam.iou\endcsname{0.00}
\expandafter\def\csname BAval@tick.dance.f201.dam.state\endcsname{U}
\expandafter\def\csname BAval@tick.dance.f202.dam.iou\endcsname{0.00}
\expandafter\def\csname BAval@tick.dance.f202.dam.state\endcsname{U}
\expandafter\def\csname BAval@tick.dance.f203.dam.iou\endcsname{0.00}
\expandafter\def\csname BAval@tick.dance.f203.dam.state\endcsname{U}
\expandafter\def\csname BAval@tick.dance.f204.dam.iou\endcsname{0.00}
\expandafter\def\csname BAval@tick.dance.f204.dam.state\endcsname{U}
\expandafter\def\csname BAval@tick.dance.f205.dam.iou\endcsname{0.00}
\expandafter\def\csname BAval@tick.dance.f205.dam.state\endcsname{U}
\expandafter\def\csname BAval@tick.dance.f206.dam.iou\endcsname{0.03}
\expandafter\def\csname BAval@tick.dance.f206.dam.state\endcsname{U}
\expandafter\def\csname BAval@tick.dance.f207.dam.iou\endcsname{0.04}
\expandafter\def\csname BAval@tick.dance.f207.dam.state\endcsname{U}
\expandafter\def\csname BAval@tick.dance.f208.dam.iou\endcsname{0.04}
\expandafter\def\csname BAval@tick.dance.f208.dam.state\endcsname{U}
\expandafter\def\csname BAval@tick.dance.f209.dam.iou\endcsname{0.04}
\expandafter\def\csname BAval@tick.dance.f209.dam.state\endcsname{U}
\expandafter\def\csname BAval@tick.dance.f210.dam.iou\endcsname{0.07}
\expandafter\def\csname BAval@tick.dance.f210.dam.state\endcsname{U}
\expandafter\def\csname BAval@tick.dance.f211.dam.iou\endcsname{0.09}
\expandafter\def\csname BAval@tick.dance.f211.dam.state\endcsname{U}
\expandafter\def\csname BAval@tick.dance.f212.dam.iou\endcsname{0.12}
\expandafter\def\csname BAval@tick.dance.f212.dam.state\endcsname{U}
\expandafter\def\csname BAval@tick.dance.f213.dam.iou\endcsname{0.13}
\expandafter\def\csname BAval@tick.dance.f213.dam.state\endcsname{U}
\expandafter\def\csname BAval@tick.dance.f214.dam.iou\endcsname{0.14}
\expandafter\def\csname BAval@tick.dance.f214.dam.state\endcsname{U}
\expandafter\def\csname BAval@tick.dance.f215.dam.iou\endcsname{0.15}
\expandafter\def\csname BAval@tick.dance.f215.dam.state\endcsname{U}
\expandafter\def\csname BAval@tick.dance.f216.dam.iou\endcsname{0.21}
\expandafter\def\csname BAval@tick.dance.f216.dam.state\endcsname{U}
\expandafter\def\csname BAval@tick.dance.f217.dam.iou\endcsname{0.24}
\expandafter\def\csname BAval@tick.dance.f217.dam.state\endcsname{U}
\expandafter\def\csname BAval@tick.dance.f218.dam.iou\endcsname{0.37}
\expandafter\def\csname BAval@tick.dance.f218.dam.state\endcsname{U}
\expandafter\def\csname BAval@tick.dance.f219.dam.iou\endcsname{0.41}
\expandafter\def\csname BAval@tick.dance.f219.dam.state\endcsname{U}
\expandafter\def\csname BAval@tick.dance.f220.dam.iou\endcsname{0.46}
\expandafter\def\csname BAval@tick.dance.f220.dam.state\endcsname{U}
\expandafter\def\csname BAval@tick.dance.f221.dam.iou\endcsname{0.51}
\expandafter\def\csname BAval@tick.dance.f221.dam.state\endcsname{C}
\expandafter\def\csname BAval@tick.dance.f222.dam.iou\endcsname{0.53}
\expandafter\def\csname BAval@tick.dance.f222.dam.state\endcsname{C}
\expandafter\def\csname BAval@tick.dance.f223.dam.iou\endcsname{0.53}
\expandafter\def\csname BAval@tick.dance.f223.dam.state\endcsname{C}
\expandafter\def\csname BAval@tick.dance.f224.dam.iou\endcsname{0.53}
\expandafter\def\csname BAval@tick.dance.f224.dam.state\endcsname{C}
\expandafter\def\csname BAval@tick.dance.f225.dam.iou\endcsname{0.54}
\expandafter\def\csname BAval@tick.dance.f225.dam.state\endcsname{C}
\expandafter\def\csname BAval@tick.dance.f226.dam.iou\endcsname{0.56}
\expandafter\def\csname BAval@tick.dance.f226.dam.state\endcsname{C}
\expandafter\def\csname BAval@tick.dance.f227.dam.iou\endcsname{0.55}
\expandafter\def\csname BAval@tick.dance.f227.dam.state\endcsname{C}
\expandafter\def\csname BAval@tick.dance.f228.dam.iou\endcsname{0.55}
\expandafter\def\csname BAval@tick.dance.f228.dam.state\endcsname{C}
\expandafter\def\csname BAval@tick.dance.f229.dam.iou\endcsname{0.54}
\expandafter\def\csname BAval@tick.dance.f229.dam.state\endcsname{C}
\expandafter\def\csname BAval@tick.dance.f230.dam.iou\endcsname{0.55}
\expandafter\def\csname BAval@tick.dance.f230.dam.state\endcsname{C}
\expandafter\def\csname BAval@tick.dance.f231.dam.iou\endcsname{0.55}
\expandafter\def\csname BAval@tick.dance.f231.dam.state\endcsname{C}
\expandafter\def\csname BAval@tick.dance.f232.dam.iou\endcsname{0.55}
\expandafter\def\csname BAval@tick.dance.f232.dam.state\endcsname{C}
\expandafter\def\csname BAval@tick.dance.f233.dam.iou\endcsname{0.56}
\expandafter\def\csname BAval@tick.dance.f233.dam.state\endcsname{C}
\expandafter\def\csname BAval@tick.dance.f234.dam.iou\endcsname{0.56}
\expandafter\def\csname BAval@tick.dance.f234.dam.state\endcsname{C}
\expandafter\def\csname BAval@tick.dance.f235.dam.iou\endcsname{0.56}
\expandafter\def\csname BAval@tick.dance.f235.dam.state\endcsname{C}
\expandafter\def\csname BAval@tick.dance.f236.dam.iou\endcsname{0.57}
\expandafter\def\csname BAval@tick.dance.f236.dam.state\endcsname{C}
\expandafter\def\csname BAval@tick.dance.f237.dam.iou\endcsname{0.58}
\expandafter\def\csname BAval@tick.dance.f237.dam.state\endcsname{C}
\expandafter\def\csname BAval@tick.dance.f238.dam.iou\endcsname{0.57}
\expandafter\def\csname BAval@tick.dance.f238.dam.state\endcsname{C}
\expandafter\def\csname BAval@tick.dance.f239.dam.iou\endcsname{0.58}
\expandafter\def\csname BAval@tick.dance.f239.dam.state\endcsname{C}
\expandafter\def\csname BAval@tick.dance.f240.dam.iou\endcsname{0.57}
\expandafter\def\csname BAval@tick.dance.f240.dam.state\endcsname{C}
\expandafter\def\csname BAval@tick.dance.f241.dam.iou\endcsname{0.58}
\expandafter\def\csname BAval@tick.dance.f241.dam.state\endcsname{C}
\expandafter\def\csname BAval@tick.dance.f242.dam.iou\endcsname{0.58}
\expandafter\def\csname BAval@tick.dance.f242.dam.state\endcsname{C}
\expandafter\def\csname BAval@tick.dance.f243.dam.iou\endcsname{0.59}
\expandafter\def\csname BAval@tick.dance.f243.dam.state\endcsname{C}
\expandafter\def\csname BAval@tick.dance.f244.dam.iou\endcsname{0.59}
\expandafter\def\csname BAval@tick.dance.f244.dam.state\endcsname{C}
\expandafter\def\csname BAval@tick.dance.f245.dam.iou\endcsname{0.60}
\expandafter\def\csname BAval@tick.dance.f245.dam.state\endcsname{C}
\expandafter\def\csname BAval@tick.dance.f246.dam.iou\endcsname{0.58}
\expandafter\def\csname BAval@tick.dance.f246.dam.state\endcsname{C}
\expandafter\def\csname BAval@tick.dance.f247.dam.iou\endcsname{0.60}
\expandafter\def\csname BAval@tick.dance.f247.dam.state\endcsname{C}
\expandafter\def\csname BAval@tick.dance.f248.dam.iou\endcsname{0.58}
\expandafter\def\csname BAval@tick.dance.f248.dam.state\endcsname{C}
\expandafter\def\csname BAval@tick.dance.f249.dam.iou\endcsname{0.57}
\expandafter\def\csname BAval@tick.dance.f249.dam.state\endcsname{C}
\expandafter\def\csname BAval@tick.dance.f250.dam.iou\endcsname{0.57}
\expandafter\def\csname BAval@tick.dance.f250.dam.state\endcsname{C}
\expandafter\def\csname BAval@tick.dance.f251.dam.iou\endcsname{0.57}
\expandafter\def\csname BAval@tick.dance.f251.dam.state\endcsname{C}
\expandafter\def\csname BAval@tick.dance.f252.dam.iou\endcsname{0.57}
\expandafter\def\csname BAval@tick.dance.f252.dam.state\endcsname{C}
\expandafter\def\csname BAval@tick.dance.f253.dam.iou\endcsname{0.56}
\expandafter\def\csname BAval@tick.dance.f253.dam.state\endcsname{C}
\expandafter\def\csname BAval@tick.dance.f254.dam.iou\endcsname{0.56}
\expandafter\def\csname BAval@tick.dance.f254.dam.state\endcsname{C}
\expandafter\def\csname BAval@tick.dance.f255.dam.iou\endcsname{0.56}
\expandafter\def\csname BAval@tick.dance.f255.dam.state\endcsname{C}
\expandafter\def\csname BAval@tick.dance.f256.dam.iou\endcsname{0.56}
\expandafter\def\csname BAval@tick.dance.f256.dam.state\endcsname{C}
\expandafter\def\csname BAval@tick.dance.f257.dam.iou\endcsname{0.56}
\expandafter\def\csname BAval@tick.dance.f257.dam.state\endcsname{C}
\expandafter\def\csname BAval@tick.dance.f258.dam.iou\endcsname{0.56}
\expandafter\def\csname BAval@tick.dance.f258.dam.state\endcsname{C}
\expandafter\def\csname BAval@tick.dance.f259.dam.iou\endcsname{0.56}
\expandafter\def\csname BAval@tick.dance.f259.dam.state\endcsname{C}
\expandafter\def\csname BAval@tick.dance.f260.dam.iou\endcsname{0.56}
\expandafter\def\csname BAval@tick.dance.f260.dam.state\endcsname{C}
\expandafter\def\csname BAval@tick.dance.f261.dam.iou\endcsname{0.56}
\expandafter\def\csname BAval@tick.dance.f261.dam.state\endcsname{C}
\expandafter\def\csname BAval@tick.dance.f262.dam.iou\endcsname{0.56}
\expandafter\def\csname BAval@tick.dance.f262.dam.state\endcsname{C}
\expandafter\def\csname BAval@tick.dance.f263.dam.iou\endcsname{0.56}
\expandafter\def\csname BAval@tick.dance.f263.dam.state\endcsname{C}
\expandafter\def\csname BAval@tick.dance.f264.dam.iou\endcsname{0.56}
\expandafter\def\csname BAval@tick.dance.f264.dam.state\endcsname{C}
\expandafter\def\csname BAval@tick.dance.f265.dam.iou\endcsname{0.56}
\expandafter\def\csname BAval@tick.dance.f265.dam.state\endcsname{C}
\expandafter\def\csname BAval@tick.dance.f266.dam.iou\endcsname{0.56}
\expandafter\def\csname BAval@tick.dance.f266.dam.state\endcsname{C}
\expandafter\def\csname BAval@tick.dance.f267.dam.iou\endcsname{0.56}
\expandafter\def\csname BAval@tick.dance.f267.dam.state\endcsname{C}
\expandafter\def\csname BAval@tick.dance.f268.dam.iou\endcsname{0.57}
\expandafter\def\csname BAval@tick.dance.f268.dam.state\endcsname{C}
\expandafter\def\csname BAval@tick.dance.f269.dam.iou\endcsname{0.58}
\expandafter\def\csname BAval@tick.dance.f269.dam.state\endcsname{C}
\expandafter\def\csname BAval@tick.dance.f270.dam.iou\endcsname{0.58}
\expandafter\def\csname BAval@tick.dance.f270.dam.state\endcsname{C}
\expandafter\def\csname BAval@tick.dance.f271.dam.iou\endcsname{0.59}
\expandafter\def\csname BAval@tick.dance.f271.dam.state\endcsname{C}
\expandafter\def\csname BAval@tick.dance.f272.dam.iou\endcsname{0.59}
\expandafter\def\csname BAval@tick.dance.f272.dam.state\endcsname{C}
\expandafter\def\csname BAval@tick.dance.f273.dam.iou\endcsname{0.60}
\expandafter\def\csname BAval@tick.dance.f273.dam.state\endcsname{C}
\expandafter\def\csname BAval@tick.dance.f274.dam.iou\endcsname{0.61}
\expandafter\def\csname BAval@tick.dance.f274.dam.state\endcsname{C}
\expandafter\def\csname BAval@tick.dance.f275.dam.iou\endcsname{0.62}
\expandafter\def\csname BAval@tick.dance.f275.dam.state\endcsname{C}
\expandafter\def\csname BAval@tick.dance.f276.dam.iou\endcsname{0.61}
\expandafter\def\csname BAval@tick.dance.f276.dam.state\endcsname{C}
\expandafter\def\csname BAval@tick.dance.f277.dam.iou\endcsname{0.61}
\expandafter\def\csname BAval@tick.dance.f277.dam.state\endcsname{C}
\expandafter\def\csname BAval@tick.dance.f278.dam.iou\endcsname{0.61}
\expandafter\def\csname BAval@tick.dance.f278.dam.state\endcsname{C}
\expandafter\def\csname BAval@tick.dance.f279.dam.iou\endcsname{0.54}
\expandafter\def\csname BAval@tick.dance.f279.dam.state\endcsname{C}
\expandafter\def\csname BAval@tick.dance.f280.dam.iou\endcsname{0.55}
\expandafter\def\csname BAval@tick.dance.f280.dam.state\endcsname{C}
\expandafter\def\csname BAval@tick.dance.f281.dam.iou\endcsname{0.57}
\expandafter\def\csname BAval@tick.dance.f281.dam.state\endcsname{C}
\expandafter\def\csname BAval@tick.dance.f282.dam.iou\endcsname{0.59}
\expandafter\def\csname BAval@tick.dance.f282.dam.state\endcsname{C}
\expandafter\def\csname BAval@tick.dance.f283.dam.iou\endcsname{0.64}
\expandafter\def\csname BAval@tick.dance.f283.dam.state\endcsname{C}
\expandafter\def\csname BAval@tick.dance.f284.dam.iou\endcsname{0.61}
\expandafter\def\csname BAval@tick.dance.f284.dam.state\endcsname{C}
\expandafter\def\csname BAval@tick.dance.f285.dam.iou\endcsname{0.47}
\expandafter\def\csname BAval@tick.dance.f285.dam.state\endcsname{U}
\expandafter\def\csname BAval@tick.dance.f286.dam.iou\endcsname{0.40}
\expandafter\def\csname BAval@tick.dance.f286.dam.state\endcsname{U}
\expandafter\def\csname BAval@tick.dance.f287.dam.iou\endcsname{0.30}
\expandafter\def\csname BAval@tick.dance.f287.dam.state\endcsname{U}
\expandafter\def\csname BAval@tick.dance.f288.dam.iou\endcsname{0.21}
\expandafter\def\csname BAval@tick.dance.f288.dam.state\endcsname{U}
\expandafter\def\csname BAval@tick.dance.f289.dam.iou\endcsname{0.15}
\expandafter\def\csname BAval@tick.dance.f289.dam.state\endcsname{U}
\expandafter\def\csname BAval@tick.dance.f290.dam.iou\endcsname{0.13}
\expandafter\def\csname BAval@tick.dance.f290.dam.state\endcsname{U}
\expandafter\def\csname BAval@tick.dance.f291.dam.iou\endcsname{0.05}
\expandafter\def\csname BAval@tick.dance.f291.dam.state\endcsname{U}
\expandafter\def\csname BAval@tick.dance.f292.dam.iou\endcsname{0.03}
\expandafter\def\csname BAval@tick.dance.f292.dam.state\endcsname{U}
\expandafter\def\csname BAval@tick.dance.f293.dam.iou\endcsname{0.00}
\expandafter\def\csname BAval@tick.dance.f293.dam.state\endcsname{W}
\expandafter\def\csname BAval@tick.dance.f294.dam.iou\endcsname{0.00}
\expandafter\def\csname BAval@tick.dance.f294.dam.state\endcsname{W}
\expandafter\def\csname BAval@tick.dance.f295.dam.iou\endcsname{0.00}
\expandafter\def\csname BAval@tick.dance.f295.dam.state\endcsname{W}
\expandafter\def\csname BAval@tick.dance.f296.dam.iou\endcsname{0.00}
\expandafter\def\csname BAval@tick.dance.f296.dam.state\endcsname{W}
\expandafter\def\csname BAval@tick.dance.f297.dam.iou\endcsname{0.00}
\expandafter\def\csname BAval@tick.dance.f297.dam.state\endcsname{W}
\expandafter\def\csname BAval@tick.dance.f298.dam.iou\endcsname{0.00}
\expandafter\def\csname BAval@tick.dance.f298.dam.state\endcsname{W}
\expandafter\def\csname BAval@tick.dance.f299.dam.iou\endcsname{0.00}
\expandafter\def\csname BAval@tick.dance.f299.dam.state\endcsname{U}
\expandafter\def\csname BAval@tick.dance.f300.dam.iou\endcsname{0.00}
\expandafter\def\csname BAval@tick.dance.f300.dam.state\endcsname{U}
\expandafter\def\csname BAval@tick.dance.f301.dam.iou\endcsname{0.00}
\expandafter\def\csname BAval@tick.dance.f301.dam.state\endcsname{U}
\expandafter\def\csname BAval@tick.dance.f302.dam.iou\endcsname{0.00}
\expandafter\def\csname BAval@tick.dance.f302.dam.state\endcsname{U}
\expandafter\def\csname BAval@tick.dance.f303.dam.iou\endcsname{0.00}
\expandafter\def\csname BAval@tick.dance.f303.dam.state\endcsname{U}
\expandafter\def\csname BAval@tick.dance.f304.dam.iou\endcsname{0.00}
\expandafter\def\csname BAval@tick.dance.f304.dam.state\endcsname{U}
\expandafter\def\csname BAval@tick.dance.f305.dam.iou\endcsname{0.00}
\expandafter\def\csname BAval@tick.dance.f305.dam.state\endcsname{U}
\expandafter\def\csname BAval@tick.dance.f306.dam.iou\endcsname{0.00}
\expandafter\def\csname BAval@tick.dance.f306.dam.state\endcsname{U}
\expandafter\def\csname BAval@tick.dance.f307.dam.iou\endcsname{0.00}
\expandafter\def\csname BAval@tick.dance.f307.dam.state\endcsname{U}
\expandafter\def\csname BAval@tick.dance.f308.dam.iou\endcsname{0.00}
\expandafter\def\csname BAval@tick.dance.f308.dam.state\endcsname{U}
\expandafter\def\csname BAval@tick.dance.f309.dam.iou\endcsname{0.00}
\expandafter\def\csname BAval@tick.dance.f309.dam.state\endcsname{U}
\expandafter\def\csname BAval@tick.dance.f310.dam.iou\endcsname{0.00}
\expandafter\def\csname BAval@tick.dance.f310.dam.state\endcsname{U}
\expandafter\def\csname BAval@tick.dance.f311.dam.iou\endcsname{0.00}
\expandafter\def\csname BAval@tick.dance.f311.dam.state\endcsname{U}
\expandafter\def\csname BAval@tick.dance.f312.dam.iou\endcsname{0.00}
\expandafter\def\csname BAval@tick.dance.f312.dam.state\endcsname{U}
\expandafter\def\csname BAval@tick.dance.f313.dam.iou\endcsname{0.00}
\expandafter\def\csname BAval@tick.dance.f313.dam.state\endcsname{U}
\expandafter\def\csname BAval@tick.dance.f314.dam.iou\endcsname{0.00}
\expandafter\def\csname BAval@tick.dance.f314.dam.state\endcsname{U}
\expandafter\def\csname BAval@tick.dance.f315.dam.iou\endcsname{0.00}
\expandafter\def\csname BAval@tick.dance.f315.dam.state\endcsname{U}
\expandafter\def\csname BAval@tick.dance.f316.dam.iou\endcsname{0.00}
\expandafter\def\csname BAval@tick.dance.f316.dam.state\endcsname{U}
\expandafter\def\csname BAval@tick.dance.f317.dam.iou\endcsname{0.00}
\expandafter\def\csname BAval@tick.dance.f317.dam.state\endcsname{W}
\expandafter\def\csname BAval@tick.dance.f318.dam.iou\endcsname{0.00}
\expandafter\def\csname BAval@tick.dance.f318.dam.state\endcsname{U}
\expandafter\def\csname BAval@tick.dance.f319.dam.iou\endcsname{0.00}
\expandafter\def\csname BAval@tick.dance.f319.dam.state\endcsname{U}
\expandafter\def\csname BAval@tick.dance.f320.dam.iou\endcsname{0.00}
\expandafter\def\csname BAval@tick.dance.f320.dam.state\endcsname{U}
\expandafter\def\csname BAval@tick.dance.f321.dam.iou\endcsname{0.00}
\expandafter\def\csname BAval@tick.dance.f321.dam.state\endcsname{U}
\expandafter\def\csname BAval@tick.dance.f322.dam.iou\endcsname{0.00}
\expandafter\def\csname BAval@tick.dance.f322.dam.state\endcsname{U}
\expandafter\def\csname BAval@tick.dance.f323.dam.iou\endcsname{0.00}
\expandafter\def\csname BAval@tick.dance.f323.dam.state\endcsname{U}
\expandafter\def\csname BAval@tick.dance.f324.dam.iou\endcsname{0.00}
\expandafter\def\csname BAval@tick.dance.f324.dam.state\endcsname{U}
\expandafter\def\csname BAval@tick.dance.f325.dam.iou\endcsname{0.00}
\expandafter\def\csname BAval@tick.dance.f325.dam.state\endcsname{U}
\expandafter\def\csname BAval@tick.dance.f326.dam.iou\endcsname{0.00}
\expandafter\def\csname BAval@tick.dance.f326.dam.state\endcsname{U}
\expandafter\def\csname BAval@tick.dance.f327.dam.iou\endcsname{0.00}
\expandafter\def\csname BAval@tick.dance.f327.dam.state\endcsname{U}
\expandafter\def\csname BAval@tick.dance.f328.dam.iou\endcsname{0.00}
\expandafter\def\csname BAval@tick.dance.f328.dam.state\endcsname{U}
\expandafter\def\csname BAval@tick.dance.f329.dam.iou\endcsname{0.00}
\expandafter\def\csname BAval@tick.dance.f329.dam.state\endcsname{U}
\expandafter\def\csname BAval@tick.dance.f330.dam.iou\endcsname{0.00}
\expandafter\def\csname BAval@tick.dance.f330.dam.state\endcsname{U}
\expandafter\def\csname BAval@tick.dance.f331.dam.iou\endcsname{0.00}
\expandafter\def\csname BAval@tick.dance.f331.dam.state\endcsname{U}
\expandafter\def\csname BAval@tick.dance.f332.dam.iou\endcsname{0.00}
\expandafter\def\csname BAval@tick.dance.f332.dam.state\endcsname{U}
\expandafter\def\csname BAval@tick.dance.f333.dam.iou\endcsname{0.00}
\expandafter\def\csname BAval@tick.dance.f333.dam.state\endcsname{U}
\expandafter\def\csname BAval@tick.dance.f334.dam.iou\endcsname{0.00}
\expandafter\def\csname BAval@tick.dance.f334.dam.state\endcsname{U}
\expandafter\def\csname BAval@tick.dance.f335.dam.iou\endcsname{0.00}
\expandafter\def\csname BAval@tick.dance.f335.dam.state\endcsname{U}
\expandafter\def\csname BAval@tick.dance.f336.dam.iou\endcsname{0.00}
\expandafter\def\csname BAval@tick.dance.f336.dam.state\endcsname{U}
\expandafter\def\csname BAval@tick.dance.f337.dam.iou\endcsname{0.00}
\expandafter\def\csname BAval@tick.dance.f337.dam.state\endcsname{U}
\expandafter\def\csname BAval@tick.dance.f338.dam.iou\endcsname{0.00}
\expandafter\def\csname BAval@tick.dance.f338.dam.state\endcsname{U}
\expandafter\def\csname BAval@state.dance.keep.correct\endcsname{72}
\expandafter\def\csname BAval@state.dance.keep.wrong\endcsname{23}
\expandafter\def\csname BAval@state.dance.keep.unresolved\endcsname{84}
\expandafter\def\csname BAval@state.dance.keep.unknown\endcsname{1}
\expandafter\def\csname BAval@tick.dance.f159.keep.iou\endcsname{0.99}
\expandafter\def\csname BAval@tick.dance.f159.keep.state\endcsname{C}
\expandafter\def\csname BAval@tick.dance.f160.keep.iou\endcsname{0.98}
\expandafter\def\csname BAval@tick.dance.f160.keep.state\endcsname{C}
\expandafter\def\csname BAval@tick.dance.f161.keep.iou\endcsname{0.97}
\expandafter\def\csname BAval@tick.dance.f161.keep.state\endcsname{C}
\expandafter\def\csname BAval@tick.dance.f162.keep.iou\endcsname{0.97}
\expandafter\def\csname BAval@tick.dance.f162.keep.state\endcsname{C}
\expandafter\def\csname BAval@tick.dance.f163.keep.iou\endcsname{0.95}
\expandafter\def\csname BAval@tick.dance.f163.keep.state\endcsname{C}
\expandafter\def\csname BAval@tick.dance.f164.keep.iou\endcsname{0.94}
\expandafter\def\csname BAval@tick.dance.f164.keep.state\endcsname{C}
\expandafter\def\csname BAval@tick.dance.f165.keep.iou\endcsname{0.92}
\expandafter\def\csname BAval@tick.dance.f165.keep.state\endcsname{C}
\expandafter\def\csname BAval@tick.dance.f166.keep.iou\endcsname{0.89}
\expandafter\def\csname BAval@tick.dance.f166.keep.state\endcsname{C}
\expandafter\def\csname BAval@tick.dance.f167.keep.iou\endcsname{0.87}
\expandafter\def\csname BAval@tick.dance.f167.keep.state\endcsname{C}
\expandafter\def\csname BAval@tick.dance.f168.keep.iou\endcsname{0.86}
\expandafter\def\csname BAval@tick.dance.f168.keep.state\endcsname{C}
\expandafter\def\csname BAval@tick.dance.f169.keep.iou\endcsname{0.83}
\expandafter\def\csname BAval@tick.dance.f169.keep.state\endcsname{C}
\expandafter\def\csname BAval@tick.dance.f170.keep.iou\endcsname{0.60}
\expandafter\def\csname BAval@tick.dance.f170.keep.state\endcsname{C}
\expandafter\def\csname BAval@tick.dance.f171.keep.iou\endcsname{0.52}
\expandafter\def\csname BAval@tick.dance.f171.keep.state\endcsname{C}
\expandafter\def\csname BAval@tick.dance.f172.keep.iou\endcsname{0.46}
\expandafter\def\csname BAval@tick.dance.f172.keep.state\endcsname{U}
\expandafter\def\csname BAval@tick.dance.f173.keep.iou\endcsname{0.51}
\expandafter\def\csname BAval@tick.dance.f173.keep.state\endcsname{C}
\expandafter\def\csname BAval@tick.dance.f174.keep.iou\endcsname{0.45}
\expandafter\def\csname BAval@tick.dance.f174.keep.state\endcsname{U}
\expandafter\def\csname BAval@tick.dance.f175.keep.iou\endcsname{0.44}
\expandafter\def\csname BAval@tick.dance.f175.keep.state\endcsname{U}
\expandafter\def\csname BAval@tick.dance.f176.keep.iou\endcsname{0.42}
\expandafter\def\csname BAval@tick.dance.f176.keep.state\endcsname{U}
\expandafter\def\csname BAval@tick.dance.f177.keep.iou\endcsname{0.42}
\expandafter\def\csname BAval@tick.dance.f177.keep.state\endcsname{U}
\expandafter\def\csname BAval@tick.dance.f178.keep.iou\endcsname{0.41}
\expandafter\def\csname BAval@tick.dance.f178.keep.state\endcsname{U}
\expandafter\def\csname BAval@tick.dance.f179.keep.iou\endcsname{0.39}
\expandafter\def\csname BAval@tick.dance.f179.keep.state\endcsname{U}
\expandafter\def\csname BAval@tick.dance.f180.keep.iou\endcsname{0.30}
\expandafter\def\csname BAval@tick.dance.f180.keep.state\endcsname{U}
\expandafter\def\csname BAval@tick.dance.f181.keep.iou\endcsname{0.27}
\expandafter\def\csname BAval@tick.dance.f181.keep.state\endcsname{U}
\expandafter\def\csname BAval@tick.dance.f182.keep.iou\endcsname{0.19}
\expandafter\def\csname BAval@tick.dance.f182.keep.state\endcsname{U}
\expandafter\def\csname BAval@tick.dance.f183.keep.iou\endcsname{0.14}
\expandafter\def\csname BAval@tick.dance.f183.keep.state\endcsname{U}
\expandafter\def\csname BAval@tick.dance.f184.keep.iou\endcsname{0.10}
\expandafter\def\csname BAval@tick.dance.f184.keep.state\endcsname{U}
\expandafter\def\csname BAval@tick.dance.f185.keep.iou\endcsname{0.08}
\expandafter\def\csname BAval@tick.dance.f185.keep.state\endcsname{W}
\expandafter\def\csname BAval@tick.dance.f186.keep.iou\endcsname{0.06}
\expandafter\def\csname BAval@tick.dance.f186.keep.state\endcsname{W}
\expandafter\def\csname BAval@tick.dance.f187.keep.iou\endcsname{0.04}
\expandafter\def\csname BAval@tick.dance.f187.keep.state\endcsname{W}
\expandafter\def\csname BAval@tick.dance.f188.keep.iou\endcsname{0.03}
\expandafter\def\csname BAval@tick.dance.f188.keep.state\endcsname{W}
\expandafter\def\csname BAval@tick.dance.f189.keep.iou\endcsname{0.02}
\expandafter\def\csname BAval@tick.dance.f189.keep.state\endcsname{W}
\expandafter\def\csname BAval@tick.dance.f190.keep.iou\endcsname{0.02}
\expandafter\def\csname BAval@tick.dance.f190.keep.state\endcsname{W}
\expandafter\def\csname BAval@tick.dance.f191.keep.iou\endcsname{0.02}
\expandafter\def\csname BAval@tick.dance.f191.keep.state\endcsname{W}
\expandafter\def\csname BAval@tick.dance.f192.keep.iou\endcsname{0.00}
\expandafter\def\csname BAval@tick.dance.f192.keep.state\endcsname{W}
\expandafter\def\csname BAval@tick.dance.f193.keep.iou\endcsname{0.00}
\expandafter\def\csname BAval@tick.dance.f193.keep.state\endcsname{W}
\expandafter\def\csname BAval@tick.dance.f194.keep.iou\endcsname{0.00}
\expandafter\def\csname BAval@tick.dance.f194.keep.state\endcsname{W}
\expandafter\def\csname BAval@tick.dance.f195.keep.iou\endcsname{0.00}
\expandafter\def\csname BAval@tick.dance.f195.keep.state\endcsname{W}
\expandafter\def\csname BAval@tick.dance.f196.keep.iou\endcsname{0.00}
\expandafter\def\csname BAval@tick.dance.f196.keep.state\endcsname{W}
\expandafter\def\csname BAval@tick.dance.f197.keep.iou\endcsname{0.00}
\expandafter\def\csname BAval@tick.dance.f197.keep.state\endcsname{W}
\expandafter\def\csname BAval@tick.dance.f198.keep.iou\endcsname{0.00}
\expandafter\def\csname BAval@tick.dance.f198.keep.state\endcsname{U}
\expandafter\def\csname BAval@tick.dance.f199.keep.iou\endcsname{0.00}
\expandafter\def\csname BAval@tick.dance.f199.keep.state\endcsname{U}
\expandafter\def\csname BAval@tick.dance.f200.keep.iou\endcsname{0.00}
\expandafter\def\csname BAval@tick.dance.f200.keep.state\endcsname{U}
\expandafter\def\csname BAval@tick.dance.f201.keep.iou\endcsname{0.00}
\expandafter\def\csname BAval@tick.dance.f201.keep.state\endcsname{U}
\expandafter\def\csname BAval@tick.dance.f202.keep.iou\endcsname{0.00}
\expandafter\def\csname BAval@tick.dance.f202.keep.state\endcsname{U}
\expandafter\def\csname BAval@tick.dance.f203.keep.iou\endcsname{0.00}
\expandafter\def\csname BAval@tick.dance.f203.keep.state\endcsname{U}
\expandafter\def\csname BAval@tick.dance.f204.keep.iou\endcsname{0.00}
\expandafter\def\csname BAval@tick.dance.f204.keep.state\endcsname{U}
\expandafter\def\csname BAval@tick.dance.f205.keep.iou\endcsname{0.00}
\expandafter\def\csname BAval@tick.dance.f205.keep.state\endcsname{U}
\expandafter\def\csname BAval@tick.dance.f206.keep.iou\endcsname{0.03}
\expandafter\def\csname BAval@tick.dance.f206.keep.state\endcsname{U}
\expandafter\def\csname BAval@tick.dance.f207.keep.iou\endcsname{0.04}
\expandafter\def\csname BAval@tick.dance.f207.keep.state\endcsname{U}
\expandafter\def\csname BAval@tick.dance.f208.keep.iou\endcsname{0.04}
\expandafter\def\csname BAval@tick.dance.f208.keep.state\endcsname{U}
\expandafter\def\csname BAval@tick.dance.f209.keep.iou\endcsname{0.04}
\expandafter\def\csname BAval@tick.dance.f209.keep.state\endcsname{U}
\expandafter\def\csname BAval@tick.dance.f210.keep.iou\endcsname{0.07}
\expandafter\def\csname BAval@tick.dance.f210.keep.state\endcsname{U}
\expandafter\def\csname BAval@tick.dance.f211.keep.iou\endcsname{0.09}
\expandafter\def\csname BAval@tick.dance.f211.keep.state\endcsname{U}
\expandafter\def\csname BAval@tick.dance.f212.keep.iou\endcsname{0.12}
\expandafter\def\csname BAval@tick.dance.f212.keep.state\endcsname{U}
\expandafter\def\csname BAval@tick.dance.f213.keep.iou\endcsname{0.13}
\expandafter\def\csname BAval@tick.dance.f213.keep.state\endcsname{U}
\expandafter\def\csname BAval@tick.dance.f214.keep.iou\endcsname{0.14}
\expandafter\def\csname BAval@tick.dance.f214.keep.state\endcsname{U}
\expandafter\def\csname BAval@tick.dance.f215.keep.iou\endcsname{0.15}
\expandafter\def\csname BAval@tick.dance.f215.keep.state\endcsname{U}
\expandafter\def\csname BAval@tick.dance.f216.keep.iou\endcsname{0.21}
\expandafter\def\csname BAval@tick.dance.f216.keep.state\endcsname{U}
\expandafter\def\csname BAval@tick.dance.f217.keep.iou\endcsname{0.24}
\expandafter\def\csname BAval@tick.dance.f217.keep.state\endcsname{U}
\expandafter\def\csname BAval@tick.dance.f218.keep.iou\endcsname{0.37}
\expandafter\def\csname BAval@tick.dance.f218.keep.state\endcsname{U}
\expandafter\def\csname BAval@tick.dance.f219.keep.iou\endcsname{0.41}
\expandafter\def\csname BAval@tick.dance.f219.keep.state\endcsname{U}
\expandafter\def\csname BAval@tick.dance.f220.keep.iou\endcsname{0.46}
\expandafter\def\csname BAval@tick.dance.f220.keep.state\endcsname{U}
\expandafter\def\csname BAval@tick.dance.f221.keep.iou\endcsname{0.51}
\expandafter\def\csname BAval@tick.dance.f221.keep.state\endcsname{C}
\expandafter\def\csname BAval@tick.dance.f222.keep.iou\endcsname{0.53}
\expandafter\def\csname BAval@tick.dance.f222.keep.state\endcsname{C}
\expandafter\def\csname BAval@tick.dance.f223.keep.iou\endcsname{0.53}
\expandafter\def\csname BAval@tick.dance.f223.keep.state\endcsname{C}
\expandafter\def\csname BAval@tick.dance.f224.keep.iou\endcsname{0.53}
\expandafter\def\csname BAval@tick.dance.f224.keep.state\endcsname{C}
\expandafter\def\csname BAval@tick.dance.f225.keep.iou\endcsname{0.54}
\expandafter\def\csname BAval@tick.dance.f225.keep.state\endcsname{C}
\expandafter\def\csname BAval@tick.dance.f226.keep.iou\endcsname{0.56}
\expandafter\def\csname BAval@tick.dance.f226.keep.state\endcsname{C}
\expandafter\def\csname BAval@tick.dance.f227.keep.iou\endcsname{0.55}
\expandafter\def\csname BAval@tick.dance.f227.keep.state\endcsname{C}
\expandafter\def\csname BAval@tick.dance.f228.keep.iou\endcsname{0.55}
\expandafter\def\csname BAval@tick.dance.f228.keep.state\endcsname{C}
\expandafter\def\csname BAval@tick.dance.f229.keep.iou\endcsname{0.54}
\expandafter\def\csname BAval@tick.dance.f229.keep.state\endcsname{C}
\expandafter\def\csname BAval@tick.dance.f230.keep.iou\endcsname{0.55}
\expandafter\def\csname BAval@tick.dance.f230.keep.state\endcsname{C}
\expandafter\def\csname BAval@tick.dance.f231.keep.iou\endcsname{0.55}
\expandafter\def\csname BAval@tick.dance.f231.keep.state\endcsname{C}
\expandafter\def\csname BAval@tick.dance.f232.keep.iou\endcsname{0.55}
\expandafter\def\csname BAval@tick.dance.f232.keep.state\endcsname{C}
\expandafter\def\csname BAval@tick.dance.f233.keep.iou\endcsname{0.56}
\expandafter\def\csname BAval@tick.dance.f233.keep.state\endcsname{C}
\expandafter\def\csname BAval@tick.dance.f234.keep.iou\endcsname{0.56}
\expandafter\def\csname BAval@tick.dance.f234.keep.state\endcsname{C}
\expandafter\def\csname BAval@tick.dance.f235.keep.iou\endcsname{0.56}
\expandafter\def\csname BAval@tick.dance.f235.keep.state\endcsname{C}
\expandafter\def\csname BAval@tick.dance.f236.keep.iou\endcsname{0.57}
\expandafter\def\csname BAval@tick.dance.f236.keep.state\endcsname{C}
\expandafter\def\csname BAval@tick.dance.f237.keep.iou\endcsname{0.58}
\expandafter\def\csname BAval@tick.dance.f237.keep.state\endcsname{C}
\expandafter\def\csname BAval@tick.dance.f238.keep.iou\endcsname{0.57}
\expandafter\def\csname BAval@tick.dance.f238.keep.state\endcsname{C}
\expandafter\def\csname BAval@tick.dance.f239.keep.iou\endcsname{0.58}
\expandafter\def\csname BAval@tick.dance.f239.keep.state\endcsname{C}
\expandafter\def\csname BAval@tick.dance.f240.keep.iou\endcsname{0.57}
\expandafter\def\csname BAval@tick.dance.f240.keep.state\endcsname{C}
\expandafter\def\csname BAval@tick.dance.f241.keep.iou\endcsname{0.58}
\expandafter\def\csname BAval@tick.dance.f241.keep.state\endcsname{C}
\expandafter\def\csname BAval@tick.dance.f242.keep.iou\endcsname{0.58}
\expandafter\def\csname BAval@tick.dance.f242.keep.state\endcsname{C}
\expandafter\def\csname BAval@tick.dance.f243.keep.iou\endcsname{0.59}
\expandafter\def\csname BAval@tick.dance.f243.keep.state\endcsname{C}
\expandafter\def\csname BAval@tick.dance.f244.keep.iou\endcsname{0.59}
\expandafter\def\csname BAval@tick.dance.f244.keep.state\endcsname{C}
\expandafter\def\csname BAval@tick.dance.f245.keep.iou\endcsname{0.60}
\expandafter\def\csname BAval@tick.dance.f245.keep.state\endcsname{C}
\expandafter\def\csname BAval@tick.dance.f246.keep.iou\endcsname{0.58}
\expandafter\def\csname BAval@tick.dance.f246.keep.state\endcsname{C}
\expandafter\def\csname BAval@tick.dance.f247.keep.iou\endcsname{0.60}
\expandafter\def\csname BAval@tick.dance.f247.keep.state\endcsname{C}
\expandafter\def\csname BAval@tick.dance.f248.keep.iou\endcsname{0.58}
\expandafter\def\csname BAval@tick.dance.f248.keep.state\endcsname{C}
\expandafter\def\csname BAval@tick.dance.f249.keep.iou\endcsname{0.57}
\expandafter\def\csname BAval@tick.dance.f249.keep.state\endcsname{C}
\expandafter\def\csname BAval@tick.dance.f250.keep.iou\endcsname{0.57}
\expandafter\def\csname BAval@tick.dance.f250.keep.state\endcsname{C}
\expandafter\def\csname BAval@tick.dance.f251.keep.iou\endcsname{0.57}
\expandafter\def\csname BAval@tick.dance.f251.keep.state\endcsname{C}
\expandafter\def\csname BAval@tick.dance.f252.keep.iou\endcsname{0.57}
\expandafter\def\csname BAval@tick.dance.f252.keep.state\endcsname{C}
\expandafter\def\csname BAval@tick.dance.f253.keep.iou\endcsname{0.56}
\expandafter\def\csname BAval@tick.dance.f253.keep.state\endcsname{C}
\expandafter\def\csname BAval@tick.dance.f254.keep.iou\endcsname{0.56}
\expandafter\def\csname BAval@tick.dance.f254.keep.state\endcsname{C}
\expandafter\def\csname BAval@tick.dance.f255.keep.iou\endcsname{0.56}
\expandafter\def\csname BAval@tick.dance.f255.keep.state\endcsname{C}
\expandafter\def\csname BAval@tick.dance.f256.keep.iou\endcsname{0.56}
\expandafter\def\csname BAval@tick.dance.f256.keep.state\endcsname{C}
\expandafter\def\csname BAval@tick.dance.f257.keep.iou\endcsname{0.56}
\expandafter\def\csname BAval@tick.dance.f257.keep.state\endcsname{C}
\expandafter\def\csname BAval@tick.dance.f258.keep.iou\endcsname{0.56}
\expandafter\def\csname BAval@tick.dance.f258.keep.state\endcsname{C}
\expandafter\def\csname BAval@tick.dance.f259.keep.iou\endcsname{0.56}
\expandafter\def\csname BAval@tick.dance.f259.keep.state\endcsname{C}
\expandafter\def\csname BAval@tick.dance.f260.keep.iou\endcsname{0.56}
\expandafter\def\csname BAval@tick.dance.f260.keep.state\endcsname{C}
\expandafter\def\csname BAval@tick.dance.f261.keep.iou\endcsname{0.56}
\expandafter\def\csname BAval@tick.dance.f261.keep.state\endcsname{C}
\expandafter\def\csname BAval@tick.dance.f262.keep.iou\endcsname{0.56}
\expandafter\def\csname BAval@tick.dance.f262.keep.state\endcsname{C}
\expandafter\def\csname BAval@tick.dance.f263.keep.iou\endcsname{0.56}
\expandafter\def\csname BAval@tick.dance.f263.keep.state\endcsname{C}
\expandafter\def\csname BAval@tick.dance.f264.keep.iou\endcsname{0.56}
\expandafter\def\csname BAval@tick.dance.f264.keep.state\endcsname{C}
\expandafter\def\csname BAval@tick.dance.f265.keep.iou\endcsname{0.56}
\expandafter\def\csname BAval@tick.dance.f265.keep.state\endcsname{C}
\expandafter\def\csname BAval@tick.dance.f266.keep.iou\endcsname{0.56}
\expandafter\def\csname BAval@tick.dance.f266.keep.state\endcsname{C}
\expandafter\def\csname BAval@tick.dance.f267.keep.iou\endcsname{0.56}
\expandafter\def\csname BAval@tick.dance.f267.keep.state\endcsname{C}
\expandafter\def\csname BAval@tick.dance.f268.keep.iou\endcsname{0.56}
\expandafter\def\csname BAval@tick.dance.f268.keep.state\endcsname{C}
\expandafter\def\csname BAval@tick.dance.f269.keep.iou\endcsname{0.57}
\expandafter\def\csname BAval@tick.dance.f269.keep.state\endcsname{C}
\expandafter\def\csname BAval@tick.dance.f270.keep.iou\endcsname{0.57}
\expandafter\def\csname BAval@tick.dance.f270.keep.state\endcsname{C}
\expandafter\def\csname BAval@tick.dance.f271.keep.iou\endcsname{0.57}
\expandafter\def\csname BAval@tick.dance.f271.keep.state\endcsname{C}
\expandafter\def\csname BAval@tick.dance.f272.keep.iou\endcsname{0.58}
\expandafter\def\csname BAval@tick.dance.f272.keep.state\endcsname{C}
\expandafter\def\csname BAval@tick.dance.f273.keep.iou\endcsname{0.58}
\expandafter\def\csname BAval@tick.dance.f273.keep.state\endcsname{C}
\expandafter\def\csname BAval@tick.dance.f274.keep.iou\endcsname{0.59}
\expandafter\def\csname BAval@tick.dance.f274.keep.state\endcsname{C}
\expandafter\def\csname BAval@tick.dance.f275.keep.iou\endcsname{0.60}
\expandafter\def\csname BAval@tick.dance.f275.keep.state\endcsname{C}
\expandafter\def\csname BAval@tick.dance.f276.keep.iou\endcsname{0.59}
\expandafter\def\csname BAval@tick.dance.f276.keep.state\endcsname{C}
\expandafter\def\csname BAval@tick.dance.f277.keep.iou\endcsname{0.59}
\expandafter\def\csname BAval@tick.dance.f277.keep.state\endcsname{C}
\expandafter\def\csname BAval@tick.dance.f278.keep.iou\endcsname{0.59}
\expandafter\def\csname BAval@tick.dance.f278.keep.state\endcsname{C}
\expandafter\def\csname BAval@tick.dance.f279.keep.iou\endcsname{0.41}
\expandafter\def\csname BAval@tick.dance.f279.keep.state\endcsname{U}
\expandafter\def\csname BAval@tick.dance.f280.keep.iou\endcsname{0.41}
\expandafter\def\csname BAval@tick.dance.f280.keep.state\endcsname{U}
\expandafter\def\csname BAval@tick.dance.f281.keep.iou\endcsname{0.43}
\expandafter\def\csname BAval@tick.dance.f281.keep.state\endcsname{U}
\expandafter\def\csname BAval@tick.dance.f282.keep.iou\endcsname{0.45}
\expandafter\def\csname BAval@tick.dance.f282.keep.state\endcsname{U}
\expandafter\def\csname BAval@tick.dance.f283.keep.iou\endcsname{0.50}
\expandafter\def\csname BAval@tick.dance.f283.keep.state\endcsname{U}
\expandafter\def\csname BAval@tick.dance.f284.keep.iou\endcsname{0.48}
\expandafter\def\csname BAval@tick.dance.f284.keep.state\endcsname{U}
\expandafter\def\csname BAval@tick.dance.f285.keep.iou\endcsname{0.37}
\expandafter\def\csname BAval@tick.dance.f285.keep.state\endcsname{U}
\expandafter\def\csname BAval@tick.dance.f286.keep.iou\endcsname{0.31}
\expandafter\def\csname BAval@tick.dance.f286.keep.state\endcsname{U}
\expandafter\def\csname BAval@tick.dance.f287.keep.iou\endcsname{0.22}
\expandafter\def\csname BAval@tick.dance.f287.keep.state\endcsname{U}
\expandafter\def\csname BAval@tick.dance.f288.keep.iou\endcsname{0.14}
\expandafter\def\csname BAval@tick.dance.f288.keep.state\endcsname{U}
\expandafter\def\csname BAval@tick.dance.f289.keep.iou\endcsname{0.09}
\expandafter\def\csname BAval@tick.dance.f289.keep.state\endcsname{U}
\expandafter\def\csname BAval@tick.dance.f290.keep.iou\endcsname{0.08}
\expandafter\def\csname BAval@tick.dance.f290.keep.state\endcsname{U}
\expandafter\def\csname BAval@tick.dance.f291.keep.iou\endcsname{0.01}
\expandafter\def\csname BAval@tick.dance.f291.keep.state\endcsname{U}
\expandafter\def\csname BAval@tick.dance.f292.keep.iou\endcsname{0.00}
\expandafter\def\csname BAval@tick.dance.f292.keep.state\endcsname{U}
\expandafter\def\csname BAval@tick.dance.f293.keep.iou\endcsname{0.00}
\expandafter\def\csname BAval@tick.dance.f293.keep.state\endcsname{W}
\expandafter\def\csname BAval@tick.dance.f294.keep.iou\endcsname{0.00}
\expandafter\def\csname BAval@tick.dance.f294.keep.state\endcsname{UNKNOWN}
\expandafter\def\csname BAval@tick.dance.f295.keep.iou\endcsname{0.00}
\expandafter\def\csname BAval@tick.dance.f295.keep.state\endcsname{W}
\expandafter\def\csname BAval@tick.dance.f296.keep.iou\endcsname{0.00}
\expandafter\def\csname BAval@tick.dance.f296.keep.state\endcsname{W}
\expandafter\def\csname BAval@tick.dance.f297.keep.iou\endcsname{0.00}
\expandafter\def\csname BAval@tick.dance.f297.keep.state\endcsname{W}
\expandafter\def\csname BAval@tick.dance.f298.keep.iou\endcsname{0.00}
\expandafter\def\csname BAval@tick.dance.f298.keep.state\endcsname{U}
\expandafter\def\csname BAval@tick.dance.f299.keep.iou\endcsname{0.00}
\expandafter\def\csname BAval@tick.dance.f299.keep.state\endcsname{U}
\expandafter\def\csname BAval@tick.dance.f300.keep.iou\endcsname{0.00}
\expandafter\def\csname BAval@tick.dance.f300.keep.state\endcsname{U}
\expandafter\def\csname BAval@tick.dance.f301.keep.iou\endcsname{0.00}
\expandafter\def\csname BAval@tick.dance.f301.keep.state\endcsname{U}
\expandafter\def\csname BAval@tick.dance.f302.keep.iou\endcsname{0.00}
\expandafter\def\csname BAval@tick.dance.f302.keep.state\endcsname{U}
\expandafter\def\csname BAval@tick.dance.f303.keep.iou\endcsname{0.00}
\expandafter\def\csname BAval@tick.dance.f303.keep.state\endcsname{U}
\expandafter\def\csname BAval@tick.dance.f304.keep.iou\endcsname{0.00}
\expandafter\def\csname BAval@tick.dance.f304.keep.state\endcsname{U}
\expandafter\def\csname BAval@tick.dance.f305.keep.iou\endcsname{0.00}
\expandafter\def\csname BAval@tick.dance.f305.keep.state\endcsname{U}
\expandafter\def\csname BAval@tick.dance.f306.keep.iou\endcsname{0.00}
\expandafter\def\csname BAval@tick.dance.f306.keep.state\endcsname{U}
\expandafter\def\csname BAval@tick.dance.f307.keep.iou\endcsname{0.00}
\expandafter\def\csname BAval@tick.dance.f307.keep.state\endcsname{U}
\expandafter\def\csname BAval@tick.dance.f308.keep.iou\endcsname{0.00}
\expandafter\def\csname BAval@tick.dance.f308.keep.state\endcsname{U}
\expandafter\def\csname BAval@tick.dance.f309.keep.iou\endcsname{0.00}
\expandafter\def\csname BAval@tick.dance.f309.keep.state\endcsname{U}
\expandafter\def\csname BAval@tick.dance.f310.keep.iou\endcsname{0.00}
\expandafter\def\csname BAval@tick.dance.f310.keep.state\endcsname{U}
\expandafter\def\csname BAval@tick.dance.f311.keep.iou\endcsname{0.00}
\expandafter\def\csname BAval@tick.dance.f311.keep.state\endcsname{U}
\expandafter\def\csname BAval@tick.dance.f312.keep.iou\endcsname{0.00}
\expandafter\def\csname BAval@tick.dance.f312.keep.state\endcsname{U}
\expandafter\def\csname BAval@tick.dance.f313.keep.iou\endcsname{0.00}
\expandafter\def\csname BAval@tick.dance.f313.keep.state\endcsname{U}
\expandafter\def\csname BAval@tick.dance.f314.keep.iou\endcsname{0.00}
\expandafter\def\csname BAval@tick.dance.f314.keep.state\endcsname{U}
\expandafter\def\csname BAval@tick.dance.f315.keep.iou\endcsname{0.00}
\expandafter\def\csname BAval@tick.dance.f315.keep.state\endcsname{U}
\expandafter\def\csname BAval@tick.dance.f316.keep.iou\endcsname{0.00}
\expandafter\def\csname BAval@tick.dance.f316.keep.state\endcsname{U}
\expandafter\def\csname BAval@tick.dance.f317.keep.iou\endcsname{0.00}
\expandafter\def\csname BAval@tick.dance.f317.keep.state\endcsname{W}
\expandafter\def\csname BAval@tick.dance.f318.keep.iou\endcsname{0.00}
\expandafter\def\csname BAval@tick.dance.f318.keep.state\endcsname{W}
\expandafter\def\csname BAval@tick.dance.f319.keep.iou\endcsname{0.00}
\expandafter\def\csname BAval@tick.dance.f319.keep.state\endcsname{U}
\expandafter\def\csname BAval@tick.dance.f320.keep.iou\endcsname{0.00}
\expandafter\def\csname BAval@tick.dance.f320.keep.state\endcsname{W}
\expandafter\def\csname BAval@tick.dance.f321.keep.iou\endcsname{0.00}
\expandafter\def\csname BAval@tick.dance.f321.keep.state\endcsname{W}
\expandafter\def\csname BAval@tick.dance.f322.keep.iou\endcsname{0.00}
\expandafter\def\csname BAval@tick.dance.f322.keep.state\endcsname{W}
\expandafter\def\csname BAval@tick.dance.f323.keep.iou\endcsname{0.00}
\expandafter\def\csname BAval@tick.dance.f323.keep.state\endcsname{W}
\expandafter\def\csname BAval@tick.dance.f324.keep.iou\endcsname{0.00}
\expandafter\def\csname BAval@tick.dance.f324.keep.state\endcsname{U}
\expandafter\def\csname BAval@tick.dance.f325.keep.iou\endcsname{0.00}
\expandafter\def\csname BAval@tick.dance.f325.keep.state\endcsname{U}
\expandafter\def\csname BAval@tick.dance.f326.keep.iou\endcsname{0.00}
\expandafter\def\csname BAval@tick.dance.f326.keep.state\endcsname{U}
\expandafter\def\csname BAval@tick.dance.f327.keep.iou\endcsname{0.00}
\expandafter\def\csname BAval@tick.dance.f327.keep.state\endcsname{U}
\expandafter\def\csname BAval@tick.dance.f328.keep.iou\endcsname{0.00}
\expandafter\def\csname BAval@tick.dance.f328.keep.state\endcsname{U}
\expandafter\def\csname BAval@tick.dance.f329.keep.iou\endcsname{0.00}
\expandafter\def\csname BAval@tick.dance.f329.keep.state\endcsname{U}
\expandafter\def\csname BAval@tick.dance.f330.keep.iou\endcsname{0.00}
\expandafter\def\csname BAval@tick.dance.f330.keep.state\endcsname{U}
\expandafter\def\csname BAval@tick.dance.f331.keep.iou\endcsname{0.00}
\expandafter\def\csname BAval@tick.dance.f331.keep.state\endcsname{U}
\expandafter\def\csname BAval@tick.dance.f332.keep.iou\endcsname{0.00}
\expandafter\def\csname BAval@tick.dance.f332.keep.state\endcsname{U}
\expandafter\def\csname BAval@tick.dance.f333.keep.iou\endcsname{0.00}
\expandafter\def\csname BAval@tick.dance.f333.keep.state\endcsname{U}
\expandafter\def\csname BAval@tick.dance.f334.keep.iou\endcsname{0.00}
\expandafter\def\csname BAval@tick.dance.f334.keep.state\endcsname{U}
\expandafter\def\csname BAval@tick.dance.f335.keep.iou\endcsname{0.00}
\expandafter\def\csname BAval@tick.dance.f335.keep.state\endcsname{U}
\expandafter\def\csname BAval@tick.dance.f336.keep.iou\endcsname{0.00}
\expandafter\def\csname BAval@tick.dance.f336.keep.state\endcsname{U}
\expandafter\def\csname BAval@tick.dance.f337.keep.iou\endcsname{0.00}
\expandafter\def\csname BAval@tick.dance.f337.keep.state\endcsname{U}
\expandafter\def\csname BAval@tick.dance.f338.keep.iou\endcsname{0.00}
\expandafter\def\csname BAval@tick.dance.f338.keep.state\endcsname{U}
\expandafter\def\csname BAval@state.dance.bind.correct\endcsname{78}
\expandafter\def\csname BAval@state.dance.bind.wrong\endcsname{23}
\expandafter\def\csname BAval@state.dance.bind.unresolved\endcsname{79}
\expandafter\def\csname BAval@state.dance.bind.unknown\endcsname{0}
\expandafter\def\csname BAval@tick.dance.f159.bind.iou\endcsname{0.99}
\expandafter\def\csname BAval@tick.dance.f159.bind.state\endcsname{C}
\expandafter\def\csname BAval@tick.dance.f160.bind.iou\endcsname{0.98}
\expandafter\def\csname BAval@tick.dance.f160.bind.state\endcsname{C}
\expandafter\def\csname BAval@tick.dance.f161.bind.iou\endcsname{0.97}
\expandafter\def\csname BAval@tick.dance.f161.bind.state\endcsname{C}
\expandafter\def\csname BAval@tick.dance.f162.bind.iou\endcsname{0.97}
\expandafter\def\csname BAval@tick.dance.f162.bind.state\endcsname{C}
\expandafter\def\csname BAval@tick.dance.f163.bind.iou\endcsname{0.95}
\expandafter\def\csname BAval@tick.dance.f163.bind.state\endcsname{C}
\expandafter\def\csname BAval@tick.dance.f164.bind.iou\endcsname{0.94}
\expandafter\def\csname BAval@tick.dance.f164.bind.state\endcsname{C}
\expandafter\def\csname BAval@tick.dance.f165.bind.iou\endcsname{0.92}
\expandafter\def\csname BAval@tick.dance.f165.bind.state\endcsname{C}
\expandafter\def\csname BAval@tick.dance.f166.bind.iou\endcsname{0.89}
\expandafter\def\csname BAval@tick.dance.f166.bind.state\endcsname{C}
\expandafter\def\csname BAval@tick.dance.f167.bind.iou\endcsname{0.87}
\expandafter\def\csname BAval@tick.dance.f167.bind.state\endcsname{C}
\expandafter\def\csname BAval@tick.dance.f168.bind.iou\endcsname{0.86}
\expandafter\def\csname BAval@tick.dance.f168.bind.state\endcsname{C}
\expandafter\def\csname BAval@tick.dance.f169.bind.iou\endcsname{0.83}
\expandafter\def\csname BAval@tick.dance.f169.bind.state\endcsname{C}
\expandafter\def\csname BAval@tick.dance.f170.bind.iou\endcsname{0.61}
\expandafter\def\csname BAval@tick.dance.f170.bind.state\endcsname{C}
\expandafter\def\csname BAval@tick.dance.f171.bind.iou\endcsname{0.52}
\expandafter\def\csname BAval@tick.dance.f171.bind.state\endcsname{C}
\expandafter\def\csname BAval@tick.dance.f172.bind.iou\endcsname{0.46}
\expandafter\def\csname BAval@tick.dance.f172.bind.state\endcsname{U}
\expandafter\def\csname BAval@tick.dance.f173.bind.iou\endcsname{0.51}
\expandafter\def\csname BAval@tick.dance.f173.bind.state\endcsname{C}
\expandafter\def\csname BAval@tick.dance.f174.bind.iou\endcsname{0.45}
\expandafter\def\csname BAval@tick.dance.f174.bind.state\endcsname{U}
\expandafter\def\csname BAval@tick.dance.f175.bind.iou\endcsname{0.44}
\expandafter\def\csname BAval@tick.dance.f175.bind.state\endcsname{U}
\expandafter\def\csname BAval@tick.dance.f176.bind.iou\endcsname{0.42}
\expandafter\def\csname BAval@tick.dance.f176.bind.state\endcsname{U}
\expandafter\def\csname BAval@tick.dance.f177.bind.iou\endcsname{0.42}
\expandafter\def\csname BAval@tick.dance.f177.bind.state\endcsname{U}
\expandafter\def\csname BAval@tick.dance.f178.bind.iou\endcsname{0.41}
\expandafter\def\csname BAval@tick.dance.f178.bind.state\endcsname{U}
\expandafter\def\csname BAval@tick.dance.f179.bind.iou\endcsname{0.39}
\expandafter\def\csname BAval@tick.dance.f179.bind.state\endcsname{U}
\expandafter\def\csname BAval@tick.dance.f180.bind.iou\endcsname{0.29}
\expandafter\def\csname BAval@tick.dance.f180.bind.state\endcsname{U}
\expandafter\def\csname BAval@tick.dance.f181.bind.iou\endcsname{0.27}
\expandafter\def\csname BAval@tick.dance.f181.bind.state\endcsname{U}
\expandafter\def\csname BAval@tick.dance.f182.bind.iou\endcsname{0.19}
\expandafter\def\csname BAval@tick.dance.f182.bind.state\endcsname{U}
\expandafter\def\csname BAval@tick.dance.f183.bind.iou\endcsname{0.14}
\expandafter\def\csname BAval@tick.dance.f183.bind.state\endcsname{U}
\expandafter\def\csname BAval@tick.dance.f184.bind.iou\endcsname{0.10}
\expandafter\def\csname BAval@tick.dance.f184.bind.state\endcsname{U}
\expandafter\def\csname BAval@tick.dance.f185.bind.iou\endcsname{0.08}
\expandafter\def\csname BAval@tick.dance.f185.bind.state\endcsname{W}
\expandafter\def\csname BAval@tick.dance.f186.bind.iou\endcsname{0.06}
\expandafter\def\csname BAval@tick.dance.f186.bind.state\endcsname{W}
\expandafter\def\csname BAval@tick.dance.f187.bind.iou\endcsname{0.04}
\expandafter\def\csname BAval@tick.dance.f187.bind.state\endcsname{W}
\expandafter\def\csname BAval@tick.dance.f188.bind.iou\endcsname{0.03}
\expandafter\def\csname BAval@tick.dance.f188.bind.state\endcsname{W}
\expandafter\def\csname BAval@tick.dance.f189.bind.iou\endcsname{0.02}
\expandafter\def\csname BAval@tick.dance.f189.bind.state\endcsname{W}
\expandafter\def\csname BAval@tick.dance.f190.bind.iou\endcsname{0.02}
\expandafter\def\csname BAval@tick.dance.f190.bind.state\endcsname{W}
\expandafter\def\csname BAval@tick.dance.f191.bind.iou\endcsname{0.02}
\expandafter\def\csname BAval@tick.dance.f191.bind.state\endcsname{W}
\expandafter\def\csname BAval@tick.dance.f192.bind.iou\endcsname{0.00}
\expandafter\def\csname BAval@tick.dance.f192.bind.state\endcsname{W}
\expandafter\def\csname BAval@tick.dance.f193.bind.iou\endcsname{0.00}
\expandafter\def\csname BAval@tick.dance.f193.bind.state\endcsname{W}
\expandafter\def\csname BAval@tick.dance.f194.bind.iou\endcsname{0.00}
\expandafter\def\csname BAval@tick.dance.f194.bind.state\endcsname{W}
\expandafter\def\csname BAval@tick.dance.f195.bind.iou\endcsname{0.00}
\expandafter\def\csname BAval@tick.dance.f195.bind.state\endcsname{W}
\expandafter\def\csname BAval@tick.dance.f196.bind.iou\endcsname{0.00}
\expandafter\def\csname BAval@tick.dance.f196.bind.state\endcsname{W}
\expandafter\def\csname BAval@tick.dance.f197.bind.iou\endcsname{0.00}
\expandafter\def\csname BAval@tick.dance.f197.bind.state\endcsname{W}
\expandafter\def\csname BAval@tick.dance.f198.bind.iou\endcsname{0.00}
\expandafter\def\csname BAval@tick.dance.f198.bind.state\endcsname{U}
\expandafter\def\csname BAval@tick.dance.f199.bind.iou\endcsname{0.00}
\expandafter\def\csname BAval@tick.dance.f199.bind.state\endcsname{U}
\expandafter\def\csname BAval@tick.dance.f200.bind.iou\endcsname{0.00}
\expandafter\def\csname BAval@tick.dance.f200.bind.state\endcsname{U}
\expandafter\def\csname BAval@tick.dance.f201.bind.iou\endcsname{0.00}
\expandafter\def\csname BAval@tick.dance.f201.bind.state\endcsname{U}
\expandafter\def\csname BAval@tick.dance.f202.bind.iou\endcsname{0.00}
\expandafter\def\csname BAval@tick.dance.f202.bind.state\endcsname{U}
\expandafter\def\csname BAval@tick.dance.f203.bind.iou\endcsname{0.00}
\expandafter\def\csname BAval@tick.dance.f203.bind.state\endcsname{U}
\expandafter\def\csname BAval@tick.dance.f204.bind.iou\endcsname{0.00}
\expandafter\def\csname BAval@tick.dance.f204.bind.state\endcsname{U}
\expandafter\def\csname BAval@tick.dance.f205.bind.iou\endcsname{0.00}
\expandafter\def\csname BAval@tick.dance.f205.bind.state\endcsname{U}
\expandafter\def\csname BAval@tick.dance.f206.bind.iou\endcsname{0.03}
\expandafter\def\csname BAval@tick.dance.f206.bind.state\endcsname{U}
\expandafter\def\csname BAval@tick.dance.f207.bind.iou\endcsname{0.04}
\expandafter\def\csname BAval@tick.dance.f207.bind.state\endcsname{U}
\expandafter\def\csname BAval@tick.dance.f208.bind.iou\endcsname{0.04}
\expandafter\def\csname BAval@tick.dance.f208.bind.state\endcsname{U}
\expandafter\def\csname BAval@tick.dance.f209.bind.iou\endcsname{0.05}
\expandafter\def\csname BAval@tick.dance.f209.bind.state\endcsname{U}
\expandafter\def\csname BAval@tick.dance.f210.bind.iou\endcsname{0.07}
\expandafter\def\csname BAval@tick.dance.f210.bind.state\endcsname{U}
\expandafter\def\csname BAval@tick.dance.f211.bind.iou\endcsname{0.09}
\expandafter\def\csname BAval@tick.dance.f211.bind.state\endcsname{U}
\expandafter\def\csname BAval@tick.dance.f212.bind.iou\endcsname{0.12}
\expandafter\def\csname BAval@tick.dance.f212.bind.state\endcsname{U}
\expandafter\def\csname BAval@tick.dance.f213.bind.iou\endcsname{0.13}
\expandafter\def\csname BAval@tick.dance.f213.bind.state\endcsname{U}
\expandafter\def\csname BAval@tick.dance.f214.bind.iou\endcsname{0.14}
\expandafter\def\csname BAval@tick.dance.f214.bind.state\endcsname{U}
\expandafter\def\csname BAval@tick.dance.f215.bind.iou\endcsname{0.15}
\expandafter\def\csname BAval@tick.dance.f215.bind.state\endcsname{U}
\expandafter\def\csname BAval@tick.dance.f216.bind.iou\endcsname{0.21}
\expandafter\def\csname BAval@tick.dance.f216.bind.state\endcsname{U}
\expandafter\def\csname BAval@tick.dance.f217.bind.iou\endcsname{0.24}
\expandafter\def\csname BAval@tick.dance.f217.bind.state\endcsname{U}
\expandafter\def\csname BAval@tick.dance.f218.bind.iou\endcsname{0.36}
\expandafter\def\csname BAval@tick.dance.f218.bind.state\endcsname{U}
\expandafter\def\csname BAval@tick.dance.f219.bind.iou\endcsname{0.41}
\expandafter\def\csname BAval@tick.dance.f219.bind.state\endcsname{U}
\expandafter\def\csname BAval@tick.dance.f220.bind.iou\endcsname{0.46}
\expandafter\def\csname BAval@tick.dance.f220.bind.state\endcsname{U}
\expandafter\def\csname BAval@tick.dance.f221.bind.iou\endcsname{0.51}
\expandafter\def\csname BAval@tick.dance.f221.bind.state\endcsname{C}
\expandafter\def\csname BAval@tick.dance.f222.bind.iou\endcsname{0.53}
\expandafter\def\csname BAval@tick.dance.f222.bind.state\endcsname{C}
\expandafter\def\csname BAval@tick.dance.f223.bind.iou\endcsname{0.53}
\expandafter\def\csname BAval@tick.dance.f223.bind.state\endcsname{C}
\expandafter\def\csname BAval@tick.dance.f224.bind.iou\endcsname{0.53}
\expandafter\def\csname BAval@tick.dance.f224.bind.state\endcsname{C}
\expandafter\def\csname BAval@tick.dance.f225.bind.iou\endcsname{0.54}
\expandafter\def\csname BAval@tick.dance.f225.bind.state\endcsname{C}
\expandafter\def\csname BAval@tick.dance.f226.bind.iou\endcsname{0.56}
\expandafter\def\csname BAval@tick.dance.f226.bind.state\endcsname{C}
\expandafter\def\csname BAval@tick.dance.f227.bind.iou\endcsname{0.55}
\expandafter\def\csname BAval@tick.dance.f227.bind.state\endcsname{C}
\expandafter\def\csname BAval@tick.dance.f228.bind.iou\endcsname{0.54}
\expandafter\def\csname BAval@tick.dance.f228.bind.state\endcsname{C}
\expandafter\def\csname BAval@tick.dance.f229.bind.iou\endcsname{0.53}
\expandafter\def\csname BAval@tick.dance.f229.bind.state\endcsname{C}
\expandafter\def\csname BAval@tick.dance.f230.bind.iou\endcsname{0.55}
\expandafter\def\csname BAval@tick.dance.f230.bind.state\endcsname{C}
\expandafter\def\csname BAval@tick.dance.f231.bind.iou\endcsname{0.55}
\expandafter\def\csname BAval@tick.dance.f231.bind.state\endcsname{C}
\expandafter\def\csname BAval@tick.dance.f232.bind.iou\endcsname{0.55}
\expandafter\def\csname BAval@tick.dance.f232.bind.state\endcsname{C}
\expandafter\def\csname BAval@tick.dance.f233.bind.iou\endcsname{0.56}
\expandafter\def\csname BAval@tick.dance.f233.bind.state\endcsname{C}
\expandafter\def\csname BAval@tick.dance.f234.bind.iou\endcsname{0.56}
\expandafter\def\csname BAval@tick.dance.f234.bind.state\endcsname{C}
\expandafter\def\csname BAval@tick.dance.f235.bind.iou\endcsname{0.56}
\expandafter\def\csname BAval@tick.dance.f235.bind.state\endcsname{C}
\expandafter\def\csname BAval@tick.dance.f236.bind.iou\endcsname{0.57}
\expandafter\def\csname BAval@tick.dance.f236.bind.state\endcsname{C}
\expandafter\def\csname BAval@tick.dance.f237.bind.iou\endcsname{0.58}
\expandafter\def\csname BAval@tick.dance.f237.bind.state\endcsname{C}
\expandafter\def\csname BAval@tick.dance.f238.bind.iou\endcsname{0.57}
\expandafter\def\csname BAval@tick.dance.f238.bind.state\endcsname{C}
\expandafter\def\csname BAval@tick.dance.f239.bind.iou\endcsname{0.58}
\expandafter\def\csname BAval@tick.dance.f239.bind.state\endcsname{C}
\expandafter\def\csname BAval@tick.dance.f240.bind.iou\endcsname{0.57}
\expandafter\def\csname BAval@tick.dance.f240.bind.state\endcsname{C}
\expandafter\def\csname BAval@tick.dance.f241.bind.iou\endcsname{0.58}
\expandafter\def\csname BAval@tick.dance.f241.bind.state\endcsname{C}
\expandafter\def\csname BAval@tick.dance.f242.bind.iou\endcsname{0.58}
\expandafter\def\csname BAval@tick.dance.f242.bind.state\endcsname{C}
\expandafter\def\csname BAval@tick.dance.f243.bind.iou\endcsname{0.58}
\expandafter\def\csname BAval@tick.dance.f243.bind.state\endcsname{C}
\expandafter\def\csname BAval@tick.dance.f244.bind.iou\endcsname{0.59}
\expandafter\def\csname BAval@tick.dance.f244.bind.state\endcsname{C}
\expandafter\def\csname BAval@tick.dance.f245.bind.iou\endcsname{0.59}
\expandafter\def\csname BAval@tick.dance.f245.bind.state\endcsname{C}
\expandafter\def\csname BAval@tick.dance.f246.bind.iou\endcsname{0.58}
\expandafter\def\csname BAval@tick.dance.f246.bind.state\endcsname{C}
\expandafter\def\csname BAval@tick.dance.f247.bind.iou\endcsname{0.60}
\expandafter\def\csname BAval@tick.dance.f247.bind.state\endcsname{C}
\expandafter\def\csname BAval@tick.dance.f248.bind.iou\endcsname{0.58}
\expandafter\def\csname BAval@tick.dance.f248.bind.state\endcsname{C}
\expandafter\def\csname BAval@tick.dance.f249.bind.iou\endcsname{0.57}
\expandafter\def\csname BAval@tick.dance.f249.bind.state\endcsname{C}
\expandafter\def\csname BAval@tick.dance.f250.bind.iou\endcsname{0.57}
\expandafter\def\csname BAval@tick.dance.f250.bind.state\endcsname{C}
\expandafter\def\csname BAval@tick.dance.f251.bind.iou\endcsname{0.57}
\expandafter\def\csname BAval@tick.dance.f251.bind.state\endcsname{C}
\expandafter\def\csname BAval@tick.dance.f252.bind.iou\endcsname{0.57}
\expandafter\def\csname BAval@tick.dance.f252.bind.state\endcsname{C}
\expandafter\def\csname BAval@tick.dance.f253.bind.iou\endcsname{0.56}
\expandafter\def\csname BAval@tick.dance.f253.bind.state\endcsname{C}
\expandafter\def\csname BAval@tick.dance.f254.bind.iou\endcsname{0.56}
\expandafter\def\csname BAval@tick.dance.f254.bind.state\endcsname{C}
\expandafter\def\csname BAval@tick.dance.f255.bind.iou\endcsname{0.56}
\expandafter\def\csname BAval@tick.dance.f255.bind.state\endcsname{C}
\expandafter\def\csname BAval@tick.dance.f256.bind.iou\endcsname{0.56}
\expandafter\def\csname BAval@tick.dance.f256.bind.state\endcsname{C}
\expandafter\def\csname BAval@tick.dance.f257.bind.iou\endcsname{0.56}
\expandafter\def\csname BAval@tick.dance.f257.bind.state\endcsname{C}
\expandafter\def\csname BAval@tick.dance.f258.bind.iou\endcsname{0.56}
\expandafter\def\csname BAval@tick.dance.f258.bind.state\endcsname{C}
\expandafter\def\csname BAval@tick.dance.f259.bind.iou\endcsname{0.56}
\expandafter\def\csname BAval@tick.dance.f259.bind.state\endcsname{C}
\expandafter\def\csname BAval@tick.dance.f260.bind.iou\endcsname{0.56}
\expandafter\def\csname BAval@tick.dance.f260.bind.state\endcsname{C}
\expandafter\def\csname BAval@tick.dance.f261.bind.iou\endcsname{0.56}
\expandafter\def\csname BAval@tick.dance.f261.bind.state\endcsname{C}
\expandafter\def\csname BAval@tick.dance.f262.bind.iou\endcsname{0.55}
\expandafter\def\csname BAval@tick.dance.f262.bind.state\endcsname{C}
\expandafter\def\csname BAval@tick.dance.f263.bind.iou\endcsname{0.55}
\expandafter\def\csname BAval@tick.dance.f263.bind.state\endcsname{C}
\expandafter\def\csname BAval@tick.dance.f264.bind.iou\endcsname{0.55}
\expandafter\def\csname BAval@tick.dance.f264.bind.state\endcsname{C}
\expandafter\def\csname BAval@tick.dance.f265.bind.iou\endcsname{0.56}
\expandafter\def\csname BAval@tick.dance.f265.bind.state\endcsname{C}
\expandafter\def\csname BAval@tick.dance.f266.bind.iou\endcsname{0.56}
\expandafter\def\csname BAval@tick.dance.f266.bind.state\endcsname{C}
\expandafter\def\csname BAval@tick.dance.f267.bind.iou\endcsname{0.55}
\expandafter\def\csname BAval@tick.dance.f267.bind.state\endcsname{C}
\expandafter\def\csname BAval@tick.dance.f268.bind.iou\endcsname{0.55}
\expandafter\def\csname BAval@tick.dance.f268.bind.state\endcsname{C}
\expandafter\def\csname BAval@tick.dance.f269.bind.iou\endcsname{0.56}
\expandafter\def\csname BAval@tick.dance.f269.bind.state\endcsname{C}
\expandafter\def\csname BAval@tick.dance.f270.bind.iou\endcsname{0.56}
\expandafter\def\csname BAval@tick.dance.f270.bind.state\endcsname{C}
\expandafter\def\csname BAval@tick.dance.f271.bind.iou\endcsname{0.57}
\expandafter\def\csname BAval@tick.dance.f271.bind.state\endcsname{C}
\expandafter\def\csname BAval@tick.dance.f272.bind.iou\endcsname{0.57}
\expandafter\def\csname BAval@tick.dance.f272.bind.state\endcsname{C}
\expandafter\def\csname BAval@tick.dance.f273.bind.iou\endcsname{0.58}
\expandafter\def\csname BAval@tick.dance.f273.bind.state\endcsname{C}
\expandafter\def\csname BAval@tick.dance.f274.bind.iou\endcsname{0.59}
\expandafter\def\csname BAval@tick.dance.f274.bind.state\endcsname{C}
\expandafter\def\csname BAval@tick.dance.f275.bind.iou\endcsname{0.60}
\expandafter\def\csname BAval@tick.dance.f275.bind.state\endcsname{C}
\expandafter\def\csname BAval@tick.dance.f276.bind.iou\endcsname{0.59}
\expandafter\def\csname BAval@tick.dance.f276.bind.state\endcsname{C}
\expandafter\def\csname BAval@tick.dance.f277.bind.iou\endcsname{0.59}
\expandafter\def\csname BAval@tick.dance.f277.bind.state\endcsname{C}
\expandafter\def\csname BAval@tick.dance.f278.bind.iou\endcsname{0.59}
\expandafter\def\csname BAval@tick.dance.f278.bind.state\endcsname{C}
\expandafter\def\csname BAval@tick.dance.f279.bind.iou\endcsname{0.52}
\expandafter\def\csname BAval@tick.dance.f279.bind.state\endcsname{C}
\expandafter\def\csname BAval@tick.dance.f280.bind.iou\endcsname{0.52}
\expandafter\def\csname BAval@tick.dance.f280.bind.state\endcsname{C}
\expandafter\def\csname BAval@tick.dance.f281.bind.iou\endcsname{0.54}
\expandafter\def\csname BAval@tick.dance.f281.bind.state\endcsname{C}
\expandafter\def\csname BAval@tick.dance.f282.bind.iou\endcsname{0.57}
\expandafter\def\csname BAval@tick.dance.f282.bind.state\endcsname{C}
\expandafter\def\csname BAval@tick.dance.f283.bind.iou\endcsname{0.62}
\expandafter\def\csname BAval@tick.dance.f283.bind.state\endcsname{C}
\expandafter\def\csname BAval@tick.dance.f284.bind.iou\endcsname{0.59}
\expandafter\def\csname BAval@tick.dance.f284.bind.state\endcsname{C}
\expandafter\def\csname BAval@tick.dance.f285.bind.iou\endcsname{0.46}
\expandafter\def\csname BAval@tick.dance.f285.bind.state\endcsname{U}
\expandafter\def\csname BAval@tick.dance.f286.bind.iou\endcsname{0.40}
\expandafter\def\csname BAval@tick.dance.f286.bind.state\endcsname{U}
\expandafter\def\csname BAval@tick.dance.f287.bind.iou\endcsname{0.29}
\expandafter\def\csname BAval@tick.dance.f287.bind.state\endcsname{U}
\expandafter\def\csname BAval@tick.dance.f288.bind.iou\endcsname{0.20}
\expandafter\def\csname BAval@tick.dance.f288.bind.state\endcsname{U}
\expandafter\def\csname BAval@tick.dance.f289.bind.iou\endcsname{0.15}
\expandafter\def\csname BAval@tick.dance.f289.bind.state\endcsname{U}
\expandafter\def\csname BAval@tick.dance.f290.bind.iou\endcsname{0.13}
\expandafter\def\csname BAval@tick.dance.f290.bind.state\endcsname{U}
\expandafter\def\csname BAval@tick.dance.f291.bind.iou\endcsname{0.05}
\expandafter\def\csname BAval@tick.dance.f291.bind.state\endcsname{U}
\expandafter\def\csname BAval@tick.dance.f292.bind.iou\endcsname{0.03}
\expandafter\def\csname BAval@tick.dance.f292.bind.state\endcsname{U}
\expandafter\def\csname BAval@tick.dance.f293.bind.iou\endcsname{0.00}
\expandafter\def\csname BAval@tick.dance.f293.bind.state\endcsname{W}
\expandafter\def\csname BAval@tick.dance.f294.bind.iou\endcsname{0.00}
\expandafter\def\csname BAval@tick.dance.f294.bind.state\endcsname{W}
\expandafter\def\csname BAval@tick.dance.f295.bind.iou\endcsname{0.00}
\expandafter\def\csname BAval@tick.dance.f295.bind.state\endcsname{W}
\expandafter\def\csname BAval@tick.dance.f296.bind.iou\endcsname{0.00}
\expandafter\def\csname BAval@tick.dance.f296.bind.state\endcsname{W}
\expandafter\def\csname BAval@tick.dance.f297.bind.iou\endcsname{0.00}
\expandafter\def\csname BAval@tick.dance.f297.bind.state\endcsname{W}
\expandafter\def\csname BAval@tick.dance.f298.bind.iou\endcsname{0.00}
\expandafter\def\csname BAval@tick.dance.f298.bind.state\endcsname{W}
\expandafter\def\csname BAval@tick.dance.f299.bind.iou\endcsname{0.00}
\expandafter\def\csname BAval@tick.dance.f299.bind.state\endcsname{U}
\expandafter\def\csname BAval@tick.dance.f300.bind.iou\endcsname{0.00}
\expandafter\def\csname BAval@tick.dance.f300.bind.state\endcsname{U}
\expandafter\def\csname BAval@tick.dance.f301.bind.iou\endcsname{0.00}
\expandafter\def\csname BAval@tick.dance.f301.bind.state\endcsname{U}
\expandafter\def\csname BAval@tick.dance.f302.bind.iou\endcsname{0.00}
\expandafter\def\csname BAval@tick.dance.f302.bind.state\endcsname{U}
\expandafter\def\csname BAval@tick.dance.f303.bind.iou\endcsname{0.00}
\expandafter\def\csname BAval@tick.dance.f303.bind.state\endcsname{U}
\expandafter\def\csname BAval@tick.dance.f304.bind.iou\endcsname{0.00}
\expandafter\def\csname BAval@tick.dance.f304.bind.state\endcsname{U}
\expandafter\def\csname BAval@tick.dance.f305.bind.iou\endcsname{0.00}
\expandafter\def\csname BAval@tick.dance.f305.bind.state\endcsname{U}
\expandafter\def\csname BAval@tick.dance.f306.bind.iou\endcsname{0.00}
\expandafter\def\csname BAval@tick.dance.f306.bind.state\endcsname{U}
\expandafter\def\csname BAval@tick.dance.f307.bind.iou\endcsname{0.00}
\expandafter\def\csname BAval@tick.dance.f307.bind.state\endcsname{U}
\expandafter\def\csname BAval@tick.dance.f308.bind.iou\endcsname{0.00}
\expandafter\def\csname BAval@tick.dance.f308.bind.state\endcsname{U}
\expandafter\def\csname BAval@tick.dance.f309.bind.iou\endcsname{0.00}
\expandafter\def\csname BAval@tick.dance.f309.bind.state\endcsname{U}
\expandafter\def\csname BAval@tick.dance.f310.bind.iou\endcsname{0.00}
\expandafter\def\csname BAval@tick.dance.f310.bind.state\endcsname{U}
\expandafter\def\csname BAval@tick.dance.f311.bind.iou\endcsname{0.00}
\expandafter\def\csname BAval@tick.dance.f311.bind.state\endcsname{U}
\expandafter\def\csname BAval@tick.dance.f312.bind.iou\endcsname{0.00}
\expandafter\def\csname BAval@tick.dance.f312.bind.state\endcsname{U}
\expandafter\def\csname BAval@tick.dance.f313.bind.iou\endcsname{0.00}
\expandafter\def\csname BAval@tick.dance.f313.bind.state\endcsname{U}
\expandafter\def\csname BAval@tick.dance.f314.bind.iou\endcsname{0.00}
\expandafter\def\csname BAval@tick.dance.f314.bind.state\endcsname{U}
\expandafter\def\csname BAval@tick.dance.f315.bind.iou\endcsname{0.00}
\expandafter\def\csname BAval@tick.dance.f315.bind.state\endcsname{U}
\expandafter\def\csname BAval@tick.dance.f316.bind.iou\endcsname{0.00}
\expandafter\def\csname BAval@tick.dance.f316.bind.state\endcsname{U}
\expandafter\def\csname BAval@tick.dance.f317.bind.iou\endcsname{0.00}
\expandafter\def\csname BAval@tick.dance.f317.bind.state\endcsname{W}
\expandafter\def\csname BAval@tick.dance.f318.bind.iou\endcsname{0.00}
\expandafter\def\csname BAval@tick.dance.f318.bind.state\endcsname{W}
\expandafter\def\csname BAval@tick.dance.f319.bind.iou\endcsname{0.00}
\expandafter\def\csname BAval@tick.dance.f319.bind.state\endcsname{U}
\expandafter\def\csname BAval@tick.dance.f320.bind.iou\endcsname{0.00}
\expandafter\def\csname BAval@tick.dance.f320.bind.state\endcsname{U}
\expandafter\def\csname BAval@tick.dance.f321.bind.iou\endcsname{0.00}
\expandafter\def\csname BAval@tick.dance.f321.bind.state\endcsname{W}
\expandafter\def\csname BAval@tick.dance.f322.bind.iou\endcsname{0.00}
\expandafter\def\csname BAval@tick.dance.f322.bind.state\endcsname{W}
\expandafter\def\csname BAval@tick.dance.f323.bind.iou\endcsname{0.00}
\expandafter\def\csname BAval@tick.dance.f323.bind.state\endcsname{U}
\expandafter\def\csname BAval@tick.dance.f324.bind.iou\endcsname{0.00}
\expandafter\def\csname BAval@tick.dance.f324.bind.state\endcsname{U}
\expandafter\def\csname BAval@tick.dance.f325.bind.iou\endcsname{0.00}
\expandafter\def\csname BAval@tick.dance.f325.bind.state\endcsname{U}
\expandafter\def\csname BAval@tick.dance.f326.bind.iou\endcsname{0.00}
\expandafter\def\csname BAval@tick.dance.f326.bind.state\endcsname{U}
\expandafter\def\csname BAval@tick.dance.f327.bind.iou\endcsname{0.00}
\expandafter\def\csname BAval@tick.dance.f327.bind.state\endcsname{U}
\expandafter\def\csname BAval@tick.dance.f328.bind.iou\endcsname{0.00}
\expandafter\def\csname BAval@tick.dance.f328.bind.state\endcsname{U}
\expandafter\def\csname BAval@tick.dance.f329.bind.iou\endcsname{0.00}
\expandafter\def\csname BAval@tick.dance.f329.bind.state\endcsname{U}
\expandafter\def\csname BAval@tick.dance.f330.bind.iou\endcsname{0.00}
\expandafter\def\csname BAval@tick.dance.f330.bind.state\endcsname{U}
\expandafter\def\csname BAval@tick.dance.f331.bind.iou\endcsname{0.00}
\expandafter\def\csname BAval@tick.dance.f331.bind.state\endcsname{U}
\expandafter\def\csname BAval@tick.dance.f332.bind.iou\endcsname{0.00}
\expandafter\def\csname BAval@tick.dance.f332.bind.state\endcsname{U}
\expandafter\def\csname BAval@tick.dance.f333.bind.iou\endcsname{0.00}
\expandafter\def\csname BAval@tick.dance.f333.bind.state\endcsname{U}
\expandafter\def\csname BAval@tick.dance.f334.bind.iou\endcsname{0.00}
\expandafter\def\csname BAval@tick.dance.f334.bind.state\endcsname{U}
\expandafter\def\csname BAval@tick.dance.f335.bind.iou\endcsname{0.00}
\expandafter\def\csname BAval@tick.dance.f335.bind.state\endcsname{U}
\expandafter\def\csname BAval@tick.dance.f336.bind.iou\endcsname{0.00}
\expandafter\def\csname BAval@tick.dance.f336.bind.state\endcsname{U}
\expandafter\def\csname BAval@tick.dance.f337.bind.iou\endcsname{0.00}
\expandafter\def\csname BAval@tick.dance.f337.bind.state\endcsname{U}
\expandafter\def\csname BAval@tick.dance.f338.bind.iou\endcsname{0.00}
\expandafter\def\csname BAval@tick.dance.f338.bind.state\endcsname{U}
\expandafter\def\csname BAval@pair.quad.dam.joint\endcsname{72}
\expandafter\def\csname BAval@pair.quad.dam.agree\endcsname{68}
\expandafter\def\csname BAval@pair.quad.dam.other\endcsname{4}
\expandafter\def\csname BAval@pair.quad.dam.unknown\endcsname{18}
\expandafter\def\csname BAval@pair.quad.dam.C.C\endcsname{1}
\expandafter\def\csname BAval@pair.quad.dam.C.W\endcsname{0}
\expandafter\def\csname BAval@pair.quad.dam.C.U\endcsname{0}
\expandafter\def\csname BAval@pair.quad.dam.C.UNKNOWN\endcsname{0}
\expandafter\def\csname BAval@pair.quad.dam.W.C\endcsname{0}
\expandafter\def\csname BAval@pair.quad.dam.W.W\endcsname{9}
\expandafter\def\csname BAval@pair.quad.dam.W.U\endcsname{3}
\expandafter\def\csname BAval@pair.quad.dam.W.UNKNOWN\endcsname{0}
\expandafter\def\csname BAval@pair.quad.dam.U.C\endcsname{0}
\expandafter\def\csname BAval@pair.quad.dam.U.W\endcsname{1}
\expandafter\def\csname BAval@pair.quad.dam.U.U\endcsname{58}
\expandafter\def\csname BAval@pair.quad.dam.U.UNKNOWN\endcsname{0}
\expandafter\def\csname BAval@pair.quad.dam.UNKNOWN.C\endcsname{0}
\expandafter\def\csname BAval@pair.quad.dam.UNKNOWN.W\endcsname{0}
\expandafter\def\csname BAval@pair.quad.dam.UNKNOWN.U\endcsname{0}
\expandafter\def\csname BAval@pair.quad.dam.UNKNOWN.UNKNOWN\endcsname{18}
\expandafter\def\csname BAval@pair.quad.keep.joint\endcsname{72}
\expandafter\def\csname BAval@pair.quad.keep.agree\endcsname{72}
\expandafter\def\csname BAval@pair.quad.keep.other\endcsname{0}
\expandafter\def\csname BAval@pair.quad.keep.unknown\endcsname{18}
\expandafter\def\csname BAval@pair.quad.keep.C.C\endcsname{1}
\expandafter\def\csname BAval@pair.quad.keep.C.W\endcsname{0}
\expandafter\def\csname BAval@pair.quad.keep.C.U\endcsname{0}
\expandafter\def\csname BAval@pair.quad.keep.C.UNKNOWN\endcsname{0}
\expandafter\def\csname BAval@pair.quad.keep.W.C\endcsname{0}
\expandafter\def\csname BAval@pair.quad.keep.W.W\endcsname{12}
\expandafter\def\csname BAval@pair.quad.keep.W.U\endcsname{0}
\expandafter\def\csname BAval@pair.quad.keep.W.UNKNOWN\endcsname{0}
\expandafter\def\csname BAval@pair.quad.keep.U.C\endcsname{0}
\expandafter\def\csname BAval@pair.quad.keep.U.W\endcsname{0}
\expandafter\def\csname BAval@pair.quad.keep.U.U\endcsname{59}
\expandafter\def\csname BAval@pair.quad.keep.U.UNKNOWN\endcsname{0}
\expandafter\def\csname BAval@pair.quad.keep.UNKNOWN.C\endcsname{0}
\expandafter\def\csname BAval@pair.quad.keep.UNKNOWN.W\endcsname{0}
\expandafter\def\csname BAval@pair.quad.keep.UNKNOWN.U\endcsname{0}
\expandafter\def\csname BAval@pair.quad.keep.UNKNOWN.UNKNOWN\endcsname{18}
\expandafter\def\csname BAval@pair.dance.dam.joint\endcsname{180}
\expandafter\def\csname BAval@pair.dance.dam.agree\endcsname{177}
\expandafter\def\csname BAval@pair.dance.dam.other\endcsname{3}
\expandafter\def\csname BAval@pair.dance.dam.unknown\endcsname{0}
\expandafter\def\csname BAval@pair.dance.dam.C.C\endcsname{78}
\expandafter\def\csname BAval@pair.dance.dam.C.W\endcsname{0}
\expandafter\def\csname BAval@pair.dance.dam.C.U\endcsname{0}
\expandafter\def\csname BAval@pair.dance.dam.C.UNKNOWN\endcsname{0}
\expandafter\def\csname BAval@pair.dance.dam.W.C\endcsname{0}
\expandafter\def\csname BAval@pair.dance.dam.W.W\endcsname{20}
\expandafter\def\csname BAval@pair.dance.dam.W.U\endcsname{3}
\expandafter\def\csname BAval@pair.dance.dam.W.UNKNOWN\endcsname{0}
\expandafter\def\csname BAval@pair.dance.dam.U.C\endcsname{0}
\expandafter\def\csname BAval@pair.dance.dam.U.W\endcsname{0}
\expandafter\def\csname BAval@pair.dance.dam.U.U\endcsname{79}
\expandafter\def\csname BAval@pair.dance.dam.U.UNKNOWN\endcsname{0}
\expandafter\def\csname BAval@pair.dance.dam.UNKNOWN.C\endcsname{0}
\expandafter\def\csname BAval@pair.dance.dam.UNKNOWN.W\endcsname{0}
\expandafter\def\csname BAval@pair.dance.dam.UNKNOWN.U\endcsname{0}
\expandafter\def\csname BAval@pair.dance.dam.UNKNOWN.UNKNOWN\endcsname{0}
\expandafter\def\csname BAval@pair.dance.keep.joint\endcsname{179}
\expandafter\def\csname BAval@pair.dance.keep.agree\endcsname{170}
\expandafter\def\csname BAval@pair.dance.keep.other\endcsname{9}
\expandafter\def\csname BAval@pair.dance.keep.unknown\endcsname{1}
\expandafter\def\csname BAval@pair.dance.keep.C.C\endcsname{72}
\expandafter\def\csname BAval@pair.dance.keep.C.W\endcsname{0}
\expandafter\def\csname BAval@pair.dance.keep.C.U\endcsname{6}
\expandafter\def\csname BAval@pair.dance.keep.C.UNKNOWN\endcsname{0}
\expandafter\def\csname BAval@pair.dance.keep.W.C\endcsname{0}
\expandafter\def\csname BAval@pair.dance.keep.W.W\endcsname{21}
\expandafter\def\csname BAval@pair.dance.keep.W.U\endcsname{1}
\expandafter\def\csname BAval@pair.dance.keep.W.UNKNOWN\endcsname{1}
\expandafter\def\csname BAval@pair.dance.keep.U.C\endcsname{0}
\expandafter\def\csname BAval@pair.dance.keep.U.W\endcsname{2}
\expandafter\def\csname BAval@pair.dance.keep.U.U\endcsname{77}
\expandafter\def\csname BAval@pair.dance.keep.U.UNKNOWN\endcsname{0}
\expandafter\def\csname BAval@pair.dance.keep.UNKNOWN.C\endcsname{0}
\expandafter\def\csname BAval@pair.dance.keep.UNKNOWN.W\endcsname{0}
\expandafter\def\csname BAval@pair.dance.keep.UNKNOWN.U\endcsname{0}
\expandafter\def\csname BAval@pair.dance.keep.UNKNOWN.UNKNOWN\endcsname{0}
\expandafter\def\csname BAval@pair.dam.joint\endcsname{252}
\expandafter\def\csname BAval@pair.dam.agree\endcsname{245}
\expandafter\def\csname BAval@pair.dam.other\endcsname{7}
\expandafter\def\csname BAval@pair.dam.unknown\endcsname{18}
\expandafter\def\csname BAval@pair.dam.C.C\endcsname{79}
\expandafter\def\csname BAval@pair.dam.C.W\endcsname{0}
\expandafter\def\csname BAval@pair.dam.C.U\endcsname{0}
\expandafter\def\csname BAval@pair.dam.C.UNKNOWN\endcsname{0}
\expandafter\def\csname BAval@pair.dam.W.C\endcsname{0}
\expandafter\def\csname BAval@pair.dam.W.W\endcsname{29}
\expandafter\def\csname BAval@pair.dam.W.U\endcsname{6}
\expandafter\def\csname BAval@pair.dam.W.UNKNOWN\endcsname{0}
\expandafter\def\csname BAval@pair.dam.U.C\endcsname{0}
\expandafter\def\csname BAval@pair.dam.U.W\endcsname{1}
\expandafter\def\csname BAval@pair.dam.U.U\endcsname{137}
\expandafter\def\csname BAval@pair.dam.U.UNKNOWN\endcsname{0}
\expandafter\def\csname BAval@pair.dam.UNKNOWN.C\endcsname{0}
\expandafter\def\csname BAval@pair.dam.UNKNOWN.W\endcsname{0}
\expandafter\def\csname BAval@pair.dam.UNKNOWN.U\endcsname{0}
\expandafter\def\csname BAval@pair.dam.UNKNOWN.UNKNOWN\endcsname{18}
\expandafter\def\csname BAval@pair.keep.joint\endcsname{251}
\expandafter\def\csname BAval@pair.keep.agree\endcsname{242}
\expandafter\def\csname BAval@pair.keep.other\endcsname{9}
\expandafter\def\csname BAval@pair.keep.unknown\endcsname{19}
\expandafter\def\csname BAval@pair.keep.C.C\endcsname{73}
\expandafter\def\csname BAval@pair.keep.C.W\endcsname{0}
\expandafter\def\csname BAval@pair.keep.C.U\endcsname{6}
\expandafter\def\csname BAval@pair.keep.C.UNKNOWN\endcsname{0}
\expandafter\def\csname BAval@pair.keep.W.C\endcsname{0}
\expandafter\def\csname BAval@pair.keep.W.W\endcsname{33}
\expandafter\def\csname BAval@pair.keep.W.U\endcsname{1}
\expandafter\def\csname BAval@pair.keep.W.UNKNOWN\endcsname{1}
\expandafter\def\csname BAval@pair.keep.U.C\endcsname{0}
\expandafter\def\csname BAval@pair.keep.U.W\endcsname{2}
\expandafter\def\csname BAval@pair.keep.U.U\endcsname{136}
\expandafter\def\csname BAval@pair.keep.U.UNKNOWN\endcsname{0}
\expandafter\def\csname BAval@pair.keep.UNKNOWN.C\endcsname{0}
\expandafter\def\csname BAval@pair.keep.UNKNOWN.W\endcsname{0}
\expandafter\def\csname BAval@pair.keep.UNKNOWN.U\endcsname{0}
\expandafter\def\csname BAval@pair.keep.UNKNOWN.UNKNOWN\endcsname{18}
\expandafter\def\csname BAval@rec.six.frames\endcsname{6}
\expandafter\def\csname BAval@rec.six.seconds\endcsname{0.30}
\expandafter\def\csname BAval@rec.six.start\endcsname{279}
\expandafter\def\csname BAval@rec.six.end\endcsname{284}
\expandafter\def\csname BAval@rec.six.anchor\endcsname{282}
\expandafter\def\csname BAval@rec.frame282.dam.iou\endcsname{0.59}
\expandafter\def\csname BAval@rec.frame282.keep.iou\endcsname{0.45}
\expandafter\def\csname BAval@rec.frame282.bind.iou\endcsname{0.57}
\expandafter\def\csname BAval@case.B.f120.frame\endcsname{120}
\expandafter\def\csname BAval@case.B.f120.kcf\endcsname{0.86}
\expandafter\def\csname BAval@case.B.f120.csrt\endcsname{0.66}
\expandafter\def\csname BAval@case.B.f140.frame\endcsname{140}
\expandafter\def\csname BAval@case.B.f140.kcf\endcsname{0.73}
\expandafter\def\csname BAval@case.B.f140.csrt\endcsname{0.62}
\expandafter\def\csname BAval@case.B.kcf.returned\endcsname{40}
\expandafter\def\csname BAval@case.B.kcf.evaluated.steps\endcsname{40}
\expandafter\def\csname BAval@case.B.kcf.mean\endcsname{0.877}
\expandafter\def\csname BAval@case.B.kcf.successes.iou50\endcsname{40}
\expandafter\def\csname BAval@case.B.csrt.returned\endcsname{40}
\expandafter\def\csname BAval@case.B.csrt.evaluated.steps\endcsname{40}
\expandafter\def\csname BAval@case.B.csrt.mean\endcsname{0.716}
\expandafter\def\csname BAval@case.B.csrt.successes.iou50\endcsname{40}
\expandafter\def\csname BAval@case.D.f272.frame\endcsname{272}
\expandafter\def\csname BAval@case.D.f272.kcf\endcsname{0.38}
\expandafter\def\csname BAval@case.D.f272.csrt\endcsname{0.43}
\expandafter\def\csname BAval@case.D.f300.frame\endcsname{300}
\expandafter\def\csname BAval@case.D.f300.kcf\endcsname{Lost}
\expandafter\def\csname BAval@case.D.f300.csrt\endcsname{0.57}
\expandafter\def\csname BAval@case.D.kcf.returned\endcsname{39}
\expandafter\def\csname BAval@case.D.kcf.evaluated.steps\endcsname{60}
\expandafter\def\csname BAval@case.D.csrt.returned\endcsname{60}
\expandafter\def\csname BAval@case.D.csrt.evaluated.steps\endcsname{60}
\expandafter\def\csname BAval@plan.strata.short.episodes\endcsname{120}
\expandafter\def\csname BAval@plan.strata.short.weight\endcsname{0.250}
\expandafter\def\csname BAval@plan.strata.similar.episodes\endcsname{180}
\expandafter\def\csname BAval@plan.strata.similar.weight\endcsname{0.375}
\expandafter\def\csname BAval@plan.strata.long.episodes\endcsname{180}
\expandafter\def\csname BAval@plan.strata.long.weight\endcsname{0.375}
\expandafter\def\csname BAval@plan.train.groups\endcsname{60}
\expandafter\def\csname BAval@plan.train.episodes\endcsname{1200}
\expandafter\def\csname BAval@plan.validation.groups\endcsname{20}
\expandafter\def\csname BAval@plan.validation.episodes\endcsname{200}
\expandafter\def\csname BAval@plan.test.groups\endcsname{40}
\expandafter\def\csname BAval@plan.test.episodes\endcsname{480}
\expandafter\def\csname BAval@t17.r01.axis\endcsname{0}
\expandafter\def\csname BAval@t17.r02.axis\endcsname{0.1}
\expandafter\def\csname BAval@t17.r03.axis\endcsname{0.25}
\expandafter\def\csname BAval@t17.r04.axis\endcsname{0.5}
\expandafter\def\csname BAval@t17.r05.axis\endcsname{1}
\expandafter\def\csname BAval@t17.r06.axis\endcsname{2}
\expandafter\def\csname BAval@t17.r07.axis\endcsname{0.5}
\expandafter\def\csname BAval@t17.r08.axis\endcsname{0.75}
\expandafter\def\csname BAval@t17.r09.axis\endcsname{1}
\expandafter\def\csname BAval@t17.r10.axis\endcsname{1.25}
\expandafter\def\csname BAval@t17.r11.axis\endcsname{1.5}
\expandafter\def\csname BAval@t17.r12.axis\endcsname{2}
\expandafter\def\csname BAval@t05.r01.axis\endcsname{0}
\expandafter\def\csname BAval@t05.r02.axis\endcsname{0.1}
\expandafter\def\csname BAval@t05.r03.axis\endcsname{0.25}
\expandafter\def\csname BAval@t05.r04.axis\endcsname{0.5}
\expandafter\def\csname BAval@t05.r05.axis\endcsname{1.0}
\expandafter\def\csname BAval@t05.r06.axis\endcsname{2.0}
\expandafter\def\csname BAval@t06.r01.axis\endcsname{0.5}
\expandafter\def\csname BAval@t06.r02.axis\endcsname{0.75}
\expandafter\def\csname BAval@t06.r03.axis\endcsname{1.0}
\expandafter\def\csname BAval@t06.r04.axis\endcsname{1.25}
\expandafter\def\csname BAval@t06.r05.axis\endcsname{1.5}
\expandafter\def\csname BAval@t06.r06.axis\endcsname{2.0}
\expandafter\def\csname BAval@t20.r01.axis\endcsname{0.0}
\expandafter\def\csname BAval@t20.r02.axis\endcsname{0.02}
\expandafter\def\csname BAval@t20.r03.axis\endcsname{0.04}
\expandafter\def\csname BAval@t20.r04.axis\endcsname{0.06}
\expandafter\def\csname BAval@t20.r05.axis\endcsname{0.08}
\expandafter\def\csname BAval@t20.r06.axis\endcsname{0.1}
\expandafter\def\csname BAval@t20.r07.axis\endcsname{0.12}
\expandafter\def\csname BAval@t20.r08.axis\endcsname{0.14}
\expandafter\def\csname BAval@t20.r09.axis\endcsname{0.16}
\expandafter\def\csname BAval@t20.r10.axis\endcsname{0.18}
\expandafter\def\csname BAval@t20.r11.axis\endcsname{0.2}
\expandafter\def\csname BAval@t20.r12.axis\endcsname{0.22}
\expandafter\def\csname BAval@t20.r13.axis\endcsname{0.24}
\expandafter\def\csname BAval@t20.r14.axis\endcsname{0.26}
\expandafter\def\csname BAval@t20.r15.axis\endcsname{0.28}
\expandafter\def\csname BAval@t20.r16.axis\endcsname{0.3}
\expandafter\def\csname BAval@t20.r17.axis\endcsname{0.32}
\expandafter\def\csname BAval@t20.r18.axis\endcsname{0.34}
\expandafter\def\csname BAval@t20.r19.axis\endcsname{0.36}
\expandafter\def\csname BAval@t20.r20.axis\endcsname{0.38}
\expandafter\def\csname BAval@t20.r21.axis\endcsname{0.4}
\expandafter\def\csname BAval@t20.r22.axis\endcsname{0.42}
\expandafter\def\csname BAval@t20.r23.axis\endcsname{0.44}
\expandafter\def\csname BAval@t20.r24.axis\endcsname{0.46}
\expandafter\def\csname BAval@t20.r25.axis\endcsname{0.48}
\expandafter\def\csname BAval@t20.r26.axis\endcsname{0.5}
\expandafter\def\csname BAval@t20.r27.axis\endcsname{0.52}
\expandafter\def\csname BAval@t20.r28.axis\endcsname{0.54}
\expandafter\def\csname BAval@t20.r29.axis\endcsname{0.56}
\expandafter\def\csname BAval@t20.r30.axis\endcsname{0.58}
\expandafter\def\csname BAval@t20.r31.axis\endcsname{0.6}
\expandafter\def\csname BAval@t20.r32.axis\endcsname{0.62}
\expandafter\def\csname BAval@t20.r33.axis\endcsname{0.64}
\expandafter\def\csname BAval@t20.r34.axis\endcsname{0.66}
\expandafter\def\csname BAval@t20.r35.axis\endcsname{0.68}
\expandafter\def\csname BAval@t20.r36.axis\endcsname{0.7}
\expandafter\def\csname BAval@t20.r37.axis\endcsname{0.72}
\expandafter\def\csname BAval@t20.r38.axis\endcsname{0.74}
\expandafter\def\csname BAval@t20.r39.axis\endcsname{0.76}
\expandafter\def\csname BAval@t20.r40.axis\endcsname{0.78}
\expandafter\def\csname BAval@t20.r41.axis\endcsname{0.8}
\expandafter\def\csname BAval@t20.r42.axis\endcsname{0.82}
\expandafter\def\csname BAval@t20.r43.axis\endcsname{0.84}
\expandafter\def\csname BAval@t20.r44.axis\endcsname{0.86}
\expandafter\def\csname BAval@t20.r45.axis\endcsname{0.88}
\expandafter\def\csname BAval@t20.r46.axis\endcsname{0.9}
\expandafter\def\csname BAval@t20.r47.axis\endcsname{0.92}
\expandafter\def\csname BAval@t20.r48.axis\endcsname{0.94}
\expandafter\def\csname BAval@t20.r49.axis\endcsname{0.96}
\expandafter\def\csname BAval@t20.r50.axis\endcsname{0.98}
\expandafter\def\csname BAval@t20.r51.axis\endcsname{1.0}
\expandafter\def\csname BAval@t20.r52.axis\endcsname{0.0}
\expandafter\def\csname BAval@t20.r53.axis\endcsname{0.02}
\expandafter\def\csname BAval@t20.r54.axis\endcsname{0.04}
\expandafter\def\csname BAval@t20.r55.axis\endcsname{0.06}
\expandafter\def\csname BAval@t20.r56.axis\endcsname{0.08}
\expandafter\def\csname BAval@t20.r57.axis\endcsname{0.1}
\expandafter\def\csname BAval@t20.r58.axis\endcsname{0.12}
\expandafter\def\csname BAval@t20.r59.axis\endcsname{0.14}
\expandafter\def\csname BAval@t20.r60.axis\endcsname{0.16}
\expandafter\def\csname BAval@t20.r61.axis\endcsname{0.18}
\expandafter\def\csname BAval@t20.r62.axis\endcsname{0.2}
\expandafter\def\csname BAval@t20.r63.axis\endcsname{0.22}
\expandafter\def\csname BAval@t20.r64.axis\endcsname{0.24}
\expandafter\def\csname BAval@t20.r65.axis\endcsname{0.26}
\expandafter\def\csname BAval@t20.r66.axis\endcsname{0.28}
\expandafter\def\csname BAval@t20.r67.axis\endcsname{0.3}
\expandafter\def\csname BAval@t20.r68.axis\endcsname{0.32}
\expandafter\def\csname BAval@t20.r69.axis\endcsname{0.34}
\expandafter\def\csname BAval@t20.r70.axis\endcsname{0.36}
\expandafter\def\csname BAval@t20.r71.axis\endcsname{0.38}
\expandafter\def\csname BAval@t20.r72.axis\endcsname{0.4}
\expandafter\def\csname BAval@t20.r73.axis\endcsname{0.42}
\expandafter\def\csname BAval@t20.r74.axis\endcsname{0.44}
\expandafter\def\csname BAval@t20.r75.axis\endcsname{0.46}
\expandafter\def\csname BAval@t20.r76.axis\endcsname{0.48}
\expandafter\def\csname BAval@t20.r77.axis\endcsname{0.5}
\expandafter\def\csname BAval@t20.r78.axis\endcsname{0.52}
\expandafter\def\csname BAval@t20.r79.axis\endcsname{0.54}
\expandafter\def\csname BAval@t20.r80.axis\endcsname{0.56}
\expandafter\def\csname BAval@t20.r81.axis\endcsname{0.58}
\expandafter\def\csname BAval@t20.r82.axis\endcsname{0.6}
\expandafter\def\csname BAval@t20.r83.axis\endcsname{0.62}
\expandafter\def\csname BAval@t20.r84.axis\endcsname{0.64}
\expandafter\def\csname BAval@t20.r85.axis\endcsname{0.66}
\expandafter\def\csname BAval@t20.r86.axis\endcsname{0.68}
\expandafter\def\csname BAval@t20.r87.axis\endcsname{0.7}
\expandafter\def\csname BAval@t20.r88.axis\endcsname{0.72}
\expandafter\def\csname BAval@t20.r89.axis\endcsname{0.74}
\expandafter\def\csname BAval@t20.r90.axis\endcsname{0.76}
\expandafter\def\csname BAval@t20.r91.axis\endcsname{0.78}
\expandafter\def\csname BAval@t20.r92.axis\endcsname{0.8}
\expandafter\def\csname BAval@t20.r93.axis\endcsname{0.82}
\expandafter\def\csname BAval@t20.r94.axis\endcsname{0.84}
\expandafter\def\csname BAval@t20.r95.axis\endcsname{0.86}
\expandafter\def\csname BAval@t20.r96.axis\endcsname{0.88}
\expandafter\def\csname BAval@t20.r97.axis\endcsname{0.9}
\expandafter\def\csname BAval@t20.r98.axis\endcsname{0.92}
\expandafter\def\csname BAval@t20.r99.axis\endcsname{0.94}
\expandafter\def\csname BAval@t20.r100.axis\endcsname{0.96}
\expandafter\def\csname BAval@t20.r101.axis\endcsname{0.98}
\expandafter\def\csname BAval@t20.r102.axis\endcsname{1.0}
\expandafter\def\csname BAval@t20.r103.axis\endcsname{0.0}
\expandafter\def\csname BAval@t20.r104.axis\endcsname{0.02}
\expandafter\def\csname BAval@t20.r105.axis\endcsname{0.04}
\expandafter\def\csname BAval@t20.r106.axis\endcsname{0.06}
\expandafter\def\csname BAval@t20.r107.axis\endcsname{0.08}
\expandafter\def\csname BAval@t20.r108.axis\endcsname{0.1}
\expandafter\def\csname BAval@t20.r109.axis\endcsname{0.12}
\expandafter\def\csname BAval@t20.r110.axis\endcsname{0.14}
\expandafter\def\csname BAval@t20.r111.axis\endcsname{0.16}
\expandafter\def\csname BAval@t20.r112.axis\endcsname{0.18}
\expandafter\def\csname BAval@t20.r113.axis\endcsname{0.2}
\expandafter\def\csname BAval@t20.r114.axis\endcsname{0.22}
\expandafter\def\csname BAval@t20.r115.axis\endcsname{0.24}
\expandafter\def\csname BAval@t20.r116.axis\endcsname{0.26}
\expandafter\def\csname BAval@t20.r117.axis\endcsname{0.28}
\expandafter\def\csname BAval@t20.r118.axis\endcsname{0.3}
\expandafter\def\csname BAval@t20.r119.axis\endcsname{0.32}
\expandafter\def\csname BAval@t20.r120.axis\endcsname{0.34}
\expandafter\def\csname BAval@t20.r121.axis\endcsname{0.36}
\expandafter\def\csname BAval@t20.r122.axis\endcsname{0.38}
\expandafter\def\csname BAval@t20.r123.axis\endcsname{0.4}
\expandafter\def\csname BAval@t20.r124.axis\endcsname{0.42}
\expandafter\def\csname BAval@t20.r125.axis\endcsname{0.44}
\expandafter\def\csname BAval@t20.r126.axis\endcsname{0.46}
\expandafter\def\csname BAval@t20.r127.axis\endcsname{0.48}
\expandafter\def\csname BAval@t20.r128.axis\endcsname{0.5}
\expandafter\def\csname BAval@t20.r129.axis\endcsname{0.52}
\expandafter\def\csname BAval@t20.r130.axis\endcsname{0.54}
\expandafter\def\csname BAval@t20.r131.axis\endcsname{0.56}
\expandafter\def\csname BAval@t20.r132.axis\endcsname{0.58}
\expandafter\def\csname BAval@t20.r133.axis\endcsname{0.6}
\expandafter\def\csname BAval@t20.r134.axis\endcsname{0.62}
\expandafter\def\csname BAval@t20.r135.axis\endcsname{0.64}
\expandafter\def\csname BAval@t20.r136.axis\endcsname{0.66}
\expandafter\def\csname BAval@t20.r137.axis\endcsname{0.68}
\expandafter\def\csname BAval@t20.r138.axis\endcsname{0.7}
\expandafter\def\csname BAval@t20.r139.axis\endcsname{0.72}
\expandafter\def\csname BAval@t20.r140.axis\endcsname{0.74}
\expandafter\def\csname BAval@t20.r141.axis\endcsname{0.76}
\expandafter\def\csname BAval@t20.r142.axis\endcsname{0.78}
\expandafter\def\csname BAval@t20.r143.axis\endcsname{0.8}
\expandafter\def\csname BAval@t20.r144.axis\endcsname{0.82}
\expandafter\def\csname BAval@t20.r145.axis\endcsname{0.84}
\expandafter\def\csname BAval@t20.r146.axis\endcsname{0.86}
\expandafter\def\csname BAval@t20.r147.axis\endcsname{0.88}
\expandafter\def\csname BAval@t20.r148.axis\endcsname{0.9}
\expandafter\def\csname BAval@t20.r149.axis\endcsname{0.92}
\expandafter\def\csname BAval@t20.r150.axis\endcsname{0.94}
\expandafter\def\csname BAval@t20.r151.axis\endcsname{0.96}
\expandafter\def\csname BAval@t20.r152.axis\endcsname{0.98}
\expandafter\def\csname BAval@t20.r153.axis\endcsname{1.0}
\expandafter\def\csname BAval@t20.r154.axis\endcsname{0.0}
\expandafter\def\csname BAval@t20.r155.axis\endcsname{0.02}
\expandafter\def\csname BAval@t20.r156.axis\endcsname{0.04}
\expandafter\def\csname BAval@t20.r157.axis\endcsname{0.06}
\expandafter\def\csname BAval@t20.r158.axis\endcsname{0.08}
\expandafter\def\csname BAval@t20.r159.axis\endcsname{0.1}
\expandafter\def\csname BAval@t20.r160.axis\endcsname{0.12}
\expandafter\def\csname BAval@t20.r161.axis\endcsname{0.14}
\expandafter\def\csname BAval@t20.r162.axis\endcsname{0.16}
\expandafter\def\csname BAval@t20.r163.axis\endcsname{0.18}
\expandafter\def\csname BAval@t20.r164.axis\endcsname{0.2}
\expandafter\def\csname BAval@t20.r165.axis\endcsname{0.22}
\expandafter\def\csname BAval@t20.r166.axis\endcsname{0.24}
\expandafter\def\csname BAval@t20.r167.axis\endcsname{0.26}
\expandafter\def\csname BAval@t20.r168.axis\endcsname{0.28}
\expandafter\def\csname BAval@t20.r169.axis\endcsname{0.3}
\expandafter\def\csname BAval@t20.r170.axis\endcsname{0.32}
\expandafter\def\csname BAval@t20.r171.axis\endcsname{0.34}
\expandafter\def\csname BAval@t20.r172.axis\endcsname{0.36}
\expandafter\def\csname BAval@t20.r173.axis\endcsname{0.38}
\expandafter\def\csname BAval@t20.r174.axis\endcsname{0.4}
\expandafter\def\csname BAval@t20.r175.axis\endcsname{0.42}
\expandafter\def\csname BAval@t20.r176.axis\endcsname{0.44}
\expandafter\def\csname BAval@t20.r177.axis\endcsname{0.46}
\expandafter\def\csname BAval@t20.r178.axis\endcsname{0.48}
\expandafter\def\csname BAval@t20.r179.axis\endcsname{0.5}
\expandafter\def\csname BAval@t20.r180.axis\endcsname{0.52}
\expandafter\def\csname BAval@t20.r181.axis\endcsname{0.54}
\expandafter\def\csname BAval@t20.r182.axis\endcsname{0.56}
\expandafter\def\csname BAval@t20.r183.axis\endcsname{0.58}
\expandafter\def\csname BAval@t20.r184.axis\endcsname{0.6}
\expandafter\def\csname BAval@t20.r185.axis\endcsname{0.62}
\expandafter\def\csname BAval@t20.r186.axis\endcsname{0.64}
\expandafter\def\csname BAval@t20.r187.axis\endcsname{0.66}
\expandafter\def\csname BAval@t20.r188.axis\endcsname{0.68}
\expandafter\def\csname BAval@t20.r189.axis\endcsname{0.7}
\expandafter\def\csname BAval@t20.r190.axis\endcsname{0.72}
\expandafter\def\csname BAval@t20.r191.axis\endcsname{0.74}
\expandafter\def\csname BAval@t20.r192.axis\endcsname{0.76}
\expandafter\def\csname BAval@t20.r193.axis\endcsname{0.78}
\expandafter\def\csname BAval@t20.r194.axis\endcsname{0.8}
\expandafter\def\csname BAval@t20.r195.axis\endcsname{0.82}
\expandafter\def\csname BAval@t20.r196.axis\endcsname{0.84}
\expandafter\def\csname BAval@t20.r197.axis\endcsname{0.86}
\expandafter\def\csname BAval@t20.r198.axis\endcsname{0.88}
\expandafter\def\csname BAval@t20.r199.axis\endcsname{0.9}
\expandafter\def\csname BAval@t20.r200.axis\endcsname{0.92}
\expandafter\def\csname BAval@t20.r201.axis\endcsname{0.94}
\expandafter\def\csname BAval@t20.r202.axis\endcsname{0.96}
\expandafter\def\csname BAval@t20.r203.axis\endcsname{0.98}
\expandafter\def\csname BAval@t20.r204.axis\endcsname{1.0}
\expandafter\def\csname BAval@t20.r205.axis\endcsname{0.0}
\expandafter\def\csname BAval@t20.r206.axis\endcsname{0.02}
\expandafter\def\csname BAval@t20.r207.axis\endcsname{0.04}
\expandafter\def\csname BAval@t20.r208.axis\endcsname{0.06}
\expandafter\def\csname BAval@t20.r209.axis\endcsname{0.08}
\expandafter\def\csname BAval@t20.r210.axis\endcsname{0.1}
\expandafter\def\csname BAval@t20.r211.axis\endcsname{0.12}
\expandafter\def\csname BAval@t20.r212.axis\endcsname{0.14}
\expandafter\def\csname BAval@t20.r213.axis\endcsname{0.16}
\expandafter\def\csname BAval@t20.r214.axis\endcsname{0.18}
\expandafter\def\csname BAval@t20.r215.axis\endcsname{0.2}
\expandafter\def\csname BAval@t20.r216.axis\endcsname{0.22}
\expandafter\def\csname BAval@t20.r217.axis\endcsname{0.24}
\expandafter\def\csname BAval@t20.r218.axis\endcsname{0.26}
\expandafter\def\csname BAval@t20.r219.axis\endcsname{0.28}
\expandafter\def\csname BAval@t20.r220.axis\endcsname{0.3}
\expandafter\def\csname BAval@t20.r221.axis\endcsname{0.32}
\expandafter\def\csname BAval@t20.r222.axis\endcsname{0.34}
\expandafter\def\csname BAval@t20.r223.axis\endcsname{0.36}
\expandafter\def\csname BAval@t20.r224.axis\endcsname{0.38}
\expandafter\def\csname BAval@t20.r225.axis\endcsname{0.4}
\expandafter\def\csname BAval@t20.r226.axis\endcsname{0.42}
\expandafter\def\csname BAval@t20.r227.axis\endcsname{0.44}
\expandafter\def\csname BAval@t20.r228.axis\endcsname{0.46}
\expandafter\def\csname BAval@t20.r229.axis\endcsname{0.48}
\expandafter\def\csname BAval@t20.r230.axis\endcsname{0.5}
\expandafter\def\csname BAval@t20.r231.axis\endcsname{0.52}
\expandafter\def\csname BAval@t20.r232.axis\endcsname{0.54}
\expandafter\def\csname BAval@t20.r233.axis\endcsname{0.56}
\expandafter\def\csname BAval@t20.r234.axis\endcsname{0.58}
\expandafter\def\csname BAval@t20.r235.axis\endcsname{0.6}
\expandafter\def\csname BAval@t20.r236.axis\endcsname{0.62}
\expandafter\def\csname BAval@t20.r237.axis\endcsname{0.64}
\expandafter\def\csname BAval@t20.r238.axis\endcsname{0.66}
\expandafter\def\csname BAval@t20.r239.axis\endcsname{0.68}
\expandafter\def\csname BAval@t20.r240.axis\endcsname{0.7}
\expandafter\def\csname BAval@t20.r241.axis\endcsname{0.72}
\expandafter\def\csname BAval@t20.r242.axis\endcsname{0.74}
\expandafter\def\csname BAval@t20.r243.axis\endcsname{0.76}
\expandafter\def\csname BAval@t20.r244.axis\endcsname{0.78}
\expandafter\def\csname BAval@t20.r245.axis\endcsname{0.8}
\expandafter\def\csname BAval@t20.r246.axis\endcsname{0.82}
\expandafter\def\csname BAval@t20.r247.axis\endcsname{0.84}
\expandafter\def\csname BAval@t20.r248.axis\endcsname{0.86}
\expandafter\def\csname BAval@t20.r249.axis\endcsname{0.88}
\expandafter\def\csname BAval@t20.r250.axis\endcsname{0.9}
\expandafter\def\csname BAval@t20.r251.axis\endcsname{0.92}
\expandafter\def\csname BAval@t20.r252.axis\endcsname{0.94}
\expandafter\def\csname BAval@t20.r253.axis\endcsname{0.96}
\expandafter\def\csname BAval@t20.r254.axis\endcsname{0.98}
\expandafter\def\csname BAval@t20.r255.axis\endcsname{1.0}
\expandafter\def\csname BAval@t20.r256.axis\endcsname{0.0}
\expandafter\def\csname BAval@t20.r257.axis\endcsname{0.02}
\expandafter\def\csname BAval@t20.r258.axis\endcsname{0.04}
\expandafter\def\csname BAval@t20.r259.axis\endcsname{0.06}
\expandafter\def\csname BAval@t20.r260.axis\endcsname{0.08}
\expandafter\def\csname BAval@t20.r261.axis\endcsname{0.1}
\expandafter\def\csname BAval@t20.r262.axis\endcsname{0.12}
\expandafter\def\csname BAval@t20.r263.axis\endcsname{0.14}
\expandafter\def\csname BAval@t20.r264.axis\endcsname{0.16}
\expandafter\def\csname BAval@t20.r265.axis\endcsname{0.18}
\expandafter\def\csname BAval@t20.r266.axis\endcsname{0.2}
\expandafter\def\csname BAval@t20.r267.axis\endcsname{0.22}
\expandafter\def\csname BAval@t20.r268.axis\endcsname{0.24}
\expandafter\def\csname BAval@t20.r269.axis\endcsname{0.26}
\expandafter\def\csname BAval@t20.r270.axis\endcsname{0.28}
\expandafter\def\csname BAval@t20.r271.axis\endcsname{0.3}
\expandafter\def\csname BAval@t20.r272.axis\endcsname{0.32}
\expandafter\def\csname BAval@t20.r273.axis\endcsname{0.34}
\expandafter\def\csname BAval@t20.r274.axis\endcsname{0.36}
\expandafter\def\csname BAval@t20.r275.axis\endcsname{0.38}
\expandafter\def\csname BAval@t20.r276.axis\endcsname{0.4}
\expandafter\def\csname BAval@t20.r277.axis\endcsname{0.42}
\expandafter\def\csname BAval@t20.r278.axis\endcsname{0.44}
\expandafter\def\csname BAval@t20.r279.axis\endcsname{0.46}
\expandafter\def\csname BAval@t20.r280.axis\endcsname{0.48}
\expandafter\def\csname BAval@t20.r281.axis\endcsname{0.5}
\expandafter\def\csname BAval@t20.r282.axis\endcsname{0.52}
\expandafter\def\csname BAval@t20.r283.axis\endcsname{0.54}
\expandafter\def\csname BAval@t20.r284.axis\endcsname{0.56}
\expandafter\def\csname BAval@t20.r285.axis\endcsname{0.58}
\expandafter\def\csname BAval@t20.r286.axis\endcsname{0.6}
\expandafter\def\csname BAval@t20.r287.axis\endcsname{0.62}
\expandafter\def\csname BAval@t20.r288.axis\endcsname{0.64}
\expandafter\def\csname BAval@t20.r289.axis\endcsname{0.66}
\expandafter\def\csname BAval@t20.r290.axis\endcsname{0.68}
\expandafter\def\csname BAval@t20.r291.axis\endcsname{0.7}
\expandafter\def\csname BAval@t20.r292.axis\endcsname{0.72}
\expandafter\def\csname BAval@t20.r293.axis\endcsname{0.74}
\expandafter\def\csname BAval@t20.r294.axis\endcsname{0.76}
\expandafter\def\csname BAval@t20.r295.axis\endcsname{0.78}
\expandafter\def\csname BAval@t20.r296.axis\endcsname{0.8}
\expandafter\def\csname BAval@t20.r297.axis\endcsname{0.82}
\expandafter\def\csname BAval@t20.r298.axis\endcsname{0.84}
\expandafter\def\csname BAval@t20.r299.axis\endcsname{0.86}
\expandafter\def\csname BAval@t20.r300.axis\endcsname{0.88}
\expandafter\def\csname BAval@t20.r301.axis\endcsname{0.9}
\expandafter\def\csname BAval@t20.r302.axis\endcsname{0.92}
\expandafter\def\csname BAval@t20.r303.axis\endcsname{0.94}
\expandafter\def\csname BAval@t20.r304.axis\endcsname{0.96}
\expandafter\def\csname BAval@t20.r305.axis\endcsname{0.98}
\expandafter\def\csname BAval@t20.r306.axis\endcsname{1.0}
\expandafter\def\csname BAval@ladder.step.law\endcsname{0.5}
\expandafter\def\csname BAval@ladder.step.id\endcsname{3.3}
\expandafter\def\csname BAval@ladder.step.future\endcsname{1.8}
\expandafter\def\csname BAval@ladder.step.zerodelay\endcsname{6.2}
\expandafter\def\csname BAval@ladder.step.fullview\endcsname{3.9}
\expandafter\def\csname BAval@gap.external.abs\endcsname{12.7}
\expandafter\def\csname BAval@diag.late.full\endcsname{75.8}
\expandafter\def\csname BAval@diag.late.ablated\endcsname{67.7}
\expandafter\def\csname BAval@diag.late.drop\endcsname{8.2}
\expandafter\def\csname BAval@diag.early.full\endcsname{87.0}
\expandafter\def\csname BAval@diag.early.ablated\endcsname{85.8}
\expandafter\def\csname BAval@diag.early.drop\endcsname{1.1}
\expandafter\def\csname BAval@diag.corr.full\endcsname{80.1}
\expandafter\def\csname BAval@diag.corr.ablated\endcsname{73.8}
\expandafter\def\csname BAval@diag.corr.drop\endcsname{6.3}
\expandafter\def\csname BAval@diag.indep.full\endcsname{84.6}
\expandafter\def\csname BAval@diag.indep.ablated\endcsname{84.2}
\expandafter\def\csname BAval@diag.indep.drop\endcsname{0.4}
\expandafter\def\csname BAval@svc.direct.sid\endcsname{78.1}
\expandafter\def\csname BAval@svc.recal.sid\endcsname{81.0}
\expandafter\def\csname BAval@svc.retrain.sid\endcsname{81.7}
\expandafter\def\csname BAval@delta.svc.recal\endcsname{2.9}
\expandafter\def\csname BAval@delta.svc.retrain\endcsname{0.6}
\expandafter\def\csname BAval@lambda.sens.range\endcsname{0.7}
\expandafter\def\csname BAval@t24.r01.lambda.w\endcsname{1}
\expandafter\def\csname BAval@t24.r01.lambda.u\endcsname{1}
\expandafter\def\csname BAval@t24.r02.lambda.w\endcsname{2}
\expandafter\def\csname BAval@t24.r02.lambda.u\endcsname{1}
\expandafter\def\csname BAval@t24.r03.lambda.w\endcsname{4}
\expandafter\def\csname BAval@t24.r03.lambda.u\endcsname{1}
\expandafter\def\csname BAval@t24.r04.lambda.w\endcsname{8}
\expandafter\def\csname BAval@t24.r04.lambda.u\endcsname{1}
\expandafter\def\csname BAval@lambda.w\endcsname{4}
\expandafter\def\csname BAval@lambda.u\endcsname{1}
\expandafter\def\csname BAval@weight.gamma.state\endcsname{1.00}
\expandafter\def\csname BAval@weight.gamma.return\endcsname{0.50}
\expandafter\def\csname BAval@weight.gamma.cost\endcsname{0.10}
\expandafter\def\csname BAval@weight.gamma.rank\endcsname{1.00}
\expandafter\def\csname BAval@weight.gamma.calibration\endcsname{0.20}
\expandafter\def\csname BAval@weight.soft.compute.penalty\endcsname{0.01}
\expandafter\def\csname BAval@weight.soft.motion.penalty\endcsname{0.01}
\expandafter\def\csname BAval@weight.uncertainty.weight\endcsname{0.05}
\expandafter\def\csname BAval@clip.quad.dam.sid\endcsname{1.1}
\expandafter\def\csname BAval@clip.quad.dam.wrong\endcsname{11.1}
\expandafter\def\csname BAval@clip.quad.keep.sid\endcsname{1.1}
\expandafter\def\csname BAval@clip.quad.keep.wrong\endcsname{13.3}
\expandafter\def\csname BAval@clip.dance.dam.sid\endcsname{43.3}
\expandafter\def\csname BAval@clip.dance.dam.wrong\endcsname{11.1}
\expandafter\def\csname BAval@clip.dance.keep.sid\endcsname{40.0}
\expandafter\def\csname BAval@clip.dance.keep.wrong\endcsname{12.8}
\expandafter\def\csname BAval@tick.dance.f272.dam.revision\endcsname{1}
\expandafter\def\csname BAval@tick.dance.f272.dam.sourceage\endcsname{5.70}
\expandafter\def\csname BAval@tick.dance.f272.dam.pubage\endcsname{0.25}
\expandafter\def\csname BAval@tick.dance.f272.dam.id\endcsname{5}
\expandafter\def\csname BAval@tick.dance.f272.dam.maxcompiou\endcsname{0.320}
\expandafter\def\csname BAval@tick.dance.f272.keep.revision\endcsname{0}
\expandafter\def\csname BAval@tick.dance.f272.keep.sourceage\endcsname{5.70}
\expandafter\def\csname BAval@tick.dance.f272.keep.pubage\endcsname{5.70}
\expandafter\def\csname BAval@tick.dance.f272.keep.id\endcsname{5}
\expandafter\def\csname BAval@tick.dance.f272.keep.maxcompiou\endcsname{0.342}
\expandafter\def\csname BAval@tick.dance.f272.bind.revision\endcsname{0}
\expandafter\def\csname BAval@tick.dance.f272.bind.sourceage\endcsname{5.70}
\expandafter\def\csname BAval@tick.dance.f272.bind.pubage\endcsname{5.70}
\expandafter\def\csname BAval@tick.dance.f272.bind.id\endcsname{5}
\expandafter\def\csname BAval@tick.dance.f272.bind.maxcompiou\endcsname{0.342}
\expandafter\def\csname BAval@tick.dance.f279.dam.revision\endcsname{1}
\expandafter\def\csname BAval@tick.dance.f279.dam.sourceage\endcsname{6.05}
\expandafter\def\csname BAval@tick.dance.f279.dam.pubage\endcsname{0.60}
\expandafter\def\csname BAval@tick.dance.f279.dam.id\endcsname{5}
\expandafter\def\csname BAval@tick.dance.f279.dam.maxcompiou\endcsname{0.314}
\expandafter\def\csname BAval@tick.dance.f279.keep.revision\endcsname{1}
\expandafter\def\csname BAval@tick.dance.f279.keep.sourceage\endcsname{6.05}
\expandafter\def\csname BAval@tick.dance.f279.keep.pubage\endcsname{0.02}
\expandafter\def\csname BAval@tick.dance.f279.keep.id\endcsname{5}
\expandafter\def\csname BAval@tick.dance.f279.keep.maxcompiou\endcsname{0.278}
\expandafter\def\csname BAval@tick.dance.f279.bind.revision\endcsname{0}
\expandafter\def\csname BAval@tick.dance.f279.bind.sourceage\endcsname{6.05}
\expandafter\def\csname BAval@tick.dance.f279.bind.pubage\endcsname{6.05}
\expandafter\def\csname BAval@tick.dance.f279.bind.id\endcsname{5}
\expandafter\def\csname BAval@tick.dance.f279.bind.maxcompiou\endcsname{0.337}
\expandafter\def\csname BAval@tick.dance.f280.dam.revision\endcsname{1}
\expandafter\def\csname BAval@tick.dance.f280.dam.sourceage\endcsname{6.10}
\expandafter\def\csname BAval@tick.dance.f280.dam.pubage\endcsname{0.65}
\expandafter\def\csname BAval@tick.dance.f280.dam.id\endcsname{5}
\expandafter\def\csname BAval@tick.dance.f280.dam.maxcompiou\endcsname{0.332}
\expandafter\def\csname BAval@tick.dance.f280.keep.revision\endcsname{1}
\expandafter\def\csname BAval@tick.dance.f280.keep.sourceage\endcsname{6.10}
\expandafter\def\csname BAval@tick.dance.f280.keep.pubage\endcsname{0.07}
\expandafter\def\csname BAval@tick.dance.f280.keep.id\endcsname{5}
\expandafter\def\csname BAval@tick.dance.f280.keep.maxcompiou\endcsname{0.293}
\expandafter\def\csname BAval@tick.dance.f280.bind.revision\endcsname{0}
\expandafter\def\csname BAval@tick.dance.f280.bind.sourceage\endcsname{6.10}
\expandafter\def\csname BAval@tick.dance.f280.bind.pubage\endcsname{6.10}
\expandafter\def\csname BAval@tick.dance.f280.bind.id\endcsname{5}
\expandafter\def\csname BAval@tick.dance.f280.bind.maxcompiou\endcsname{0.355}
\expandafter\def\csname BAval@tick.dance.f281.dam.revision\endcsname{1}
\expandafter\def\csname BAval@tick.dance.f281.dam.sourceage\endcsname{6.15}
\expandafter\def\csname BAval@tick.dance.f281.dam.pubage\endcsname{0.70}
\expandafter\def\csname BAval@tick.dance.f281.dam.id\endcsname{5}
\expandafter\def\csname BAval@tick.dance.f281.dam.maxcompiou\endcsname{0.343}
\expandafter\def\csname BAval@tick.dance.f281.keep.revision\endcsname{1}
\expandafter\def\csname BAval@tick.dance.f281.keep.sourceage\endcsname{6.15}
\expandafter\def\csname BAval@tick.dance.f281.keep.pubage\endcsname{0.12}
\expandafter\def\csname BAval@tick.dance.f281.keep.id\endcsname{5}
\expandafter\def\csname BAval@tick.dance.f281.keep.maxcompiou\endcsname{0.301}
\expandafter\def\csname BAval@tick.dance.f281.bind.revision\endcsname{0}
\expandafter\def\csname BAval@tick.dance.f281.bind.sourceage\endcsname{6.15}
\expandafter\def\csname BAval@tick.dance.f281.bind.pubage\endcsname{6.15}
\expandafter\def\csname BAval@tick.dance.f281.bind.id\endcsname{5}
\expandafter\def\csname BAval@tick.dance.f281.bind.maxcompiou\endcsname{0.366}
\expandafter\def\csname BAval@tick.dance.f282.dam.revision\endcsname{1}
\expandafter\def\csname BAval@tick.dance.f282.dam.sourceage\endcsname{6.20}
\expandafter\def\csname BAval@tick.dance.f282.dam.pubage\endcsname{0.75}
\expandafter\def\csname BAval@tick.dance.f282.dam.id\endcsname{5}
\expandafter\def\csname BAval@tick.dance.f282.dam.maxcompiou\endcsname{0.336}
\expandafter\def\csname BAval@tick.dance.f282.keep.revision\endcsname{1}
\expandafter\def\csname BAval@tick.dance.f282.keep.sourceage\endcsname{6.20}
\expandafter\def\csname BAval@tick.dance.f282.keep.pubage\endcsname{0.17}
\expandafter\def\csname BAval@tick.dance.f282.keep.id\endcsname{5}
\expandafter\def\csname BAval@tick.dance.f282.keep.maxcompiou\endcsname{0.292}
\expandafter\def\csname BAval@tick.dance.f282.bind.revision\endcsname{0}
\expandafter\def\csname BAval@tick.dance.f282.bind.sourceage\endcsname{6.20}
\expandafter\def\csname BAval@tick.dance.f282.bind.pubage\endcsname{6.20}
\expandafter\def\csname BAval@tick.dance.f282.bind.id\endcsname{5}
\expandafter\def\csname BAval@tick.dance.f282.bind.maxcompiou\endcsname{0.358}
\expandafter\def\csname BAval@tick.dance.f283.dam.revision\endcsname{1}
\expandafter\def\csname BAval@tick.dance.f283.dam.sourceage\endcsname{6.25}
\expandafter\def\csname BAval@tick.dance.f283.dam.pubage\endcsname{0.80}
\expandafter\def\csname BAval@tick.dance.f283.dam.id\endcsname{5}
\expandafter\def\csname BAval@tick.dance.f283.dam.maxcompiou\endcsname{0.281}
\expandafter\def\csname BAval@tick.dance.f283.keep.revision\endcsname{1}
\expandafter\def\csname BAval@tick.dance.f283.keep.sourceage\endcsname{6.25}
\expandafter\def\csname BAval@tick.dance.f283.keep.pubage\endcsname{0.22}
\expandafter\def\csname BAval@tick.dance.f283.keep.id\endcsname{5}
\expandafter\def\csname BAval@tick.dance.f283.keep.maxcompiou\endcsname{0.226}
\expandafter\def\csname BAval@tick.dance.f283.bind.revision\endcsname{0}
\expandafter\def\csname BAval@tick.dance.f283.bind.sourceage\endcsname{6.25}
\expandafter\def\csname BAval@tick.dance.f283.bind.pubage\endcsname{6.25}
\expandafter\def\csname BAval@tick.dance.f283.bind.id\endcsname{5}
\expandafter\def\csname BAval@tick.dance.f283.bind.maxcompiou\endcsname{0.297}
\expandafter\def\csname BAval@tick.dance.f284.dam.revision\endcsname{1}
\expandafter\def\csname BAval@tick.dance.f284.dam.sourceage\endcsname{6.30}
\expandafter\def\csname BAval@tick.dance.f284.dam.pubage\endcsname{0.85}
\expandafter\def\csname BAval@tick.dance.f284.dam.id\endcsname{5}
\expandafter\def\csname BAval@tick.dance.f284.dam.maxcompiou\endcsname{0.298}
\expandafter\def\csname BAval@tick.dance.f284.keep.revision\endcsname{1}
\expandafter\def\csname BAval@tick.dance.f284.keep.sourceage\endcsname{6.30}
\expandafter\def\csname BAval@tick.dance.f284.keep.pubage\endcsname{0.27}
\expandafter\def\csname BAval@tick.dance.f284.keep.id\endcsname{5}
\expandafter\def\csname BAval@tick.dance.f284.keep.maxcompiou\endcsname{0.242}
\expandafter\def\csname BAval@tick.dance.f284.bind.revision\endcsname{0}
\expandafter\def\csname BAval@tick.dance.f284.bind.sourceage\endcsname{6.30}
\expandafter\def\csname BAval@tick.dance.f284.bind.pubage\endcsname{6.30}
\expandafter\def\csname BAval@tick.dance.f284.bind.id\endcsname{5}
\expandafter\def\csname BAval@tick.dance.f284.bind.maxcompiou\endcsname{0.314}
\expandafter\def\csname BAval@tick.dance.f296.dam.revision\endcsname{1}
\expandafter\def\csname BAval@tick.dance.f296.dam.sourceage\endcsname{6.90}
\expandafter\def\csname BAval@tick.dance.f296.dam.pubage\endcsname{1.45}
\expandafter\def\csname BAval@tick.dance.f296.dam.id\endcsname{5}
\expandafter\def\csname BAval@tick.dance.f296.dam.competitor\endcsname{6}
\expandafter\def\csname BAval@tick.dance.f296.dam.compiou\endcsname{0.822}
\expandafter\def\csname BAval@tick.dance.f296.dam.maxcompiou\endcsname{0.822}
\expandafter\def\csname BAval@tick.dance.f296.keep.revision\endcsname{1}
\expandafter\def\csname BAval@tick.dance.f296.keep.sourceage\endcsname{6.90}
\expandafter\def\csname BAval@tick.dance.f296.keep.pubage\endcsname{0.87}
\expandafter\def\csname BAval@tick.dance.f296.keep.id\endcsname{5}
\expandafter\def\csname BAval@tick.dance.f296.keep.competitor\endcsname{6}
\expandafter\def\csname BAval@tick.dance.f296.keep.compiou\endcsname{0.792}
\expandafter\def\csname BAval@tick.dance.f296.keep.maxcompiou\endcsname{0.792}
\expandafter\def\csname BAval@tick.dance.f296.bind.revision\endcsname{0}
\expandafter\def\csname BAval@tick.dance.f296.bind.sourceage\endcsname{6.90}
\expandafter\def\csname BAval@tick.dance.f296.bind.pubage\endcsname{6.90}
\expandafter\def\csname BAval@tick.dance.f296.bind.id\endcsname{5}
\expandafter\def\csname BAval@tick.dance.f296.bind.competitor\endcsname{6}
\expandafter\def\csname BAval@tick.dance.f296.bind.compiou\endcsname{0.786}
\expandafter\def\csname BAval@tick.dance.f296.bind.maxcompiou\endcsname{0.786}
\expandafter\def\csname BAval@tick.dance.f320.dam.revision\endcsname{1}
\expandafter\def\csname BAval@tick.dance.f320.dam.sourceage\endcsname{8.10}
\expandafter\def\csname BAval@tick.dance.f320.dam.pubage\endcsname{2.65}
\expandafter\def\csname BAval@tick.dance.f320.dam.id\endcsname{5}
\expandafter\def\csname BAval@tick.dance.f320.dam.maxcompiou\endcsname{0.474}
\expandafter\def\csname BAval@tick.dance.f320.keep.revision\endcsname{1}
\expandafter\def\csname BAval@tick.dance.f320.keep.sourceage\endcsname{8.10}
\expandafter\def\csname BAval@tick.dance.f320.keep.pubage\endcsname{2.07}
\expandafter\def\csname BAval@tick.dance.f320.keep.id\endcsname{5}
\expandafter\def\csname BAval@tick.dance.f320.keep.competitor\endcsname{4}
\expandafter\def\csname BAval@tick.dance.f320.keep.compiou\endcsname{0.502}
\expandafter\def\csname BAval@tick.dance.f320.keep.maxcompiou\endcsname{0.502}
\expandafter\def\csname BAval@tick.dance.f320.bind.revision\endcsname{0}
\expandafter\def\csname BAval@tick.dance.f320.bind.sourceage\endcsname{8.10}
\expandafter\def\csname BAval@tick.dance.f320.bind.pubage\endcsname{8.10}
\expandafter\def\csname BAval@tick.dance.f320.bind.id\endcsname{5}
\expandafter\def\csname BAval@tick.dance.f320.bind.maxcompiou\endcsname{0.493}
\expandafter\def\csname BAval@tick.quad.f465.dam.revision\endcsname{1}
\expandafter\def\csname BAval@tick.quad.f465.dam.sourceage\endcsname{5.70}
\expandafter\def\csname BAval@tick.quad.f465.dam.pubage\endcsname{2.25}
\expandafter\def\csname BAval@tick.quad.f465.dam.id\endcsname{59}
\expandafter\def\csname BAval@tick.quad.f465.dam.maxcompiou\endcsname{0.192}
\expandafter\def\csname BAval@tick.quad.f465.keep.revision\endcsname{1}
\expandafter\def\csname BAval@tick.quad.f465.keep.sourceage\endcsname{5.70}
\expandafter\def\csname BAval@tick.quad.f465.keep.pubage\endcsname{0.94}
\expandafter\def\csname BAval@tick.quad.f465.keep.id\endcsname{59}
\expandafter\def\csname BAval@tick.quad.f465.keep.maxcompiou\endcsname{0.232}
\expandafter\def\csname BAval@tick.quad.f465.bind.revision\endcsname{0}
\expandafter\def\csname BAval@tick.quad.f465.bind.sourceage\endcsname{5.70}
\expandafter\def\csname BAval@tick.quad.f465.bind.pubage\endcsname{5.70}
\expandafter\def\csname BAval@tick.quad.f465.bind.id\endcsname{59}
\expandafter\def\csname BAval@tick.quad.f465.bind.maxcompiou\endcsname{0.225}
\expandafter\def\csname BAval@tick.quad.f477.dam.revision\endcsname{1}
\expandafter\def\csname BAval@tick.quad.f477.dam.sourceage\endcsname{6.90}
\expandafter\def\csname BAval@tick.quad.f477.dam.pubage\endcsname{3.45}
\expandafter\def\csname BAval@tick.quad.f477.dam.id\endcsname{59}
\expandafter\def\csname BAval@tick.quad.f477.dam.maxcompiou\endcsname{0.007}
\expandafter\def\csname BAval@tick.quad.f477.keep.revision\endcsname{1}
\expandafter\def\csname BAval@tick.quad.f477.keep.sourceage\endcsname{6.90}
\expandafter\def\csname BAval@tick.quad.f477.keep.pubage\endcsname{2.14}
\expandafter\def\csname BAval@tick.quad.f477.keep.id\endcsname{59}
\expandafter\def\csname BAval@tick.quad.f477.keep.maxcompiou\endcsname{0.030}
\expandafter\def\csname BAval@tick.quad.f477.bind.revision\endcsname{0}
\expandafter\def\csname BAval@tick.quad.f477.bind.sourceage\endcsname{6.90}
\expandafter\def\csname BAval@tick.quad.f477.bind.pubage\endcsname{6.90}
\expandafter\def\csname BAval@tick.quad.f477.bind.id\endcsname{59}
\expandafter\def\csname BAval@tick.quad.f477.bind.maxcompiou\endcsname{0.027}
\expandafter\def\csname BAval@tick.quad.f489.dam.revision\endcsname{2}
\expandafter\def\csname BAval@tick.quad.f489.dam.sourceage\endcsname{4.69}
\expandafter\def\csname BAval@tick.quad.f489.dam.pubage\endcsname{0.44}
\expandafter\def\csname BAval@tick.quad.f489.dam.id\endcsname{59}
\expandafter\def\csname BAval@tick.quad.f489.dam.maxcompiou\endcsname{0.363}
\expandafter\def\csname BAval@tick.quad.f489.keep.revision\endcsname{1}
\expandafter\def\csname BAval@tick.quad.f489.keep.sourceage\endcsname{8.10}
\expandafter\def\csname BAval@tick.quad.f489.keep.pubage\endcsname{3.34}
\expandafter\def\csname BAval@tick.quad.f489.keep.id\endcsname{59}
\expandafter\def\csname BAval@tick.quad.f489.keep.competitor\endcsname{101}
\expandafter\def\csname BAval@tick.quad.f489.keep.compiou\endcsname{0.547}
\expandafter\def\csname BAval@tick.quad.f489.keep.maxcompiou\endcsname{0.547}
\expandafter\def\csname BAval@tick.quad.f489.bind.revision\endcsname{0}
\expandafter\def\csname BAval@tick.quad.f489.bind.sourceage\endcsname{8.10}
\expandafter\def\csname BAval@tick.quad.f489.bind.pubage\endcsname{8.10}
\expandafter\def\csname BAval@tick.quad.f489.bind.id\endcsname{59}
\expandafter\def\csname BAval@tick.quad.f489.bind.competitor\endcsname{101}
\expandafter\def\csname BAval@tick.quad.f489.bind.compiou\endcsname{0.531}
\expandafter\def\csname BAval@tick.quad.f489.bind.maxcompiou\endcsname{0.531}
\expandafter\def\csname BAval@goal.B.f100.x\endcsname{647}
\expandafter\def\csname BAval@goal.B.f100.y\endcsname{438}
\expandafter\def\csname BAval@goal.B.f100.width\endcsname{100}
\expandafter\def\csname BAval@goal.B.f100.height\endcsname{305}
\expandafter\def\csname BAval@goal.B.f120.x\endcsname{676}
\expandafter\def\csname BAval@goal.B.f120.y\endcsname{438}
\expandafter\def\csname BAval@goal.B.f120.width\endcsname{97}
\expandafter\def\csname BAval@goal.B.f120.height\endcsname{318}
\expandafter\def\csname BAval@goal.B.f140.x\endcsname{693}
\expandafter\def\csname BAval@goal.B.f140.y\endcsname{434}
\expandafter\def\csname BAval@goal.B.f140.width\endcsname{109}
\expandafter\def\csname BAval@goal.B.f140.height\endcsname{328}
\expandafter\def\csname BAval@goal.D.f240.x\endcsname{348}
\expandafter\def\csname BAval@goal.D.f240.y\endcsname{202}
\expandafter\def\csname BAval@goal.D.f240.width\endcsname{50}
\expandafter\def\csname BAval@goal.D.f240.height\endcsname{165}
\expandafter\def\csname BAval@goal.D.f272.x\endcsname{324}
\expandafter\def\csname BAval@goal.D.f272.y\endcsname{295}
\expandafter\def\csname BAval@goal.D.f272.width\endcsname{89}
\expandafter\def\csname BAval@goal.D.f272.height\endcsname{242}
\expandafter\def\csname BAval@goal.D.f300.x\endcsname{634}
\expandafter\def\csname BAval@goal.D.f300.y\endcsname{228}
\expandafter\def\csname BAval@goal.D.f300.width\endcsname{69}
\expandafter\def\csname BAval@goal.D.f300.height\endcsname{212}
