# Supplementary material for: BindAdapt: Joint Camera-Computation Scheduling for Persistent Target Identity in PTZ Tracking
Source: arXiv:2611.38995 source file (2026-11-28)
Supplement: Supplementary file 2 [file supp_numbers_update_20261117.tex]

\expandafter\def\csname BAval@t17.r01.dam4sam.chanakya.j\endcsname{80.12}
\expandafter\def\csname BAval@t17.r01.bindadapt\endcsname{84.22}
\expandafter\def\csname BAval@t17.r02.dam4sam.chanakya.j\endcsname{79.36}
\expandafter\def\csname BAval@t17.r02.bindadapt\endcsname{84.09}
\expandafter\def\csname BAval@t17.r03.dam4sam.chanakya.j\endcsname{77.84}
\expandafter\def\csname BAval@t17.r03.bindadapt\endcsname{83.46}
\expandafter\def\csname BAval@t17.r04.dam4sam.chanakya.j\endcsname{75.20}
\expandafter\def\csname BAval@t17.r04.bindadapt\endcsname{82.30}
\expandafter\def\csname BAval@t17.r05.dam4sam.chanakya.j\endcsname{68.46}
\expandafter\def\csname BAval@t17.r05.bindadapt\endcsname{78.13}
\expandafter\def\csname BAval@t17.r06.dam4sam.chanakya.j\endcsname{54.82}
\expandafter\def\csname BAval@t17.r06.bindadapt\endcsname{67.02}
\expandafter\def\csname BAval@delta.sweep.zero\endcsname{4.10}
\expandafter\def\csname BAval@delta.sweep.ref\endcsname{7.10}
\expandafter\def\csname BAval@delta.sweep.two\endcsname{12.20}
\expandafter\def\csname BAval@svc.direct.sid\endcsname{81.34}
\expandafter\def\csname BAval@svc.recal.sid\endcsname{83.62}
\expandafter\def\csname BAval@svc.retrain.sid\endcsname{84.03}
\expandafter\def\csname BAval@delta.svc.recal\endcsname{2.28}
\expandafter\def\csname BAval@delta.svc.retrain\endcsname{0.41}
\expandafter\def\csname BAval@delta.svc.gap\endcsname{2.69}
