# Supplementary material for: BindAdapt: Joint Camera-Computation Scheduling for Persistent Target Identity in PTZ Tracking
Source: arXiv:2611.38995 source file (2026-11-28)
Supplement: Supplementary file 3 [file supp_numbers_v38.tex]

\expandafter\def\csname BAval@sd.ext.advat\endcsname{0.3}
\expandafter\def\csname BAval@sd.ext.oavat\endcsname{0.2}
\expandafter\def\csname BAval@sd.ext.pvt\endcsname{0.4}
\expandafter\def\csname BAval@sd.ext.artrack\endcsname{0.3}
\expandafter\def\csname BAval@sd.ext.chanakya\endcsname{0.6}
\expandafter\def\csname BAval@sd.ext.joint\endcsname{0.8}
\expandafter\def\csname BAval@sd.ext.best\endcsname{0.2}
\expandafter\def\csname BAval@sd.ext.bind\endcsname{0.3}
\expandafter\def\csname BAval@sd.t03.r01\endcsname{0.6}
\expandafter\def\csname BAval@sd.t03.r02\endcsname{0.9}
\expandafter\def\csname BAval@sd.t03.r03\endcsname{0.3}
\expandafter\def\csname BAval@sd.t03.r04\endcsname{0.3}
\expandafter\def\csname BAval@t03.r01.sidx\endcsname{65.9}
\expandafter\def\csname BAval@t03.r02.sidx\endcsname{70.3}
\expandafter\def\csname BAval@t03.r03.sidx\endcsname{77.6}
\expandafter\def\csname BAval@t03.r04.sidx\endcsname{82.3}
\expandafter\def\csname BAval@sd.t04.r01\endcsname{0.3}
\expandafter\def\csname BAval@sd.t04.r02\endcsname{0.2}
\expandafter\def\csname BAval@sd.t04.r03\endcsname{0.2}
\expandafter\def\csname BAval@sd.t04.r04\endcsname{0.9}
\expandafter\def\csname BAval@sd.t04.r05\endcsname{1.1}
\expandafter\def\csname BAval@sd.t04.r06\endcsname{0.3}
\expandafter\def\csname BAval@sd.t04.r07\endcsname{0.3}
\expandafter\def\csname BAval@abl.unc.sid\endcsname{80.5}
\expandafter\def\csname BAval@abl.unc.wrong\endcsname{5.8}
\expandafter\def\csname BAval@abl.unc.t5\endcsname{1.5}
\expandafter\def\csname BAval@abl.unc.drop\endcsname{1.8}
\expandafter\def\csname BAval@sd.abl.unc\endcsname{0.1}
\expandafter\def\csname BAval@abl.imm.sid\endcsname{76.2}
\expandafter\def\csname BAval@abl.imm.wrong\endcsname{7.1}
\expandafter\def\csname BAval@abl.imm.t5\endcsname{1.7}
\expandafter\def\csname BAval@abl.imm.drop\endcsname{6.1}
\expandafter\def\csname BAval@rule.prox.sid\endcsname{73.6}
\expandafter\def\csname BAval@rule.prox.wrong\endcsname{8.0}
\expandafter\def\csname BAval@rule.prox.t5\endcsname{1.8}
\expandafter\def\csname BAval@rule.prox.drop\endcsname{8.7}
\expandafter\def\csname BAval@rule.prox.k\endcsname{1.5}
\expandafter\def\csname BAval@rule.rate.sid\endcsname{71.4}
\expandafter\def\csname BAval@rule.rate.wrong\endcsname{8.8}
\expandafter\def\csname BAval@rule.rate.t5\endcsname{1.6}
\expandafter\def\csname BAval@rule.rate.drop\endcsname{10.9}
\expandafter\def\csname BAval@rule.rate.period\endcsname{0.6}
\expandafter\def\csname BAval@rule.prox.long\endcsname{61.4}
\expandafter\def\csname BAval@rule.rate.long\endcsname{58.9}
\expandafter\def\csname BAval@ci.lo\endcsname{5.1}
\expandafter\def\csname BAval@ci.hi\endcsname{9.0}
\expandafter\def\csname BAval@ci.groups\endcsname{40}
\expandafter\def\csname BAval@ci.resamples\endcsname{10{,}000}
\expandafter\def\csname BAval@idf1.best\endcsname{77.5}
\expandafter\def\csname BAval@idf1.bind\endcsname{83.5}
\expandafter\def\csname BAval@hota.best\endcsname{61.8}
\expandafter\def\csname BAval@hota.bind\endcsname{67.3}
\expandafter\def\csname BAval@tune.configs\endcsname{24}
\expandafter\def\csname BAval@tune.seeds\endcsname{3}
\expandafter\def\csname BAval@tune.groups\endcsname{20}
\expandafter\def\csname BAval@retsweep.episodes\endcsname{243}
\expandafter\def\csname BAval@retsweep.early\endcsname{94.2}
\expandafter\def\csname BAval@retsweep.zero\endcsname{80.7}
\expandafter\def\csname BAval@retsweep.late\endcsname{56.8}
\expandafter\def\csname BAval@attr.dam.total\endcsname{137}
\expandafter\def\csname BAval@attr.dam.after\endcsname{89}
\expandafter\def\csname BAval@attr.dam.pct\endcsname{65.0}
\expandafter\def\csname BAval@attr.keep.total\endcsname{151}
\expandafter\def\csname BAval@attr.keep.after\endcsname{87}
\expandafter\def\csname BAval@attr.keep.pct\endcsname{57.6}
\expandafter\def\csname BAval@attr.best.total\endcsname{97}
\expandafter\def\csname BAval@attr.best.after\endcsname{61}
\expandafter\def\csname BAval@attr.best.pct\endcsname{62.9}
\expandafter\def\csname BAval@attr.bind.total\endcsname{53}
\expandafter\def\csname BAval@attr.bind.after\endcsname{18}
\expandafter\def\csname BAval@attr.bind.pct\endcsname{34.0}
\expandafter\def\csname BAval@plan.mean\endcsname{2.1}
\expandafter\def\csname BAval@plan.p95\endcsname{3.8}
\expandafter\def\csname BAval@plan.decisions\endcsname{10{,}000}
\expandafter\def\csname BAval@plan.limit\endcsname{10}
\expandafter\def\csname BAval@cost.mixformer\endcsname{19.8}
\expandafter\def\csname BAval@cost.hiptrack\endcsname{27.5}
\expandafter\def\csname BAval@cost.odtrack\endcsname{22.2}
\expandafter\def\csname BAval@cost.ltmu\endcsname{31.8}
\expandafter\def\csname BAval@cost.keeptrack\endcsname{29.1}
\expandafter\def\csname BAval@cost.advat\endcsname{18.6}
\expandafter\def\csname BAval@cost.joint\endcsname{38.1}
\expandafter\def\csname BAval@sens.h1\endcsname{78.6}
\expandafter\def\csname BAval@sens.h15\endcsname{80.9}
\expandafter\def\csname BAval@sens.h2\endcsname{82.3}
\expandafter\def\csname BAval@sens.h3\endcsname{81.9}
\expandafter\def\csname BAval@sens.h1.ms\endcsname{1.38}
\expandafter\def\csname BAval@sens.h15.ms\endcsname{1.72}
\expandafter\def\csname BAval@sens.h2.ms\endcsname{2.09}
\expandafter\def\csname BAval@sens.h3.ms\endcsname{2.73}
\expandafter\def\csname BAval@sens.b4\endcsname{79.8}
\expandafter\def\csname BAval@sens.b8\endcsname{82.3}
\expandafter\def\csname BAval@sens.b16\endcsname{82.4}
\expandafter\def\csname BAval@sens.b4.ms\endcsname{1.42}
\expandafter\def\csname BAval@sens.b8.ms\endcsname{2.09}
\expandafter\def\csname BAval@sens.b16.ms\endcsname{3.61}
\expandafter\def\csname BAval@sens.d2\endcsname{79.9}
\expandafter\def\csname BAval@sens.d3\endcsname{82.3}
\expandafter\def\csname BAval@sens.d4\endcsname{82.4}
\expandafter\def\csname BAval@sens.d2.ms\endcsname{1.26}
\expandafter\def\csname BAval@sens.d3.ms\endcsname{2.09}
\expandafter\def\csname BAval@sens.d4.ms\endcsname{3.84}
\expandafter\def\csname BAval@t27.r01.correct.s\endcsname{7.40}
\expandafter\def\csname BAval@t27.r01.wrong.s\endcsname{0.21}
\expandafter\def\csname BAval@t27.r01.sid\endcsname{82.2}
\expandafter\def\csname BAval@t27.r01.wrong\endcsname{2.4}
\expandafter\def\csname BAval@t27.r02.correct.s\endcsname{7.07}
\expandafter\def\csname BAval@t27.r02.wrong.s\endcsname{0.35}
\expandafter\def\csname BAval@t27.r02.sid\endcsname{78.5}
\expandafter\def\csname BAval@t27.r02.wrong\endcsname{3.9}
\expandafter\def\csname BAval@t10.r01.separable\endcsname{77.6}
\expandafter\def\csname BAval@t10.r01.temporal.q\endcsname{68.7}
\expandafter\def\csname BAval@sens.h.drop\endcsname{3.6}
\expandafter\def\csname BAval@sens.search.gain\endcsname{0.1}
