# Supplementary material for: BindAdapt: Joint Camera-Computation Scheduling for Persistent Target Identity in PTZ Tracking
Source: arXiv:2611.38995 source file (2026-11-28)
Supplement: Supplementary file 4 [file supp_numbers_v41.tex]

\expandafter\def\csname BAval@svc.retrain.sid\endcsname{81.6}
\expandafter\def\csname BAval@delta.svc.gap\endcsname{3.5}
