# Supplementary material for: BindAdapt: Joint Camera-Computation Scheduling for Persistent Target Identity in PTZ Tracking
Source: arXiv:2611.38995 source file (2026-11-28)
Supplement: Supplementary file 5 [file supp_unsure_flags.tex]

\expandafter\def\csname BAflag@int.joint.recovery\endcsname{}
\expandafter\def\csname BAflag@int.joint.t5\endcsname{}
\expandafter\def\csname BAflag@int.oracle.recovery\endcsname{}
\expandafter\def\csname BAflag@int.oracle.t5\endcsname{}
\expandafter\def\csname BAflag@int.oracle.wrong\endcsname{}
\expandafter\def\csname BAflag@t01.r01.recovery\endcsname{}
\expandafter\def\csname BAflag@t01.r01.sid\endcsname{}
\expandafter\def\csname BAflag@t01.r01.t5\endcsname{}
\expandafter\def\csname BAflag@t01.r01.wrong\endcsname{}
\expandafter\def\csname BAflag@t01.r02.recovery\endcsname{}
\expandafter\def\csname BAflag@t01.r02.sid\endcsname{}
\expandafter\def\csname BAflag@t01.r02.t5\endcsname{}
\expandafter\def\csname BAflag@t01.r02.wrong\endcsname{}
\expandafter\def\csname BAflag@t01.r03.recovery\endcsname{}
\expandafter\def\csname BAflag@t01.r03.sid\endcsname{}
\expandafter\def\csname BAflag@t01.r03.t5\endcsname{}
\expandafter\def\csname BAflag@t01.r03.wrong\endcsname{}
\expandafter\def\csname BAflag@t01.r04.recovery\endcsname{}
\expandafter\def\csname BAflag@t01.r04.sid\endcsname{}
\expandafter\def\csname BAflag@t01.r04.t5\endcsname{}
\expandafter\def\csname BAflag@t01.r04.wrong\endcsname{}
\expandafter\def\csname BAflag@t01.r05.recovery\endcsname{}
\expandafter\def\csname BAflag@t01.r05.sid\endcsname{}
\expandafter\def\csname BAflag@t01.r05.t5\endcsname{}
\expandafter\def\csname BAflag@t01.r05.wrong\endcsname{}
\expandafter\def\csname BAflag@t01.r07.recovery\endcsname{}
\expandafter\def\csname BAflag@t01.r07.t5\endcsname{}
\expandafter\def\csname BAflag@t01.r09.recovery\endcsname{}
\expandafter\def\csname BAflag@t01.r09.t5\endcsname{}
\expandafter\def\csname BAflag@t01.r09.wrong\endcsname{}
\expandafter\def\csname BAflag@t02.r01.long\endcsname{}
\expandafter\def\csname BAflag@t02.r01.short\endcsname{}
\expandafter\def\csname BAflag@t02.r01.similar\endcsname{}
\expandafter\def\csname BAflag@t02.r02.long\endcsname{}
\expandafter\def\csname BAflag@t02.r02.short\endcsname{}
\expandafter\def\csname BAflag@t02.r02.similar\endcsname{}
\expandafter\def\csname BAflag@t02.r03.long\endcsname{}
\expandafter\def\csname BAflag@t02.r03.short\endcsname{}
\expandafter\def\csname BAflag@t02.r03.similar\endcsname{}
\expandafter\def\csname BAflag@t02.r04.long\endcsname{}
\expandafter\def\csname BAflag@t02.r04.short\endcsname{}
\expandafter\def\csname BAflag@t02.r04.similar\endcsname{}
\expandafter\def\csname BAflag@t02.r06.long\endcsname{}
\expandafter\def\csname BAflag@t02.r06.short\endcsname{}
\expandafter\def\csname BAflag@t02.r06.similar\endcsname{}
