# Supplementary material for: BindAdapt: Joint Camera-Computation Scheduling for Persistent Target Identity in PTZ Tracking
Source: arXiv:2611.38995 source file (2026-11-28)
Supplement: Supplementary file 7 [file supper.tex]

\rowcolor{BAours}BindAdapt online & \BAval{t08.r01.sid}\\
Plus exact response & \BAval{t08.r02.sid}\\
Plus perfect acquired-frame identity & \BAval{t08.r03.sid}\\
Plus finite-action future outcomes & \BAval{t08.r04.sid}\\
Plus zero service delay & \BAval{t08.r05.sid}\\
Plus full source visibility & \BAval{t08.r06.sid}\\
